# Supplementary material for: Coulomb matrix elements in multi-orbital Hubbard models
Source: arXiv:1610.04035 source file (2017-01-15)
Supplement: Supplementary file 1 [file suppl_new.pdf]

# Coulomb matrix elements in multi-orbital Hubbard models

## Supplementary material

Jörg Bünemann and Florian Gebhard

### Contents

|          |                                                              |           |
|----------|--------------------------------------------------------------|-----------|
| <b>1</b> | <b>Spherical approximation</b>                               | <b>2</b>  |
| 1.1      | $d$ -orbitals . . . . .                                      | 2         |
| 1.2      | $f$ -orbitals, cubic basis . . . . .                         | 4         |
| 1.3      | $f$ -orbitals, axial basis . . . . .                         | 8         |
| <b>2</b> | <b>First-order correction to the spherical approximation</b> | <b>12</b> |
| 2.1      | $d$ -orbitals, groups $O_h$ , $O$ , $T_d$ . . . . .          | 12        |
| 2.2      | $d$ -orbitals, group $T_h$ . . . . .                         | 14        |
| 2.3      | $d$ -orbitals, group $D_{6h}$ . . . . .                      | 15        |
| 2.4      | $d$ -orbitals, group $D_{4h}$ . . . . .                      | 16        |
| 2.5      | $f$ -orbitals, groups $O_h$ , $O$ , $T_d$ . . . . .          | 17        |
| 2.6      | $f$ -orbitals, group $T_h$ . . . . .                         | 23        |
| 2.7      | $f$ -orbitals, group $D_{6h}$ . . . . .                      | 29        |
| 2.8      | $f$ -orbitals, group $D_{4h}$ . . . . .                      | 37        |

# 1 Spherical approximation

## 1.1 *d*-orbitals

Independent parameters:

$$U(v), U(v, u), U(v, \zeta).$$

Dependent parameters:

$$U(u) = U(v) ,$$

$$U(\zeta) = U(v) ,$$

$$U(\eta) = U(v) ,$$

$$U(\xi) = U(v) ,$$

$$U(u, \zeta) = U(v, u) ,$$

$$U(v, \eta) = \frac{3}{4}U(v, u) + \frac{1}{4}U(v, \zeta) ,$$

$$U(v, \xi) = \frac{3}{4}U(v, u) + \frac{1}{4}U(v, \zeta) ,$$

$$U(u, \eta) = \frac{1}{4}U(v, u) + \frac{3}{4}U(v, \zeta) ,$$

$$U(u, \xi) = \frac{1}{4}U(v, u) + \frac{3}{4}U(v, \zeta) ,$$

$$U(\zeta, \eta) = \frac{3}{4}U(v, u) + \frac{1}{4}U(v, \zeta) ,$$

$$U(\zeta, \xi) = \frac{3}{4}U(v, u) + \frac{1}{4}U(v, \zeta) ,$$

$$U(\eta, \xi) = \frac{3}{4}U(v, u) + \frac{1}{4}U(v, \zeta) ,$$

$$J(v, u) = \frac{1}{2}U(v) - \frac{1}{2}U(v, u) ,$$

$$J(v, \zeta) = \frac{1}{2}U(v) - \frac{1}{2}U(v, \zeta) ,$$

$$J(v, \eta) = \frac{1}{2}U(v) - \frac{3}{8}U(v, u) - \frac{1}{8}U(v, \zeta) ,$$

$$J(u, \zeta) = \frac{1}{2}U(v) - \frac{1}{2}U(v, u) ,$$

$$J(v, \xi) = \frac{1}{2}U(v) - \frac{3}{8}U(v, u) - \frac{1}{8}U(v, \zeta) ,$$

$$J(u, \eta) = \frac{1}{2}U(v) - \frac{1}{8}U(v, u) - \frac{3}{8}U(v, \zeta) ,$$

$$J(u, \xi) = \frac{1}{2}U(v) - \frac{1}{8}U(v, u) - \frac{3}{8}U(v, \zeta) ,$$

$$J(\zeta, \eta) = \frac{1}{2}U(v) - \frac{3}{8}U(v, u) - \frac{1}{8}U(v, \zeta) ,$$

$$J(\zeta, \xi) = \frac{1}{2}U(v) - \frac{3}{8}U(v, u) - \frac{1}{8}U(v, \zeta) ,$$

$$J(\eta, \xi) = \frac{1}{2}U(v) - \frac{3}{8}U(v, u) - \frac{1}{8}U(v, \zeta) ,$$

$$T(\eta; v, u) = \frac{\sqrt{3}}{4}U(v, u) - \frac{\sqrt{3}}{4}U(v, \zeta) ,$$

$$T(\xi; v, u) = -\frac{\sqrt{3}}{4}U(v, u) + \frac{\sqrt{3}}{4}U(v, \zeta) ,$$

$$A(\eta; v, u) = -\frac{\sqrt{3}}{8}U(v, u) + \frac{\sqrt{3}}{8}U(v, \zeta) ,$$

$$\begin{aligned}
A(\xi; v, u) &= \frac{\sqrt{3}}{8}U(v, u) - \frac{\sqrt{3}}{8}U(v, \zeta) , \\
S(v, \zeta; \xi, \eta) &= -\frac{3}{8}U(v, u) + \frac{3}{8}U(v, \zeta) , \\
S(v, \zeta; \eta, \xi) &= \frac{3}{8}U(v, u) - \frac{3}{8}U(v, \zeta) , \\
S(u, \zeta; \xi, \eta) &= -\frac{\sqrt{3}}{8}U(v, u) + \frac{\sqrt{3}}{8}U(v, \zeta) , \\
S(u, \eta; \xi, \zeta) &= \frac{\sqrt{3}}{4}U(v, u) - \frac{\sqrt{3}}{4}U(v, \zeta) , \\
S(u, \zeta; \eta, \xi) &= -\frac{\sqrt{3}}{8}U(v, u) + \frac{\sqrt{3}}{8}U(v, \zeta) .
\end{aligned}$$

## 1.2 $f$ -orbitals, cubic basis

Independent parameters:

$$U(a), U(x), U(a, x), U(x, y).$$

Dependent parameters:

$$U(y) = U(x) ,$$

$$U(z) = U(x) ,$$

$$U(\alpha) = U(a) ,$$

$$U(\beta) = U(a) ,$$

$$U(\gamma) = U(a) ,$$

$$U(a, y) = U(a, x) ,$$

$$U(a, z) = U(a, x) ,$$

$$U(x, z) = U(x, y) ,$$

$$U(a, \alpha) = -\frac{8}{9}U(a) + \frac{8}{9}U(x) - \frac{7}{9}U(a, x) + \frac{16}{9}U(x, y) ,$$

$$U(x, \alpha) = U(a, x) ,$$

$$U(a, \beta) = -\frac{8}{9}U(a) + \frac{8}{9}U(x) - \frac{7}{9}U(a, x) + \frac{16}{9}U(x, y) ,$$

$$U(y, z) = U(x, y) ,$$

$$U(a, \gamma) = -\frac{8}{9}U(a) + \frac{8}{9}U(x) - \frac{7}{9}U(a, x) + \frac{16}{9}U(x, y) ,$$

$$U(x, \beta) = -\frac{5}{6}U(a) + \frac{5}{6}U(x) - \frac{2}{3}U(a, x) + \frac{5}{3}U(x, y) ,$$

$$U(y, \alpha) = -\frac{5}{6}U(a) + \frac{5}{6}U(x) - \frac{2}{3}U(a, x) + \frac{5}{3}U(x, y) ,$$

$$U(z, \alpha) = -\frac{5}{6}U(a) + \frac{5}{6}U(x) - \frac{2}{3}U(a, x) + \frac{5}{3}U(x, y) ,$$

$$U(x, \gamma) = -\frac{5}{6}U(a) + \frac{5}{6}U(x) - \frac{2}{3}U(a, x) + \frac{5}{3}U(x, y) ,$$

$$U(y, \beta) = U(a, x) ,$$

$$U(z, \beta) = -\frac{5}{6}U(a) + \frac{5}{6}U(x) - \frac{2}{3}U(a, x) + \frac{5}{3}U(x, y) ,$$

$$U(y, \gamma) = -\frac{5}{6}U(a) + \frac{5}{6}U(x) - \frac{2}{3}U(a, x) + \frac{5}{3}U(x, y) ,$$

$$U(z, \gamma) = U(a, x) ,$$

$$U(\alpha, \beta) = -\frac{1}{18}U(a) + \frac{1}{18}U(x) + \frac{8}{9}U(a, x) + \frac{2}{18}U(x, y) ,$$

$$U(\alpha, \gamma) = -\frac{1}{18}U(a) + \frac{1}{18}U(x) + \frac{8}{9}U(a, x) + \frac{2}{18}U(x, y) ,$$

$$U(\beta, \gamma) = -\frac{1}{18}U(a) + \frac{1}{18}U(x) + \frac{8}{9}U(a, x) + \frac{2}{18}U(x, y) ,$$

$$J(a, x) = -\frac{3}{4}U(a) + \frac{5}{4}U(x) - \frac{1}{2}U(a, x) ,$$

$$J(a, y) = -\frac{3}{4}U(a) + \frac{5}{4}U(x) - \frac{1}{2}U(a, x) ,$$

$$J(a, z) = -\frac{3}{4}U(a) + \frac{5}{4}U(x) - \frac{1}{2}U(a, x) ,$$

$$J(x, y) = \frac{45}{64}U(a) - \frac{13}{64}U(x) - \frac{1}{2}U(x, y) ,$$

$$J(x, z) = \frac{45}{64}U(a) - \frac{13}{64}U(x) - \frac{1}{2}U(x, y) ,$$

$$J(a, \alpha) = \frac{17}{18}U(a) - \frac{4}{9}U(x) + \frac{7}{18}U(a, x) - \frac{8}{9}U(x, y) ,$$

$$\begin{aligned}
J(a, \beta) &= \frac{17}{18}U(a) - \frac{4}{9}U(x) + \frac{7}{18}U(a, x) - \frac{8}{9}U(x, y) , \\
J(x, \alpha) &= -\frac{3}{4}U(a) + \frac{5}{4}U(x) - \frac{1}{2}U(a, x) , \\
J(y, z) &= \frac{45}{64}U(a) - \frac{13}{64}U(x) - \frac{1}{2}U(x, y) , \\
J(y, \alpha) &= \frac{161}{192}U(a) - \frac{65}{192}U(x) + \frac{1}{3}U(a, x) - \frac{5}{6}U(x, y) , \\
J(x, \beta) &= \frac{161}{192}U(a) - \frac{65}{192}U(x) + \frac{1}{3}U(a, x) - \frac{5}{6}U(x, y) , \\
J(a, \gamma) &= \frac{17}{18}U(a) - \frac{4}{9}U(x) + \frac{7}{18}U(a, x) - \frac{8}{9}U(x, y) , \\
J(y, \beta) &= -\frac{3}{4}U(a) + \frac{5}{4}U(x) - \frac{1}{2}U(a, x) , \\
J(x, \gamma) &= \frac{161}{192}U(a) - \frac{65}{192}U(x) + \frac{1}{3}U(a, x) - \frac{5}{6}U(x, y) , \\
J(z, \alpha) &= \frac{161}{192}U(a) - \frac{65}{192}U(x) + \frac{1}{3}U(a, x) - \frac{5}{6}U(x, y) , \\
J(z, \beta) &= \frac{161}{192}U(a) - \frac{65}{192}U(x) + \frac{1}{3}U(a, x) - \frac{5}{6}U(x, y) , \\
J(y, \gamma) &= \frac{161}{192}U(a) - \frac{65}{192}U(x) + \frac{1}{3}U(a, x) - \frac{5}{6}U(x, y) , \\
J(\alpha, \beta) &= -\frac{371}{576}U(a) + \frac{659}{576}U(x) - \frac{4}{9}U(a, x) - \frac{1}{18}U(x, y) , \\
J(z, \gamma) &= -\frac{3}{4}U(a) + \frac{5}{4}U(x) - \frac{1}{2}U(a, x) , \\
J(\alpha, \gamma) &= -\frac{371}{576}U(a) + \frac{659}{576}U(x) - \frac{4}{9}U(a, x) - \frac{1}{18}U(x, y) , \\
J(\beta, \gamma) &= -\frac{371}{576}U(a) + \frac{659}{576}U(x) - \frac{4}{9}U(a, x) - \frac{1}{18}U(x, y) , \\
T(x; y, \beta) &= \frac{5}{4}\sqrt{\frac{5}{3}}U(a) - \frac{5}{4}\sqrt{\frac{5}{3}}U(x) + \sqrt{\frac{5}{3}}U(a, x) - \sqrt{\frac{5}{3}}U(x, y) , \\
T(y; x, \alpha) &= \frac{5}{4}\sqrt{\frac{5}{3}}U(a) - \frac{5}{4}\sqrt{\frac{5}{3}}U(x) + \sqrt{\frac{5}{3}}U(a, x) - \sqrt{\frac{5}{3}}U(x, y) , \\
T(z; x, \alpha) &= -\frac{5}{4}\sqrt{\frac{5}{3}}U(a) + \frac{5}{4}\sqrt{\frac{5}{3}}U(x) - \sqrt{\frac{5}{3}}U(a, x) + \sqrt{\frac{5}{3}}U(x, y) , \\
T(x; z, \gamma) &= \frac{5}{4}\sqrt{\frac{5}{3}}U(a) - \frac{5}{4}\sqrt{\frac{5}{3}}U(x) + \sqrt{\frac{5}{3}}U(a, x) - \sqrt{\frac{5}{3}}U(x, y) , \\
T(z; y, \beta) &= -\frac{5}{4}\sqrt{\frac{5}{3}}U(a) + \frac{5}{4}\sqrt{\frac{5}{3}}U(x) - \sqrt{\frac{5}{3}}U(a, x) + \sqrt{\frac{5}{3}}U(x, y) , \\
T(y; z, \gamma) &= -\frac{5}{4}\sqrt{\frac{5}{3}}U(a) + \frac{5}{4}\sqrt{\frac{5}{3}}U(x) - \sqrt{\frac{5}{3}}U(a, x) + \sqrt{\frac{5}{3}}U(x, y) , \\
T(\alpha; y, \beta) &= \frac{1}{6}\sqrt{\frac{5}{3}}U(a) - \frac{1}{6}\sqrt{\frac{5}{3}}U(x) + \frac{1}{3}\sqrt{\frac{5}{3}}U(a, x) - \frac{1}{3}\sqrt{\frac{5}{3}}U(x, y) , \\
T(\beta; x, \alpha) &= \frac{1}{6}\sqrt{\frac{5}{3}}U(a) - \frac{1}{6}\sqrt{\frac{5}{3}}U(x) + \frac{1}{3}\sqrt{\frac{5}{3}}U(a, x) - \frac{1}{3}\sqrt{\frac{5}{3}}U(x, y) , \\
T(\alpha; z, \gamma) &= \frac{1}{6}\sqrt{\frac{5}{3}}U(a) - \frac{1}{6}\sqrt{\frac{5}{3}}U(x) + \frac{1}{3}\sqrt{\frac{5}{3}}U(a, x) - \frac{1}{3}\sqrt{\frac{5}{3}}U(x, y) , \\
T(\gamma; x, \alpha) &= -\frac{1}{6}\sqrt{\frac{5}{3}}U(a) + \frac{1}{6}\sqrt{\frac{5}{3}}U(x) - \frac{1}{3}\sqrt{\frac{5}{3}}U(a, x) + \frac{1}{3}\sqrt{\frac{5}{3}}U(x, y) , \\
T(\beta; z, \gamma) &= -\frac{1}{6}\sqrt{\frac{5}{3}}U(a) + \frac{1}{6}\sqrt{\frac{5}{3}}U(x) - \frac{1}{3}\sqrt{\frac{5}{3}}U(a, x) + \frac{1}{3}\sqrt{\frac{5}{3}}U(x, y) ,
\end{aligned}$$

$$\begin{aligned}
T(\gamma; y, \beta) &= -\frac{1}{6}\sqrt{\frac{5}{3}}U(a) + \frac{1}{6}\sqrt{\frac{5}{3}}U(x) - \frac{1}{3}\sqrt{\frac{5}{3}}U(a, x) + \frac{1}{3}\sqrt{\frac{5}{3}}U(x, y) , \\
A(y; x, \alpha) &= -\frac{13}{64}\sqrt{\frac{5}{3}}U(a) + \frac{13}{64}\sqrt{\frac{5}{3}}U(x) - \frac{1}{2}\sqrt{\frac{5}{3}}U(a, x) + \frac{1}{2}\sqrt{\frac{5}{3}}U(x, y) , \\
A(x; x, \beta) &= -\frac{13}{64}\sqrt{\frac{5}{3}}U(a) + \frac{13}{64}\sqrt{\frac{5}{3}}U(x) - \frac{1}{2}\sqrt{\frac{5}{3}}U(a, x) + \frac{1}{2}\sqrt{\frac{5}{3}}U(x, y) , \\
A(z; x, \alpha) &= \frac{13}{64}\sqrt{\frac{5}{3}}U(a) - \frac{13}{64}\sqrt{\frac{5}{3}}U(x) + \frac{1}{2}\sqrt{\frac{5}{3}}U(a, x) - \frac{1}{2}\sqrt{\frac{5}{3}}U(x, y) , \\
A(x; x, \gamma) &= -\frac{13}{64}\sqrt{\frac{5}{3}}U(a) + \frac{13}{64}\sqrt{\frac{5}{3}}U(x) - \frac{1}{2}\sqrt{\frac{5}{3}}U(a, x) + \frac{1}{2}\sqrt{\frac{5}{3}}U(x, y) , \\
A(y; y, \gamma) &= \frac{13}{64}\sqrt{\frac{5}{3}}U(a) - \frac{13}{64}\sqrt{\frac{5}{3}}U(x) + \frac{1}{2}\sqrt{\frac{5}{3}}U(a, x) - \frac{1}{2}\sqrt{\frac{5}{3}}U(x, y) , \\
A(z; y, \beta) &= \frac{13}{64}\sqrt{\frac{5}{3}}U(a) - \frac{13}{64}\sqrt{\frac{5}{3}}U(x) + \frac{1}{2}\sqrt{\frac{5}{3}}U(a, x) - \frac{1}{2}\sqrt{\frac{5}{3}}U(x, y) , \\
A(\beta; x, \alpha) &= -\frac{61}{192}\sqrt{\frac{5}{3}}U(a) + \frac{61}{192}\sqrt{\frac{5}{3}}U(x) - \frac{1}{6}\sqrt{\frac{5}{3}}U(a, x) + \frac{1}{6}\sqrt{\frac{5}{3}}U(x, y) , \\
A(\alpha; y, \beta) &= -\frac{61}{192}\sqrt{\frac{5}{3}}U(a) + \frac{61}{192}\sqrt{\frac{5}{3}}U(x) - \frac{1}{6}\sqrt{\frac{5}{3}}U(a, x) + \frac{1}{6}\sqrt{\frac{5}{3}}U(x, y) , \\
A(\gamma; x, \alpha) &= \frac{61}{192}\sqrt{\frac{5}{3}}U(a) - \frac{61}{192}\sqrt{\frac{5}{3}}U(x) + \frac{1}{6}\sqrt{\frac{5}{3}}U(a, x) - \frac{1}{6}\sqrt{\frac{5}{3}}U(x, y) , \\
A(\alpha; z, \gamma) &= -\frac{61}{192}\sqrt{\frac{5}{3}}U(a) + \frac{61}{192}\sqrt{\frac{5}{3}}U(x) - \frac{1}{6}\sqrt{\frac{5}{3}}U(a, x) + \frac{1}{6}\sqrt{\frac{5}{3}}U(x, y) , \\
A(\beta; z, \gamma) &= \frac{61}{192}\sqrt{\frac{5}{3}}U(a) - \frac{61}{192}\sqrt{\frac{5}{3}}U(x) + \frac{1}{6}\sqrt{\frac{5}{3}}U(a, x) - \frac{1}{6}\sqrt{\frac{5}{3}}U(x, y) , \\
A(\gamma; y, \beta) &= \frac{61}{192}\sqrt{\frac{5}{3}}U(a) - \frac{61}{192}\sqrt{\frac{5}{3}}U(x) + \frac{1}{6}\sqrt{\frac{5}{3}}U(a, x) - \frac{1}{6}\sqrt{\frac{5}{3}}U(x, y) , \\
S(a, x; z, y) &= -\frac{1}{9}\sqrt{\frac{5}{3}}U(a) + \frac{1}{9}\sqrt{\frac{5}{3}}U(x) , \\
S(a, y; z, x) &= -\frac{1}{9}\sqrt{\frac{5}{3}}U(a) + \frac{1}{9}\sqrt{\frac{5}{3}}U(x) , \\
S(a, x; y, z) &= -\frac{1}{9}\sqrt{\frac{5}{3}}U(a) + \frac{1}{9}\sqrt{\frac{5}{3}}U(x) , \\
S(a, x; \gamma, y) &= \frac{31}{48}U(a) - \frac{31}{48}U(x) + \frac{2}{3}U(a, x) - \frac{2}{3}U(x, y) , \\
S(a, z; \alpha, y) &= -\frac{31}{48}U(a) + \frac{31}{48}U(x) - \frac{2}{3}U(a, x) + \frac{2}{3}U(x, y) , \\
S(a, z; \beta, x) &= -\frac{31}{48}U(a) + \frac{31}{48}U(x) - \frac{2}{3}U(a, x) + \frac{2}{3}U(x, y) , \\
S(a, y; \alpha, z) &= \frac{31}{48}U(a) - \frac{31}{48}U(x) + \frac{2}{3}U(a, x) - \frac{2}{3}U(x, y) , \\
S(a, y; \gamma, x) &= -\frac{31}{48}U(a) + \frac{31}{48}U(x) - \frac{2}{3}U(a, x) + \frac{2}{3}U(x, y) , \\
S(a, x; \beta, z) &= \frac{31}{48}U(a) - \frac{31}{48}U(x) + \frac{2}{3}U(a, x) - \frac{2}{3}U(x, y) , \\
S(a, \beta; \gamma, x) &= \frac{77}{48}\sqrt{\frac{5}{3}}U(a) - \frac{77}{48}\sqrt{\frac{5}{3}}U(x) + \frac{4}{27}\sqrt{5}U(a, x) - \frac{4}{27}\sqrt{5}U(x, y) , \\
S(x, \alpha; \beta, y) &= \frac{4096}{6250}U(a) - \frac{4096}{6250}U(x) + \frac{5}{6}U(a, x) - \frac{5}{6}U(x, y) , \\
S(x, y; \alpha, \beta) &= \frac{1}{192}U(a) - \frac{1}{192}U(x) + \frac{1}{6}U(a, x) - \frac{1}{6}U(x, y) ,
\end{aligned}$$

$$\begin{aligned}
S(a, z; \beta, \alpha) &= -\frac{1}{3}\sqrt{\frac{5}{3}}U(a) + \frac{1}{3}\sqrt{\frac{5}{3}}U(x) - \frac{2}{3}\sqrt{\frac{5}{3}}U(a, x) + \frac{2}{3}\sqrt{\frac{5}{3}}U(x, y) , \\
S(x, y; \beta, \alpha) &= -\frac{9}{8}U(a) + \frac{9}{8}U(x) - U(a, x) + U(x, y) , \\
S(a, \alpha; \beta, z) &= \frac{77}{48}\sqrt{\frac{5}{3}}U(a) - \frac{77}{48}\sqrt{\frac{5}{3}}U(x) + \frac{4}{27}\sqrt{5}U(a, x) - \frac{4}{27}\sqrt{5}U(x, y) , \\
S(a, \alpha; \gamma, y) &= -\frac{77}{48}\sqrt{\frac{5}{3}}U(a) + \frac{77}{48}\sqrt{\frac{5}{3}}U(x) - \frac{4}{27}\sqrt{5}U(a, x) + \frac{4}{27}\sqrt{5}U(x, y) , \\
S(a, y; \alpha, \gamma) &= \frac{1}{3}\sqrt{\frac{5}{3}}U(a) - \frac{1}{3}\sqrt{\frac{5}{3}}U(x) + \frac{2}{3}\sqrt{\frac{5}{3}}U(a, x) - \frac{2}{3}\sqrt{\frac{5}{3}}U(x, y) , \\
S(a, x; \beta, \gamma) &= -\frac{1}{3}\sqrt{\frac{5}{3}}U(a) + \frac{1}{3}\sqrt{\frac{5}{3}}U(x) - \frac{2}{3}\sqrt{\frac{5}{3}}U(a, x) + \frac{2}{3}\sqrt{\frac{5}{3}}U(x, y) , \\
S(a, x; \gamma, \beta) &= -\frac{1}{3}\sqrt{\frac{5}{3}}U(a) + \frac{1}{3}\sqrt{\frac{5}{3}}U(x) - \frac{2}{3}\sqrt{\frac{5}{3}}U(a, x) + \frac{2}{3}\sqrt{\frac{5}{3}}U(x, y) , \\
S(a, z; \alpha, \beta) &= -\frac{1}{3}\sqrt{\frac{5}{3}}U(a) + \frac{1}{3}\sqrt{\frac{5}{3}}U(x) - \frac{2}{3}\sqrt{\frac{5}{3}}U(a, x) + \frac{2}{3}\sqrt{\frac{5}{3}}U(x, y) , \\
S(a, y; \gamma, \alpha) &= \frac{1}{3}\sqrt{\frac{5}{3}}U(a) - \frac{1}{3}\sqrt{\frac{5}{3}}U(x) + \frac{2}{3}\sqrt{\frac{5}{3}}U(a, x) - \frac{2}{3}\sqrt{\frac{5}{3}}U(x, y) , \\
S(x, z; \alpha, \gamma) &= -\frac{1}{192}U(a) + \frac{1}{192}U(x) - \frac{1}{6}U(a, x) + \frac{1}{6}U(x, y) , \\
S(x, \alpha; \gamma, z) &= -\frac{4096}{6250}U(a) + \frac{4096}{6250}U(x) - \frac{5}{6}U(a, x) + \frac{5}{6}U(x, y) , \\
S(x, z; \gamma, \alpha) &= \frac{9}{8}U(a) - \frac{9}{8}U(x) + U(a, x) - U(x, y) , \\
S(y, \beta; \gamma, z) &= \frac{4096}{6250}U(a) - \frac{4096}{6250}U(x) + \frac{5}{6}U(a, x) - \frac{5}{6}U(x, y) , \\
S(y, z; \gamma, \beta) &= -\frac{9}{8}U(a) + \frac{9}{8}U(x) - U(a, x) + U(x, y) , \\
S(y, z; \beta, \gamma) &= \frac{1}{192}U(a) - \frac{1}{192}U(x) + \frac{1}{6}U(a, x) - \frac{1}{6}U(x, y) .
\end{aligned}$$

### 1.3 $f$ -orbitals, axial basis

Independent parameters:

$$U(a), U(x'), U(a, x'), U(x', y').$$

Dependent parameters:

$$U(y') = U(x') ,$$

$$U(z) = U(x') ,$$

$$U(\alpha') = U(a) ,$$

$$U(\beta') = U(a) ,$$

$$U(\gamma) = U(a) ,$$

$$U(a, y') = U(a, x') ,$$

$$U(a, z) = U(a, x') ,$$

$$U(x', z) = U(x', y') ,$$

$$U(a, \alpha') = -\frac{8}{9}U(a) + \frac{8}{9}U(x') - \frac{7}{9}U(a, x') + \frac{16}{9}U(x', y') ,$$

$$U(x', \alpha') = U(a, x') ,$$

$$U(a, \beta') = -\frac{8}{9}U(a) + \frac{8}{9}U(x') - \frac{7}{9}U(a, x') + \frac{16}{9}U(x', y') ,$$

$$U(y', z) = U(x', y') ,$$

$$U(a, \gamma) = -\frac{8}{9}U(a) + \frac{8}{9}U(x') - \frac{7}{9}U(a, x') + \frac{16}{9}U(x', y') ,$$

$$U(x', \beta') = -\frac{5}{6}U(a) + \frac{5}{6}U(x') - \frac{2}{3}U(a, x') + \frac{5}{3}U(x', y') ,$$

$$U(y', \alpha') = -\frac{5}{6}U(a) + \frac{5}{6}U(x') - \frac{2}{3}U(a, x') + \frac{5}{3}U(x', y') ,$$

$$U(z, \alpha') = -\frac{5}{6}U(a) + \frac{5}{6}U(x') - \frac{2}{3}U(a, x') + \frac{5}{3}U(x', y') ,$$

$$U(x', \gamma) = -\frac{5}{6}U(a) + \frac{5}{6}U(x') - \frac{2}{3}U(a, x') + \frac{5}{3}U(x', y') ,$$

$$U(y', \beta') = U(a, x') ,$$

$$U(z, \beta') = -\frac{5}{6}U(a) + \frac{5}{6}U(x') - \frac{2}{3}U(a, x') + \frac{5}{3}U(x', y') ,$$

$$U(y', \gamma) = -\frac{5}{6}U(a) + \frac{5}{6}U(x') - \frac{2}{3}U(a, x') + \frac{5}{3}U(x', y') ,$$

$$U(z, \gamma) = U(a, x') ,$$

$$U(\alpha', \beta') = -\frac{1}{18}U(a) + \frac{1}{18}U(x') + \frac{8}{9}U(a, x') + \frac{2}{18}U(x', y') ,$$

$$U(\alpha', \gamma) = -\frac{1}{18}U(a) + \frac{1}{18}U(x') + \frac{8}{9}U(a, x') + \frac{2}{18}U(x', y') ,$$

$$U(\beta', \gamma) = -\frac{1}{18}U(a) + \frac{1}{18}U(x') + \frac{8}{9}U(a, x') + \frac{2}{18}U(x', y') ,$$

$$J(a, x') = -\frac{3}{4}U(a) + \frac{5}{4}U(x') - \frac{1}{2}U(a, x') ,$$

$$J(a, y') = -\frac{3}{4}U(a) + \frac{5}{4}U(x') - \frac{1}{2}U(a, x') ,$$

$$J(a, z) = -\frac{3}{4}U(a) + \frac{5}{4}U(x') - \frac{1}{2}U(a, x') ,$$

$$J(x', y') = \frac{45}{64}U(a) - \frac{13}{64}U(x') - \frac{1}{2}U(x', y') ,$$

$$J(x', z) = \frac{45}{64}U(a) - \frac{13}{64}U(x') - \frac{1}{2}U(x', y') ,$$

$$J(a, \alpha') = \frac{17}{18}U(a) - \frac{4}{9}U(x') + \frac{7}{18}U(a, x') - \frac{8}{9}U(x', y') ,$$



$$\begin{aligned}
J(a, \beta') &= \frac{17}{18}U(a) - \frac{4}{9}U(x') + \frac{7}{18}U(a, x') - \frac{8}{9}U(x', y') , \\
J(x', \alpha') &= -\frac{3}{4}U(a) + \frac{5}{4}U(x') - \frac{1}{2}U(a, x') , \\
J(y', z) &= \frac{45}{64}U(a) - \frac{13}{64}U(x') - \frac{1}{2}U(x', y') , \\
J(y', \alpha') &= \frac{161}{192}U(a) - \frac{65}{192}U(x') + \frac{1}{3}U(a, x') - \frac{5}{6}U(x', y') , \\
J(x', \beta') &= \frac{161}{192}U(a) - \frac{65}{192}U(x') + \frac{1}{3}U(a, x') - \frac{5}{6}U(x', y') , \\
J(a, \gamma) &= \frac{17}{18}U(a) - \frac{4}{9}U(x') + \frac{7}{18}U(a, x') - \frac{8}{9}U(x', y') , \\
J(y', \beta') &= -\frac{3}{4}U(a) + \frac{5}{4}U(x') - \frac{1}{2}U(a, x') , \\
J(x', \gamma) &= \frac{161}{192}U(a) - \frac{65}{192}U(x') + \frac{1}{3}U(a, x') - \frac{5}{6}U(x', y') , \\
J(z, \alpha') &= \frac{161}{192}U(a) - \frac{65}{192}U(x') + \frac{1}{3}U(a, x') - \frac{5}{6}U(x', y') , \\
J(z, \beta') &= \frac{161}{192}U(a) - \frac{65}{192}U(x') + \frac{1}{3}U(a, x') - \frac{5}{6}U(x', y') , \\
J(y', \gamma) &= \frac{161}{192}U(a) - \frac{65}{192}U(x') + \frac{1}{3}U(a, x') - \frac{5}{6}U(x', y') , \\
J(\alpha', \beta') &= -\frac{371}{576}U(a) + \frac{659}{576}U(x') - \frac{4}{9}U(a, x') - \frac{1}{18}U(x', y') , \\
J(z, \gamma) &= -\frac{3}{4}U(a) + \frac{5}{4}U(x') - \frac{1}{2}U(a, x') , \\
J(\alpha', \gamma) &= -\frac{371}{576}U(a) + \frac{659}{576}U(x') - \frac{4}{9}U(a, x') - \frac{1}{18}U(x', y') , \\
J(\beta', \gamma) &= -\frac{371}{576}U(a) + \frac{659}{576}U(x') - \frac{4}{9}U(a, x') - \frac{1}{18}U(x', y') , \\
T(x'; y', \beta') &= \frac{5}{4}\sqrt{\frac{5}{3}}U(a) - \frac{5}{4}\sqrt{\frac{5}{3}}U(x') + \sqrt{\frac{5}{3}}U(a, x') - \sqrt{\frac{5}{3}}U(x', y') , \\
T(y'; x', \alpha') &= \frac{5}{4}\sqrt{\frac{5}{3}}U(a) - \frac{5}{4}\sqrt{\frac{5}{3}}U(x') + \sqrt{\frac{5}{3}}U(a, x') - \sqrt{\frac{5}{3}}U(x', y') , \\
T(z; x', \alpha') &= -\frac{5}{4}\sqrt{\frac{5}{3}}U(a) + \frac{5}{4}\sqrt{\frac{5}{3}}U(x') - \sqrt{\frac{5}{3}}U(a, x') + \sqrt{\frac{5}{3}}U(x', y') , \\
T(x'; z, \gamma) &= \frac{5}{4}\sqrt{\frac{5}{3}}U(a) - \frac{5}{4}\sqrt{\frac{5}{3}}U(x') + \sqrt{\frac{5}{3}}U(a, x') - \sqrt{\frac{5}{3}}U(x', y') , \\
T(z; y', \beta') &= -\frac{5}{4}\sqrt{\frac{5}{3}}U(a) + \frac{5}{4}\sqrt{\frac{5}{3}}U(x') - \sqrt{\frac{5}{3}}U(a, x') + \sqrt{\frac{5}{3}}U(x', y') , \\
T(y'; z, \gamma) &= -\frac{5}{4}\sqrt{\frac{5}{3}}U(a) + \frac{5}{4}\sqrt{\frac{5}{3}}U(x') - \sqrt{\frac{5}{3}}U(a, x') + \sqrt{\frac{5}{3}}U(x', y') , \\
T(\alpha'; y', \beta') &= \frac{1}{6}\sqrt{\frac{5}{3}}U(a) - \frac{1}{6}\sqrt{\frac{5}{3}}U(x') + \frac{1}{3}\sqrt{\frac{5}{3}}U(a, x') - \frac{1}{3}\sqrt{\frac{5}{3}}U(x', y') , \\
T(\beta'; x', \alpha') &= \frac{1}{6}\sqrt{\frac{5}{3}}U(a) - \frac{1}{6}\sqrt{\frac{5}{3}}U(x') + \frac{1}{3}\sqrt{\frac{5}{3}}U(a, x') - \frac{1}{3}\sqrt{\frac{5}{3}}U(x', y') , \\
T(\alpha'; z, \gamma) &= \frac{1}{6}\sqrt{\frac{5}{3}}U(a) - \frac{1}{6}\sqrt{\frac{5}{3}}U(x') + \frac{1}{3}\sqrt{\frac{5}{3}}U(a, x') - \frac{1}{3}\sqrt{\frac{5}{3}}U(x', y') , \\
T(\gamma; x', \alpha') &= -\frac{1}{6}\sqrt{\frac{5}{3}}U(a) + \frac{1}{6}\sqrt{\frac{5}{3}}U(x') - \frac{1}{3}\sqrt{\frac{5}{3}}U(a, x') + \frac{1}{3}\sqrt{\frac{5}{3}}U(x', y') , \\
T(\beta'; z, \gamma) &= -\frac{1}{6}\sqrt{\frac{5}{3}}U(a) + \frac{1}{6}\sqrt{\frac{5}{3}}U(x') - \frac{1}{3}\sqrt{\frac{5}{3}}U(a, x') + \frac{1}{3}\sqrt{\frac{5}{3}}U(x', y') ,
\end{aligned}$$

$$\begin{aligned}
T(\gamma; y', \beta') &= -\frac{1}{6}\sqrt{\frac{5}{3}}U(a) + \frac{1}{6}\sqrt{\frac{5}{3}}U(x') - \frac{1}{3}\sqrt{\frac{5}{3}}U(a, x') + \frac{1}{3}\sqrt{\frac{5}{3}}U(x', y') , \\
A(y'; x', \alpha') &= -\frac{13}{64}\sqrt{\frac{5}{3}}U(a) + \frac{13}{64}\sqrt{\frac{5}{3}}U(x') - \frac{1}{2}\sqrt{\frac{5}{3}}U(a, x') + \frac{1}{2}\sqrt{\frac{5}{3}}U(x', y') , \\
A(x'; x', \beta') &= -\frac{13}{64}\sqrt{\frac{5}{3}}U(a) + \frac{13}{64}\sqrt{\frac{5}{3}}U(x') - \frac{1}{2}\sqrt{\frac{5}{3}}U(a, x') + \frac{1}{2}\sqrt{\frac{5}{3}}U(x', y') , \\
A(z; x', \alpha') &= \frac{13}{64}\sqrt{\frac{5}{3}}U(a) - \frac{13}{64}\sqrt{\frac{5}{3}}U(x') + \frac{1}{2}\sqrt{\frac{5}{3}}U(a, x') - \frac{1}{2}\sqrt{\frac{5}{3}}U(x', y') , \\
A(x'; x', \gamma) &= -\frac{13}{64}\sqrt{\frac{5}{3}}U(a) + \frac{13}{64}\sqrt{\frac{5}{3}}U(x') - \frac{1}{2}\sqrt{\frac{5}{3}}U(a, x') + \frac{1}{2}\sqrt{\frac{5}{3}}U(x', y') , \\
A(y'; y', \gamma) &= \frac{13}{64}\sqrt{\frac{5}{3}}U(a) - \frac{13}{64}\sqrt{\frac{5}{3}}U(x') + \frac{1}{2}\sqrt{\frac{5}{3}}U(a, x') - \frac{1}{2}\sqrt{\frac{5}{3}}U(x', y') , \\
A(z; y', \beta') &= \frac{13}{64}\sqrt{\frac{5}{3}}U(a) - \frac{13}{64}\sqrt{\frac{5}{3}}U(x') + \frac{1}{2}\sqrt{\frac{5}{3}}U(a, x') - \frac{1}{2}\sqrt{\frac{5}{3}}U(x', y') , \\
A(\beta'; x', \alpha') &= -\frac{61}{192}\sqrt{\frac{5}{3}}U(a) + \frac{61}{192}\sqrt{\frac{5}{3}}U(x') - \frac{1}{6}\sqrt{\frac{5}{3}}U(a, x') + \frac{1}{6}\sqrt{\frac{5}{3}}U(x', y') , \\
A(\alpha'; y', \beta') &= -\frac{61}{192}\sqrt{\frac{5}{3}}U(a) + \frac{61}{192}\sqrt{\frac{5}{3}}U(x') - \frac{1}{6}\sqrt{\frac{5}{3}}U(a, x') + \frac{1}{6}\sqrt{\frac{5}{3}}U(x', y') , \\
A(\gamma; x', \alpha') &= \frac{61}{192}\sqrt{\frac{5}{3}}U(a) - \frac{61}{192}\sqrt{\frac{5}{3}}U(x') + \frac{1}{6}\sqrt{\frac{5}{3}}U(a, x') - \frac{1}{6}\sqrt{\frac{5}{3}}U(x', y') , \\
A(\alpha'; z, \gamma) &= -\frac{61}{192}\sqrt{\frac{5}{3}}U(a) + \frac{61}{192}\sqrt{\frac{5}{3}}U(x') - \frac{1}{6}\sqrt{\frac{5}{3}}U(a, x') + \frac{1}{6}\sqrt{\frac{5}{3}}U(x', y') , \\
A(\beta'; z, \gamma) &= \frac{61}{192}\sqrt{\frac{5}{3}}U(a) - \frac{61}{192}\sqrt{\frac{5}{3}}U(x') + \frac{1}{6}\sqrt{\frac{5}{3}}U(a, x') - \frac{1}{6}\sqrt{\frac{5}{3}}U(x', y') , \\
A(\gamma; y', \beta') &= \frac{61}{192}\sqrt{\frac{5}{3}}U(a) - \frac{61}{192}\sqrt{\frac{5}{3}}U(x') + \frac{1}{6}\sqrt{\frac{5}{3}}U(a, x') - \frac{1}{6}\sqrt{\frac{5}{3}}U(x', y') , \\
S(a, x'; z, y') &= -\frac{1}{9}\sqrt{\frac{5}{3}}U(a) + \frac{1}{9}\sqrt{\frac{5}{3}}U(x') , \\
S(a, y'; z, x') &= -\frac{1}{9}\sqrt{\frac{5}{3}}U(a) + \frac{1}{9}\sqrt{\frac{5}{3}}U(x') , \\
S(a, x'; y', z) &= -\frac{1}{9}\sqrt{\frac{5}{3}}U(a) + \frac{1}{9}\sqrt{\frac{5}{3}}U(x') , \\
S(a, x'; \gamma, y') &= \frac{31}{48}U(a) - \frac{31}{48}U(x') + \frac{2}{3}U(a, x') - \frac{2}{3}U(x', y') , \\
S(a, z; \alpha', y') &= -\frac{31}{48}U(a) + \frac{31}{48}U(x') - \frac{2}{3}U(a, x') + \frac{2}{3}U(x', y') , \\
S(a, z; \beta', x') &= -\frac{31}{48}U(a) + \frac{31}{48}U(x') - \frac{2}{3}U(a, x') + \frac{2}{3}U(x', y') , \\
S(a, y'; \alpha', z) &= \frac{31}{48}U(a) - \frac{31}{48}U(x') + \frac{2}{3}U(a, x') - \frac{2}{3}U(x', y') , \\
S(a, y'; \gamma, x') &= -\frac{31}{48}U(a) + \frac{31}{48}U(x') - \frac{2}{3}U(a, x') + \frac{2}{3}U(x', y') , \\
S(a, x'; \beta', z) &= \frac{31}{48}U(a) - \frac{31}{48}U(x') + \frac{2}{3}U(a, x') - \frac{2}{3}U(x', y') , \\
S(a, \beta'; \gamma, x') &= \frac{77}{48}\sqrt{\frac{5}{3}}U(a) - \frac{77}{48}\sqrt{\frac{5}{3}}U(x') + \frac{4}{27}\sqrt{5}U(a, x') - \frac{4}{27}\sqrt{5}U(x', y') , \\
S(x', \alpha'; \beta', y') &= \frac{4096}{6250}U(a) - \frac{4096}{6250}U(x') + \frac{5}{6}U(a, x') - \frac{5}{6}U(x', y') , \\
S(x', y'; \alpha', \beta') &= \frac{1}{192}U(a) - \frac{1}{192}U(x') + \frac{1}{6}U(a, x') - \frac{1}{6}U(x', y') ,
\end{aligned}$$

$$\begin{aligned}
S(a, z; \beta', \alpha') &= -\frac{1}{3}\sqrt{\frac{5}{3}}U(a) + \frac{1}{3}\sqrt{\frac{5}{3}}U(x') - \frac{2}{3}\sqrt{\frac{5}{3}}U(a, x') + \frac{2}{3}\sqrt{\frac{5}{3}}U(x', y') , \\
S(x', y'; \beta', \alpha') &= -\frac{9}{8}U(a) + \frac{9}{8}U(x') - U(a, x') + U(x', y') , \\
S(a, \alpha'; \beta', z) &= \frac{77}{48}\sqrt{\frac{5}{3}}U(a) - \frac{77}{48}\sqrt{\frac{5}{3}}U(x') + \frac{4}{27}\sqrt{5}U(a, x') - \frac{4}{27}\sqrt{5}U(x', y') , \\
S(a, \alpha'; \gamma, y') &= -\frac{77}{48}\sqrt{\frac{5}{3}}U(a) + \frac{77}{48}\sqrt{\frac{5}{3}}U(x') - \frac{4}{27}\sqrt{5}U(a, x') + \frac{4}{27}\sqrt{5}U(x', y') , \\
S(a, y'; \alpha', \gamma) &= \frac{1}{3}\sqrt{\frac{5}{3}}U(a) - \frac{1}{3}\sqrt{\frac{5}{3}}U(x') + \frac{2}{3}\sqrt{\frac{5}{3}}U(a, x') - \frac{2}{3}\sqrt{\frac{5}{3}}U(x', y') , \\
S(a, x'; \beta', \gamma) &= -\frac{1}{3}\sqrt{\frac{5}{3}}U(a) + \frac{1}{3}\sqrt{\frac{5}{3}}U(x') - \frac{2}{3}\sqrt{\frac{5}{3}}U(a, x') + \frac{2}{3}\sqrt{\frac{5}{3}}U(x', y') , \\
S(a, x'; \gamma, \beta') &= -\frac{1}{3}\sqrt{\frac{5}{3}}U(a) + \frac{1}{3}\sqrt{\frac{5}{3}}U(x') - \frac{2}{3}\sqrt{\frac{5}{3}}U(a, x') + \frac{2}{3}\sqrt{\frac{5}{3}}U(x', y') , \\
S(a, z; \alpha', \beta') &= -\frac{1}{3}\sqrt{\frac{5}{3}}U(a) + \frac{1}{3}\sqrt{\frac{5}{3}}U(x') - \frac{2}{3}\sqrt{\frac{5}{3}}U(a, x') + \frac{2}{3}\sqrt{\frac{5}{3}}U(x', y') , \\
S(a, y'; \gamma, \alpha') &= \frac{1}{3}\sqrt{\frac{5}{3}}U(a) - \frac{1}{3}\sqrt{\frac{5}{3}}U(x') + \frac{2}{3}\sqrt{\frac{5}{3}}U(a, x') - \frac{2}{3}\sqrt{\frac{5}{3}}U(x', y') , \\
S(x', z; \alpha', \gamma) &= -\frac{1}{192}U(a) + \frac{1}{192}U(x') - \frac{1}{6}U(a, x') + \frac{1}{6}U(x', y') , \\
S(x', \alpha'; \gamma, z) &= -\frac{4096}{6250}U(a) + \frac{4096}{6250}U(x') - \frac{5}{6}U(a, x') + \frac{5}{6}U(x', y') , \\
S(x', z; \gamma, \alpha') &= \frac{9}{8}U(a) - \frac{9}{8}U(x') + U(a, x') - U(x', y') , \\
S(y', \beta'; \gamma, z) &= \frac{4096}{6250}U(a) - \frac{4096}{6250}U(x') + \frac{5}{6}U(a, x') - \frac{5}{6}U(x', y') , \\
S(y', z; \gamma, \beta') &= -\frac{9}{8}U(a) + \frac{9}{8}U(x') - U(a, x') + U(x', y') , \\
S(y', z; \beta', \gamma) &= \frac{1}{192}U(a) - \frac{1}{192}U(x') + \frac{1}{6}U(a, x') - \frac{1}{6}U(x', y') .
\end{aligned}$$

## 2 First-order correction to the spherical approximation

### 2.1 *d*-orbitals, groups $O_h$ , $O$ , $T_d$

Independent parameter variations:

$$\delta U(\zeta), \delta U(u, \zeta), \delta U(\zeta, \eta).$$

Dependent parameter variations:

$$\begin{aligned} \delta U(\eta) &= \delta U(\zeta) , \\ \delta U(\xi) &= \delta U(\zeta) , \\ \delta U(v, \eta) &= \frac{3}{4} \delta U(u, \zeta) , \\ \delta U(v, \xi) &= \frac{3}{4} \delta U(u, \zeta) , \\ \delta U(u, \eta) &= \frac{1}{4} \delta U(u, \zeta) , \\ \delta U(u, \xi) &= \frac{1}{4} \delta U(u, \zeta) , \\ \delta U(\zeta, \xi) &= \delta U(\zeta, \eta) , \\ \delta U(\eta, \xi) &= \delta U(\zeta, \eta) , \\ \delta J(v, \zeta) &= \frac{1}{4} \delta U(\zeta) , \\ \delta J(v, \eta) &= \frac{1}{4} \delta U(\zeta) - \frac{3}{8} \delta U(u, \zeta) , \\ \delta J(v, \xi) &= \frac{1}{4} \delta U(\zeta) - \frac{3}{8} \delta U(u, \zeta) , \\ \delta J(u, \zeta) &= \frac{1}{4} \delta U(\zeta) - \frac{1}{2} \delta U(u, \zeta) , \\ \delta J(u, \eta) &= \frac{1}{4} \delta U(\zeta) - \frac{1}{8} \delta U(u, \zeta) , \\ \delta J(u, \xi) &= \frac{1}{4} \delta U(\zeta) - \frac{1}{8} \delta U(u, \zeta) , \\ \delta J(\zeta, \eta) &= \frac{1}{2} \delta U(\zeta) - \frac{1}{2} \delta U(\zeta, \eta) , \\ \delta J(\zeta, \xi) &= \frac{1}{2} \delta U(\zeta) - \frac{1}{2} \delta U(\zeta, \eta) , \\ \delta J(\eta, \xi) &= \frac{1}{2} \delta U(\zeta) - \frac{1}{2} \delta U(\zeta, \eta) , \\ \delta T(\eta; v, u) &= \frac{\sqrt{3}}{4} \delta U(u, \zeta) , \\ \delta T(\xi; v, u) &= -\frac{\sqrt{3}}{4} \delta U(u, \zeta) , \\ \delta A(\eta; v, u) &= -\frac{\sqrt{3}}{8} \delta U(u, \zeta) , \\ \delta A(\xi; v, u) &= \frac{\sqrt{3}}{8} \delta U(u, \zeta) , \\ \delta S(v, \zeta; \eta, \xi) &= \frac{27}{16} \delta U(u, \zeta) - \frac{3}{4} \delta U(\zeta, \eta) , \\ \delta S(v, \zeta; \xi, \eta) &= -\frac{27}{16} \delta U(u, \zeta) + \frac{3}{4} \delta U(\zeta, \eta) , \\ \delta S(u, \zeta; \eta, \xi) &= -\frac{9}{16} \sqrt{3} \delta U(u, \zeta) + \frac{\sqrt{3}}{4} \delta U(\zeta, \eta) , \\ \delta S(u, \zeta; \xi, \eta) &= -\frac{9}{16} \sqrt{3} \delta U(u, \zeta) + \frac{\sqrt{3}}{4} \delta U(\zeta, \eta) , \end{aligned}$$

$$\delta S(u, \eta; \xi, \zeta) = \frac{9}{8} \sqrt{3} \delta U(u, \zeta) - \frac{\sqrt{3}}{2} \delta U(\zeta, \eta) .$$

## 2.2 *d*-orbitals, group $T_h$

Independent parameter variations:

$$\delta U(\zeta), \delta U(u, \zeta), \delta U(\zeta, \eta).$$

Dependent parameter variations:

$$\begin{aligned} \delta U(\eta) &= \delta U(\zeta) , \\ \delta U(\xi) &= \delta U(\zeta) , \\ \delta U(v, \eta) &= \frac{3}{4} \delta U(u, \zeta) , \\ \delta U(v, \xi) &= \frac{3}{4} \delta U(u, \zeta) , \\ \delta U(u, \eta) &= \frac{1}{4} \delta U(u, \zeta) , \\ \delta U(u, \xi) &= \frac{1}{4} \delta U(u, \zeta) , \\ \delta U(\zeta, \xi) &= \delta U(\zeta, \eta) , \\ \delta U(\eta, \xi) &= \delta U(\zeta, \eta) , \\ \delta J(v, \zeta) &= \frac{1}{4} \delta U(\zeta) , \\ \delta J(v, \eta) &= \frac{1}{4} \delta U(\zeta) - \frac{3}{8} \delta U(u, \zeta) , \\ \delta J(v, \xi) &= \frac{1}{4} \delta U(\zeta) - \frac{3}{8} \delta U(u, \zeta) , \\ \delta J(u, \zeta) &= \frac{1}{4} \delta U(\zeta) - \frac{1}{2} \delta U(u, \zeta) , \\ \delta J(u, \eta) &= \frac{1}{4} \delta U(\zeta) - \frac{1}{8} \delta U(u, \zeta) , \\ \delta J(u, \xi) &= \frac{1}{4} \delta U(\zeta) - \frac{1}{8} \delta U(u, \zeta) , \\ \delta J(\zeta, \eta) &= \frac{1}{2} \delta U(\zeta) - \frac{1}{2} \delta U(\zeta, \eta) , \\ \delta J(\zeta, \xi) &= \frac{1}{2} \delta U(\zeta) - \frac{1}{2} \delta U(\zeta, \eta) , \\ \delta J(\eta, \xi) &= \frac{1}{2} \delta U(\zeta) - \frac{1}{2} \delta U(\zeta, \eta) , \\ \delta T(\eta; v, u) &= \frac{\sqrt{3}}{4} \delta U(u, \zeta) , \\ \delta T(\xi; v, u) &= -\frac{\sqrt{3}}{4} \delta U(u, \zeta) , \\ \delta A(\eta; v, u) &= -\frac{\sqrt{3}}{8} \delta U(u, \zeta) , \\ \delta A(\xi; v, u) &= \frac{\sqrt{3}}{8} \delta U(u, \zeta) , \\ \delta S(v, \zeta; \eta, \xi) &= \frac{27}{16} \delta U(u, \zeta) - \frac{3}{4} \delta U(\zeta, \eta) , \\ \delta S(v, \zeta; \xi, \eta) &= -\frac{27}{16} \delta U(u, \zeta) + \frac{3}{4} \delta U(\zeta, \eta) , \\ \delta S(u, \zeta; \eta, \xi) &= -\frac{9}{16} \sqrt{3} \delta U(u, \zeta) + \frac{\sqrt{3}}{4} \delta U(\zeta, \eta) , \\ \delta S(u, \zeta; \xi, \eta) &= -\frac{9}{16} \sqrt{3} \delta U(u, \zeta) + \frac{\sqrt{3}}{4} \delta U(\zeta, \eta) , \\ \delta S(u, \eta; \xi, \zeta) &= \frac{9}{8} \sqrt{3} \delta U(u, \zeta) - \frac{\sqrt{3}}{2} \delta U(\zeta, \eta) . \end{aligned}$$

### 2.3 *d*-orbitals, group $D_{6h}$

Independent parameter variations:

$$\delta U(u), \delta U(\eta), \delta U(u, \zeta), \delta U(\eta, \xi), \delta U(v, \eta), \delta U(u, \eta).$$

Dependent parameter variations:

$$\begin{aligned} \delta U(\zeta) &= \delta U(u) , \\ \delta U(\xi) &= \delta U(\eta) , \\ \delta U(v, \xi) &= \delta U(v, \eta) , \\ \delta U(u, \xi) &= \delta U(u, \eta) , \\ \delta U(\zeta, \eta) &= \delta U(\eta, \xi) - \delta U(v, \eta) , \\ \delta U(\zeta, \xi) &= \delta U(\eta, \xi) - \delta U(v, \eta) , \\ \delta J(v, u) &= \frac{1}{4} \delta U(u) , \\ \delta J(v, \zeta) &= \frac{1}{4} \delta U(u) , \\ \delta J(v, \eta) &= \frac{1}{4} \delta U(\eta) - \frac{1}{2} \delta U(v, \eta) , \\ \delta J(v, \xi) &= \frac{1}{4} \delta U(\eta) - \frac{1}{2} \delta U(v, \eta) , \\ \delta J(u, \zeta) &= \frac{1}{2} \delta U(u) - \frac{1}{2} \delta U(u, \zeta) , \\ \delta J(u, \eta) &= \frac{1}{4} \delta U(u) + \frac{1}{4} \delta U(\eta) - \frac{1}{2} \delta U(u, \eta) , \\ \delta J(u, \xi) &= \frac{1}{4} \delta U(u) + \frac{1}{4} \delta U(\eta) - \frac{1}{2} \delta U(u, \eta) , \\ \delta J(\zeta, \eta) &= \frac{1}{4} \delta U(u) + \frac{1}{4} \delta U(\eta) - \frac{1}{2} \delta U(\eta, \xi) + \frac{1}{2} \delta U(v, \eta) , \\ \delta J(\zeta, \xi) &= \frac{1}{4} \delta U(u) + \frac{1}{4} \delta U(\eta) - \frac{1}{2} \delta U(\eta, \xi) + \frac{1}{2} \delta U(v, \eta) , \\ \delta J(\eta, \xi) &= \frac{1}{2} \delta U(\eta) - \frac{1}{2} \delta U(\eta, \xi) , \\ \delta T(\eta; v, u) &= -\frac{\sqrt{3}}{2} \delta U(u, \zeta) + \sqrt{3} \delta U(\eta, \xi) - \frac{3}{2} \sqrt{3} \delta U(v, \eta) - \frac{\sqrt{3}}{2} \delta U(u, \eta) , \\ \delta T(\xi; v, u) &= \frac{\sqrt{3}}{2} \delta U(u, \zeta) - \sqrt{3} \delta U(\eta, \xi) + \frac{3}{2} \sqrt{3} \delta U(v, \eta) + \frac{\sqrt{3}}{2} \delta U(u, \eta) , \\ \delta A(\eta; v, u) &= \frac{\sqrt{3}}{4} \delta U(u, \zeta) - \frac{\sqrt{3}}{2} \delta U(\eta, \xi) + 3 \frac{\sqrt{3}}{4} \delta U(v, \eta) + \frac{\sqrt{3}}{4} \delta U(u, \eta) , \\ \delta A(\xi; v, u) &= -\frac{\sqrt{3}}{4} \delta U(u, \zeta) + \frac{\sqrt{3}}{2} \delta U(\eta, \xi) - 3 \frac{\sqrt{3}}{4} \delta U(v, \eta) - \frac{\sqrt{3}}{4} \delta U(u, \eta) , \\ \delta S(v, \zeta; \eta, \xi) &= -\frac{3}{4} \delta U(u, \zeta) + \frac{3}{2} \delta U(\eta, \xi) - \frac{9}{4} \delta U(v, \eta) - \frac{3}{4} \delta U(u, \eta) , \\ \delta S(v, \zeta; \xi, \eta) &= \frac{3}{4} \delta U(u, \zeta) - \frac{3}{2} \delta U(\eta, \xi) + \frac{9}{4} \delta U(v, \eta) + \frac{3}{4} \delta U(u, \eta) , \\ \delta S(u, \zeta; \eta, \xi) &= -\frac{\sqrt{3}}{4} \delta U(\eta, \xi) + \frac{\sqrt{3}}{4} \delta U(v, \eta) + \frac{\sqrt{3}}{4} \delta U(u, \eta) , \\ \delta S(u, \zeta; \xi, \eta) &= -\frac{\sqrt{3}}{4} \delta U(\eta, \xi) + \frac{\sqrt{3}}{4} \delta U(v, \eta) + \frac{\sqrt{3}}{4} \delta U(u, \eta) , \\ \delta S(u, \eta; \xi, \zeta) &= \frac{\sqrt{3}}{2} \delta U(\eta, \xi) - \frac{\sqrt{3}}{2} \delta U(v, \eta) - \frac{\sqrt{3}}{2} \delta U(u, \eta) . \end{aligned}$$

## 2.4 *d*-orbitals, group $D_{4h}$

Independent parameter variations:

$$\delta U(\eta), \delta U(u), \delta U(\zeta), \delta U(u, \zeta), \delta U(v, \eta), \delta U(u, \eta), \delta U(\zeta, \eta), \delta U(\eta, \xi), \delta T(\eta; v, u).$$

Dependent parameter variations:

$$\delta U(\xi) = \delta U(\eta) ,$$

$$\delta U(v, \xi) = \delta U(v, \eta) ,$$

$$\delta U(u, \xi) = \delta U(u, \eta) ,$$

$$\delta U(\zeta, \xi) = \delta U(\zeta, \eta) ,$$

$$\delta J(v, u) = \frac{1}{4}\delta U(u) ,$$

$$\delta J(v, \zeta) = \frac{1}{4}\delta U(\zeta) ,$$

$$\delta J(v, \eta) = \frac{1}{4}\delta U(\eta) - \frac{1}{2}\delta U(v, \eta) ,$$

$$\delta J(v, \xi) = \frac{1}{4}\delta U(\eta) - \frac{1}{2}\delta U(v, \eta) ,$$

$$\delta J(u, \zeta) = \frac{1}{4}\delta U(u) + \frac{1}{4}\delta U(\zeta) - \frac{1}{2}\delta U(u, \zeta) ,$$

$$\delta J(u, \eta) = \frac{1}{4}\delta U(\eta) + \frac{1}{4}\delta U(u) - \frac{1}{2}\delta U(u, \eta) ,$$

$$\delta J(u, \xi) = \frac{1}{4}\delta U(\eta) + \frac{1}{4}\delta U(u) - \frac{1}{2}\delta U(u, \eta) ,$$

$$\delta J(\zeta, \eta) = \frac{1}{4}\delta U(\eta) + \frac{1}{4}\delta U(\zeta) - \frac{1}{2}\delta U(\zeta, \eta) ,$$

$$\delta J(\zeta, \xi) = \frac{1}{4}\delta U(\eta) + \frac{1}{4}\delta U(\zeta) - \frac{1}{2}\delta U(\zeta, \eta) ,$$

$$\delta J(\eta, \xi) = \frac{1}{2}\delta U(\eta) - \frac{1}{2}\delta U(\eta, \xi) ,$$

$$\delta T(\eta; v, u) = \delta T(\eta; v, u) ,$$

$$\delta T(\xi; v, u) = -\delta T(\eta; v, u) ,$$

$$\delta A(\eta; v, u) = -\frac{1}{2}\delta T(\eta; v, u) ,$$

$$\delta A(\xi; v, u) = \frac{1}{2}\delta T(\eta; v, u) ,$$

$$\delta S(v, \zeta; \eta, \xi) = \frac{3}{8}\delta U(u, \zeta) + \frac{7}{8}\delta U(v, \eta) + \frac{3}{8}\delta U(u, \eta) - \frac{1}{4}\delta U(\zeta, \eta) - \frac{1}{2}\delta U(\eta, \xi) + 3\frac{\sqrt{3}}{4}\delta T(\eta; v, u) ,$$

$$\delta S(v, \zeta; \xi, \eta) = -\frac{3}{8}\delta U(u, \zeta) - \frac{7}{8}\delta U(v, \eta) - \frac{3}{8}\delta U(u, \eta) + \frac{1}{4}\delta U(\zeta, \eta) + \frac{1}{2}\delta U(\eta, \xi) - 3\frac{\sqrt{3}}{4}\delta T(\eta; v, u) ,$$

$$\delta S(u, \zeta; \eta, \xi) = -\frac{\sqrt{3}}{4}\delta U(u, \zeta) - \frac{\sqrt{3}}{4}\delta U(v, \eta) + \frac{\sqrt{3}}{4}\delta U(\zeta, \eta) - \frac{1}{2}\delta T(\eta; v, u) ,$$

$$\delta S(u, \zeta; \xi, \eta) = -\frac{\sqrt{3}}{4}\delta U(u, \zeta) - \frac{\sqrt{3}}{4}\delta U(v, \eta) + \frac{\sqrt{3}}{4}\delta U(\zeta, \eta) - \frac{1}{2}\delta T(\eta; v, u) ,$$

$$\delta S(u, \eta; \xi, \zeta) = \frac{\sqrt{3}}{2}\delta U(u, \zeta) + \frac{\sqrt{3}}{2}\delta U(v, \eta) - \frac{\sqrt{3}}{2}\delta U(\zeta, \eta) + \delta T(\eta; v, u) .$$



## 2.5 $f$ -orbitals, groups $O_h$ , $O$ , $T_d$

Independent parameter variations:

$$\delta U(\alpha), \delta U(a, \alpha), \delta U(x, \alpha), \delta U(x, \beta), \delta U(\alpha, \beta), \delta J(a, x), \delta J(x, y), \delta J(\alpha, \beta).$$

Dependent parameter variations:

$$\begin{aligned} \delta U(\beta) &= \delta U(\alpha) , \\ \delta U(\gamma) &= \delta U(\alpha) , \\ \delta U(a, \beta) &= \delta U(a, \alpha) , \\ \delta U(a, \gamma) &= \delta U(a, \alpha) , \\ \delta U(x, \gamma) &= \delta U(x, \beta) , \\ \delta U(y, \alpha) &= \delta U(x, \beta) , \\ \delta U(y, \beta) &= \delta U(x, \alpha) , \\ \delta U(y, \gamma) &= \delta U(x, \beta) , \\ \delta U(z, \alpha) &= \delta U(x, \beta) , \\ \delta U(z, \beta) &= \delta U(x, \beta) , \\ \delta U(z, \gamma) &= \delta U(x, \alpha) , \\ \delta U(\alpha, \gamma) &= \delta U(\alpha, \beta) , \\ \delta U(\beta, \gamma) &= \delta U(\alpha, \beta) , \\ \delta J(a, y) &= \delta J(a, x) , \\ \delta J(a, z) &= \delta J(a, x) , \\ \delta J(a, \alpha) &= \frac{1}{4}\delta U(\alpha) - \frac{1}{2}\delta U(a, \alpha) , \\ \delta J(a, \beta) &= \frac{1}{4}\delta U(\alpha) - \frac{1}{2}\delta U(a, \alpha) , \\ \delta J(a, \gamma) &= \frac{1}{4}\delta U(\alpha) - \frac{1}{2}\delta U(a, \alpha) , \\ \delta J(x, z) &= \delta J(x, y) , \\ \delta J(x, \alpha) &= -\frac{1}{60}\delta U(\alpha) - \frac{1}{2}\delta U(x, \alpha) + \frac{4}{5}\delta U(\alpha, \beta) - \frac{8}{15}\delta J(x, y) \\ &\quad + \frac{8}{15}\delta J(\alpha, \beta) , \\ \delta J(x, \beta) &= \frac{7}{30}\delta U(\alpha) - \frac{1}{2}\delta U(x, \beta) + \frac{1}{60}\delta U(\alpha, \beta) + \frac{3}{10}\delta J(x, y) \\ &\quad + \frac{1}{30}\delta J(\alpha, \beta) , \\ \delta J(x, \gamma) &= \frac{7}{30}\delta U(\alpha) - \frac{1}{2}\delta U(x, \beta) + \frac{1}{60}\delta U(\alpha, \beta) + \frac{3}{10}\delta J(x, y) \\ &\quad + \frac{1}{30}\delta J(\alpha, \beta) , \\ \delta J(y, z) &= \delta J(x, y) , \\ \delta J(y, \alpha) &= \frac{7}{30}\delta U(\alpha) - \frac{1}{2}\delta U(x, \beta) + \frac{1}{60}\delta U(\alpha, \beta) + \frac{3}{10}\delta J(x, y) \\ &\quad + \frac{1}{30}\delta J(\alpha, \beta) , \\ \delta J(y, \beta) &= -\frac{1}{60}\delta U(\alpha) - \frac{1}{2}\delta U(x, \alpha) + \frac{4}{5}\delta U(\alpha, \beta) - \frac{8}{15}\delta J(x, y) \\ &\quad + \frac{8}{15}\delta J(\alpha, \beta) , \\ \delta J(y, \gamma) &= \frac{7}{30}\delta U(\alpha) - \frac{1}{2}\delta U(x, \beta) + \frac{1}{60}\delta U(\alpha, \beta) + \frac{3}{10}\delta J(x, y) \end{aligned}$$

$$\begin{aligned}
& + \frac{1}{30} \delta J(\alpha, \beta) , \\
\delta J(z, \alpha) &= \frac{7}{30} \delta U(\alpha) - \frac{1}{2} \delta U(x, \beta) + \frac{1}{60} \delta U(\alpha, \beta) + \frac{3}{10} \delta J(x, y) \\
& + \frac{1}{30} \delta J(\alpha, \beta) , \\
\delta J(z, \beta) &= \frac{7}{30} \delta U(\alpha) - \frac{1}{2} \delta U(x, \beta) + \frac{1}{60} \delta U(\alpha, \beta) + \frac{3}{10} \delta J(x, y) \\
& + \frac{1}{30} \delta J(\alpha, \beta) , \\
\delta J(z, \gamma) &= -\frac{1}{60} \delta U(\alpha) - \frac{1}{2} \delta U(x, \alpha) + \frac{4}{5} \delta U(\alpha, \beta) - \frac{8}{15} \delta J(x, y) \\
& + \frac{8}{15} \delta J(\alpha, \beta) , \\
\delta J(\alpha, \beta) &= \delta J(\alpha, \beta) , \\
\delta J(\alpha, \gamma) &= \delta J(\alpha, \beta) , \\
\delta J(\beta, \gamma) &= \delta J(\alpha, \beta) , \\
\delta T(y; x, \alpha) &= \frac{2}{5\sqrt{15}} \delta U(\alpha) + \frac{9}{4} \sqrt{\frac{3}{5}} \delta U(x, \alpha) - \frac{3}{8} \sqrt{\frac{3}{5}} \delta U(x, \beta) - \frac{257}{80\sqrt{15}} \delta U(\alpha, \beta) \\
& + 2\sqrt{\frac{3}{5}} \delta J(x, y) - \frac{4}{5\sqrt{15}} \delta J(\alpha, \beta) , \\
\delta T(x; y, \beta) &= \frac{2}{5\sqrt{15}} \delta U(\alpha) + \frac{9}{4} \sqrt{\frac{3}{5}} \delta U(x, \alpha) - \frac{3}{8} \sqrt{\frac{3}{5}} \delta U(x, \beta) - \frac{257}{80\sqrt{15}} \delta U(\alpha, \beta) \\
& + 2\sqrt{\frac{3}{5}} \delta J(x, y) - \frac{4}{5\sqrt{15}} \delta J(\alpha, \beta) , \\
\delta T(z; x, \alpha) &= -\frac{2}{5\sqrt{15}} \delta U(\alpha) - \frac{9}{4} \sqrt{\frac{3}{5}} \delta U(x, \alpha) + \frac{3}{8} \sqrt{\frac{3}{5}} \delta U(x, \beta) + \frac{257}{80\sqrt{15}} \delta U(\alpha, \beta) \\
& - 2\sqrt{\frac{3}{5}} \delta J(x, y) + \frac{4}{5\sqrt{15}} \delta J(\alpha, \beta) , \\
\delta T(x; z, \gamma) &= \frac{2}{5\sqrt{15}} \delta U(\alpha) + \frac{9}{4} \sqrt{\frac{3}{5}} \delta U(x, \alpha) - \frac{3}{8} \sqrt{\frac{3}{5}} \delta U(x, \beta) - \frac{257}{80\sqrt{15}} \delta U(\alpha, \beta) \\
& + 2\sqrt{\frac{3}{5}} \delta J(x, y) - \frac{4}{5\sqrt{15}} \delta J(\alpha, \beta) , \\
\delta T(\beta; x, \alpha) &= -\frac{1}{4\sqrt{15}} \delta U(x, \alpha) - \frac{13}{8\sqrt{15}} \delta U(x, \beta) + \frac{1}{9} \sqrt{\frac{5}{3}} \delta U(\alpha, \beta) - \frac{2}{3\sqrt{15}} \delta J(x, y) , \\
\delta T(\gamma; x, \alpha) &= \frac{1}{4\sqrt{15}} \delta U(x, \alpha) + \frac{13}{8\sqrt{15}} \delta U(x, \beta) - \frac{1}{9} \sqrt{\frac{5}{3}} \delta U(\alpha, \beta) + \frac{2}{3\sqrt{15}} \delta J(x, y) , \\
\delta T(z; y, \beta) &= -\frac{2}{5\sqrt{15}} \delta U(\alpha) - \frac{9}{4} \sqrt{\frac{3}{5}} \delta U(x, \alpha) + \frac{3}{8} \sqrt{\frac{3}{5}} \delta U(x, \beta) + \frac{257}{80\sqrt{15}} \delta U(\alpha, \beta) \\
& - 2\sqrt{\frac{3}{5}} \delta J(x, y) + \frac{4}{5\sqrt{15}} \delta J(\alpha, \beta) , \\
\delta T(y; z, \gamma) &= -\frac{2}{5\sqrt{15}} \delta U(\alpha) - \frac{9}{4} \sqrt{\frac{3}{5}} \delta U(x, \alpha) + \frac{3}{8} \sqrt{\frac{3}{5}} \delta U(x, \beta) + \frac{257}{80\sqrt{15}} \delta U(\alpha, \beta) \\
& - 2\sqrt{\frac{3}{5}} \delta J(x, y) + \frac{4}{5\sqrt{15}} \delta J(\alpha, \beta) , \\
\delta T(\alpha; y, \beta) &= -\frac{1}{4\sqrt{15}} \delta U(x, \alpha) - \frac{13}{8\sqrt{15}} \delta U(x, \beta) + \frac{1}{9} \sqrt{\frac{5}{3}} \delta U(\alpha, \beta) - \frac{2}{3\sqrt{15}} \delta J(x, y) ,
\end{aligned}$$

$$\begin{aligned}
\delta T(\gamma; y, \beta) &= \frac{1}{4\sqrt{15}}\delta U(x, \alpha) + \frac{13}{8\sqrt{15}}\delta U(x, \beta) - \frac{1}{9}\sqrt{\frac{5}{3}}\delta U(\alpha, \beta) + \frac{2}{3\sqrt{15}}\delta J(x, y) , \\
\delta T(\alpha; z, \gamma) &= -\frac{1}{4\sqrt{15}}\delta U(x, \alpha) - \frac{13}{8\sqrt{15}}\delta U(x, \beta) + \frac{1}{9}\sqrt{\frac{5}{3}}\delta U(\alpha, \beta) - \frac{2}{3\sqrt{15}}\delta J(x, y) , \\
\delta T(\beta; z, \gamma) &= \frac{1}{4\sqrt{15}}\delta U(x, \alpha) + \frac{13}{8\sqrt{15}}\delta U(x, \beta) - \frac{1}{9}\sqrt{\frac{5}{3}}\delta U(\alpha, \beta) + \frac{2}{3\sqrt{15}}\delta J(x, y) , \\
\delta A(x; x, \beta) &= \frac{1}{40\sqrt{15}}\delta U(\alpha) - \frac{9}{8}\sqrt{\frac{3}{5}}\delta U(x, \alpha) + \frac{3}{16}\sqrt{\frac{3}{5}}\delta U(x, \beta) + \frac{221}{800}\sqrt{\frac{3}{5}}\delta U(\alpha, \beta) \\
&\quad - \frac{1}{4}\sqrt{\frac{3}{5}}\delta J(x, y) - \frac{1}{20\sqrt{15}}\delta J(\alpha, \beta) , \\
\delta A(x; x, \gamma) &= \frac{1}{40\sqrt{15}}\delta U(\alpha) - \frac{9}{8}\sqrt{\frac{3}{5}}\delta U(x, \alpha) + \frac{3}{16}\sqrt{\frac{3}{5}}\delta U(x, \beta) + \frac{221}{800}\sqrt{\frac{3}{5}}\delta U(\alpha, \beta) \\
&\quad - \frac{1}{4}\sqrt{\frac{3}{5}}\delta J(x, y) - \frac{1}{20\sqrt{15}}\delta J(\alpha, \beta) , \\
\delta A(y; x, \alpha) &= \frac{1}{40\sqrt{15}}\delta U(\alpha) - \frac{9}{8}\sqrt{\frac{3}{5}}\delta U(x, \alpha) + \frac{3}{16}\sqrt{\frac{3}{5}}\delta U(x, \beta) + \frac{221}{800}\sqrt{\frac{3}{5}}\delta U(\alpha, \beta) \\
&\quad - \frac{1}{4}\sqrt{\frac{3}{5}}\delta J(x, y) - \frac{1}{20\sqrt{15}}\delta J(\alpha, \beta) , \\
\delta A(z; x, \alpha) &= -\frac{1}{40\sqrt{15}}\delta U(\alpha) + \frac{9}{8}\sqrt{\frac{3}{5}}\delta U(x, \alpha) - \frac{3}{16}\sqrt{\frac{3}{5}}\delta U(x, \beta) - \frac{221}{800}\sqrt{\frac{3}{5}}\delta U(\alpha, \beta) \\
&\quad + \frac{1}{4}\sqrt{\frac{3}{5}}\delta J(x, y) + \frac{1}{20\sqrt{15}}\delta J(\alpha, \beta) , \\
\delta A(\beta; x, \alpha) &= -\frac{1}{8}\sqrt{\frac{3}{5}}\delta U(\alpha) + \frac{1}{8\sqrt{15}}\delta U(x, \alpha) + \frac{13}{16\sqrt{15}}\delta U(x, \beta) - \frac{1}{32}\sqrt{\frac{3}{5}}\delta U(\alpha, \beta) \\
&\quad - \frac{1}{12\sqrt{15}}\delta J(x, y) + \frac{1}{4}\sqrt{\frac{3}{5}}\delta J(\alpha, \beta) , \\
\delta A(\gamma; x, \alpha) &= \frac{1}{8}\sqrt{\frac{3}{5}}\delta U(\alpha) - \frac{1}{8\sqrt{15}}\delta U(x, \alpha) - \frac{13}{16\sqrt{15}}\delta U(x, \beta) + \frac{1}{32}\sqrt{\frac{3}{5}}\delta U(\alpha, \beta) \\
&\quad + \frac{1}{12\sqrt{15}}\delta J(x, y) - \frac{1}{4}\sqrt{\frac{3}{5}}\delta J(\alpha, \beta) , \\
\delta A(y; y, \gamma) &= -\frac{1}{40\sqrt{15}}\delta U(\alpha) + \frac{9}{8}\sqrt{\frac{3}{5}}\delta U(x, \alpha) - \frac{3}{16}\sqrt{\frac{3}{5}}\delta U(x, \beta) - \frac{221}{800}\sqrt{\frac{3}{5}}\delta U(\alpha, \beta) \\
&\quad + \frac{1}{4}\sqrt{\frac{3}{5}}\delta J(x, y) + \frac{1}{20\sqrt{15}}\delta J(\alpha, \beta) , \\
\delta A(z; y, \beta) &= -\frac{1}{40\sqrt{15}}\delta U(\alpha) + \frac{9}{8}\sqrt{\frac{3}{5}}\delta U(x, \alpha) - \frac{3}{16}\sqrt{\frac{3}{5}}\delta U(x, \beta) - \frac{221}{800}\sqrt{\frac{3}{5}}\delta U(\alpha, \beta) \\
&\quad + \frac{1}{4}\sqrt{\frac{3}{5}}\delta J(x, y) + \frac{1}{20\sqrt{15}}\delta J(\alpha, \beta) , \\
\delta A(\alpha; y, \beta) &= -\frac{1}{8}\sqrt{\frac{3}{5}}\delta U(\alpha) + \frac{1}{8\sqrt{15}}\delta U(x, \alpha) + \frac{13}{16\sqrt{15}}\delta U(x, \beta) - \frac{1}{32}\sqrt{\frac{3}{5}}\delta U(\alpha, \beta) \\
&\quad - \frac{1}{12\sqrt{15}}\delta J(x, y) + \frac{1}{4}\sqrt{\frac{3}{5}}\delta J(\alpha, \beta) , \\
\delta A(\gamma; y, \beta) &= \frac{1}{8}\sqrt{\frac{3}{5}}\delta U(\alpha) - \frac{1}{8\sqrt{15}}\delta U(x, \alpha) - \frac{13}{16\sqrt{15}}\delta U(x, \beta) + \frac{1}{32}\sqrt{\frac{3}{5}}\delta U(\alpha, \beta)
\end{aligned}$$

$$\begin{aligned}
& + \frac{1}{12\sqrt{15}}\delta J(x, y) - \frac{1}{4}\sqrt{\frac{3}{5}}\delta J(\alpha, \beta) , \\
\delta A(\alpha; z, \gamma) &= -\frac{1}{8}\sqrt{\frac{3}{5}}\delta U(\alpha) + \frac{1}{8\sqrt{15}}\delta U(x, \alpha) + \frac{13}{16\sqrt{15}}\delta U(x, \beta) - \frac{1}{32}\sqrt{\frac{3}{5}}\delta U(\alpha, \beta) \\
& - \frac{1}{12\sqrt{15}}\delta J(x, y) + \frac{1}{4}\sqrt{\frac{3}{5}}\delta J(\alpha, \beta) , \\
\delta A(\beta; z, \gamma) &= \frac{1}{8}\sqrt{\frac{3}{5}}\delta U(\alpha) - \frac{1}{8\sqrt{15}}\delta U(x, \alpha) - \frac{13}{16\sqrt{15}}\delta U(x, \beta) + \frac{1}{32}\sqrt{\frac{3}{5}}\delta U(\alpha, \beta) \\
& + \frac{1}{12\sqrt{15}}\delta J(x, y) - \frac{1}{4}\sqrt{\frac{3}{5}}\delta J(\alpha, \beta) , \\
\delta S(a, x; y, z) &= \frac{1}{8}\sqrt{\frac{3}{5}}\delta J(a, x) - \frac{4}{5\sqrt{15}}\delta J(x, y) , \\
\delta S(a, x; z, y) &= \frac{1}{8}\sqrt{\frac{3}{5}}\delta J(a, x) - \frac{4}{5\sqrt{15}}\delta J(x, y) , \\
\delta S(a, x; \beta, z) &= \frac{1}{30}\delta U(\alpha) - \frac{3}{16}\delta U(a, \alpha) + \frac{79}{160}\delta U(x, \alpha) + \frac{7}{320}\delta U(x, \beta) \\
& - \frac{379}{1920}\delta U(\alpha, \beta) - \frac{1}{8}\delta J(a, x) + \frac{73}{180}\delta J(x, y) - \frac{1}{15}\delta J(\alpha, \beta) , \\
\delta S(a, x; \beta, \gamma) &= \frac{1}{9}\sqrt{\frac{5}{3}}\delta U(a, \alpha) + \frac{1}{32\sqrt{15}}\delta U(x, \alpha) + \frac{73}{64\sqrt{15}}\delta U(x, \beta) - \frac{9\sqrt{15}}{128}\delta U(\alpha, \beta) \\
& + \frac{1}{12\sqrt{15}}\delta J(x, y) , \\
\delta S(a, x; \gamma, y) &= \frac{1}{30}\delta U(\alpha) - \frac{3}{16}\delta U(a, \alpha) + \frac{79}{160}\delta U(x, \alpha) + \frac{7}{320}\delta U(x, \beta) \\
& - \frac{379}{1920}\delta U(\alpha, \beta) - \frac{1}{8}\delta J(a, x) + \frac{73}{180}\delta J(x, y) - \frac{1}{15}\delta J(\alpha, \beta) , \\
\delta S(a, x; \gamma, \beta) &= \frac{1}{9}\sqrt{\frac{5}{3}}\delta U(a, \alpha) + \frac{1}{32\sqrt{15}}\delta U(x, \alpha) + \frac{73}{64\sqrt{15}}\delta U(x, \beta) - \frac{9\sqrt{15}}{128}\delta U(\alpha, \beta) \\
& + \frac{1}{12\sqrt{15}}\delta J(x, y) , \\
\delta S(a, y; z, x) &= \frac{1}{8}\sqrt{\frac{3}{5}}\delta J(a, x) - \frac{4}{5\sqrt{15}}\delta J(x, y) , \\
\delta S(a, y; \alpha, z) &= \frac{1}{30}\delta U(\alpha) - \frac{3}{16}\delta U(a, \alpha) + \frac{79}{160}\delta U(x, \alpha) + \frac{7}{320}\delta U(x, \beta) \\
& - \frac{379}{1920}\delta U(\alpha, \beta) - \frac{1}{8}\delta J(a, x) + \frac{73}{180}\delta J(x, y) - \frac{1}{15}\delta J(\alpha, \beta) , \\
\delta S(a, y; \alpha, \gamma) &= -\frac{1}{9}\sqrt{\frac{5}{3}}\delta U(a, \alpha) - \frac{1}{32\sqrt{15}}\delta U(x, \alpha) - \frac{73}{64\sqrt{15}}\delta U(x, \beta) + \frac{9\sqrt{15}}{128}\delta U(\alpha, \beta) \\
& - \frac{1}{12\sqrt{15}}\delta J(x, y) , \\
\delta S(a, y; \gamma, x) &= -\frac{1}{30}\delta U(\alpha) + \frac{3}{16}\delta U(a, \alpha) - \frac{79}{160}\delta U(x, \alpha) - \frac{7}{320}\delta U(x, \beta) \\
& + \frac{379}{1920}\delta U(\alpha, \beta) + \frac{1}{8}\delta J(a, x) - \frac{73}{180}\delta J(x, y) + \frac{1}{15}\delta J(\alpha, \beta) , \\
\delta S(a, y; \gamma, \alpha) &= -\frac{1}{9}\sqrt{\frac{5}{3}}\delta U(a, \alpha) - \frac{1}{32\sqrt{15}}\delta U(x, \alpha) - \frac{73}{64\sqrt{15}}\delta U(x, \beta) + \frac{9\sqrt{15}}{128}\delta U(\alpha, \beta) \\
& - \frac{1}{12\sqrt{15}}\delta J(x, y) , \\
\delta S(a, z; \alpha, y) &= -\frac{1}{30}\delta U(\alpha) + \frac{3}{16}\delta U(a, \alpha) - \frac{79}{160}\delta U(x, \alpha) - \frac{7}{320}\delta U(x, \beta)
\end{aligned}$$

$$\begin{aligned}
& + \frac{379}{1920} \delta U(\alpha, \beta) + \frac{1}{8} \delta J(a, x) - \frac{73}{180} \delta J(x, y) + \frac{1}{15} \delta J(\alpha, \beta) , \\
\delta S(a, z; \alpha, \beta) &= \frac{1}{9} \sqrt{\frac{5}{3}} \delta U(a, \alpha) + \frac{1}{32\sqrt{15}} \delta U(x, \alpha) + \frac{73}{64\sqrt{15}} \delta U(x, \beta) - \frac{9\sqrt{15}}{128} \delta U(\alpha, \beta) \\
& + \frac{1}{12\sqrt{15}} \delta J(x, y) , \\
\delta S(a, z; \beta, x) &= -\frac{1}{30} \delta U(\alpha) + \frac{3}{16} \delta U(a, \alpha) - \frac{79}{160} \delta U(x, \alpha) - \frac{7}{320} \delta U(x, \beta) \\
& + \frac{379}{1920} \delta U(\alpha, \beta) + \frac{1}{8} \delta J(a, x) - \frac{73}{180} \delta J(x, y) + \frac{1}{15} \delta J(\alpha, \beta) , \\
\delta S(a, z; \beta, \alpha) &= \frac{1}{9} \sqrt{\frac{5}{3}} \delta U(a, \alpha) + \frac{1}{32\sqrt{15}} \delta U(x, \alpha) + \frac{73}{64\sqrt{15}} \delta U(x, \beta) - \frac{9\sqrt{15}}{128} \delta U(\alpha, \beta) \\
& + \frac{1}{12\sqrt{15}} \delta J(x, y) , \\
\delta S(a, \alpha; \beta, z) &= \frac{1}{\sqrt{15}} \delta U(\alpha) - \frac{1}{8\sqrt{15}} \delta U(a, \alpha) - \frac{1}{16\sqrt{15}} \delta U(x, \alpha) - \frac{73}{32\sqrt{15}} \delta U(x, \beta) \\
& + \frac{71}{64\sqrt{15}} \delta U(\alpha, \beta) - \frac{1}{8\sqrt{15}} \delta J(a, x) + \frac{1}{2\sqrt{15}} \delta J(x, y) - \frac{2}{\sqrt{15}} \delta J(\alpha, \beta) , \\
\delta S(a, \alpha; \gamma, y) &= -\frac{1}{\sqrt{15}} \delta U(\alpha) + \frac{1}{8\sqrt{15}} \delta U(a, \alpha) + \frac{1}{16\sqrt{15}} \delta U(x, \alpha) + \frac{73}{32\sqrt{15}} \delta U(x, \beta) \\
& - \frac{71}{64\sqrt{15}} \delta U(\alpha, \beta) + \frac{1}{8\sqrt{15}} \delta J(a, x) - \frac{1}{2\sqrt{15}} \delta J(x, y) + \frac{2}{\sqrt{15}} \delta J(\alpha, \beta) , \\
\delta S(a, \beta; \gamma, x) &= \frac{1}{\sqrt{15}} \delta U(\alpha) - \frac{1}{8\sqrt{15}} \delta U(a, \alpha) - \frac{1}{16\sqrt{15}} \delta U(x, \alpha) - \frac{73}{32\sqrt{15}} \delta U(x, \beta) \\
& + \frac{71}{64\sqrt{15}} \delta U(\alpha, \beta) - \frac{1}{8\sqrt{15}} \delta J(a, x) + \frac{1}{2\sqrt{15}} \delta J(x, y) - \frac{2}{\sqrt{15}} \delta J(\alpha, \beta) , \\
\delta S(x, y; \alpha, \beta) &= -\frac{1}{60} \delta U(\alpha) + \frac{1}{10} \delta U(x, \alpha) - \frac{1}{10} \delta U(x, \beta) + \frac{1}{60} \delta U(\alpha, \beta) \\
& - \frac{1}{18} \delta J(x, y) + \frac{1}{30} \delta J(\alpha, \beta) , \\
\delta S(x, y; \beta, \alpha) &= -\frac{2}{15} \delta U(\alpha) - \frac{3}{5} \delta U(x, \alpha) + \frac{3}{5} \delta U(x, \beta) + \frac{2}{15} \delta U(\alpha, \beta) \\
& - \frac{4}{9} \delta J(x, y) + \frac{4}{5} \delta J(\alpha, \beta) , \\
\delta S(x, z; \alpha, \gamma) &= \frac{1}{60} \delta U(\alpha) - \frac{1}{10} \delta U(x, \alpha) + \frac{1}{10} \delta U(x, \beta) - \frac{1}{60} \delta U(\alpha, \beta) \\
& + \frac{1}{18} \delta J(x, y) - \frac{1}{30} \delta J(\alpha, \beta) , \\
\delta S(x, z; \gamma, \alpha) &= \frac{2}{15} \delta U(\alpha) + \frac{3}{5} \delta U(x, \alpha) - \frac{3}{5} \delta U(x, \beta) - \frac{2}{15} \delta U(\alpha, \beta) \\
& + \frac{4}{9} \delta J(x, y) - \frac{4}{5} \delta J(\alpha, \beta) , \\
\delta S(x, \alpha; \beta, y) &= \frac{1}{20} \delta U(\alpha) + \frac{1}{2} \delta U(x, \alpha) - \frac{1}{2} \delta U(x, \beta) - \frac{1}{20} \delta U(\alpha, \beta) \\
& + \frac{1}{6} \delta J(x, y) - \frac{1}{10} \delta J(\alpha, \beta) , \\
\delta S(x, \alpha; \gamma, z) &= -\frac{1}{20} \delta U(\alpha) - \frac{1}{2} \delta U(x, \alpha) + \frac{1}{2} \delta U(x, \beta) + \frac{1}{20} \delta U(\alpha, \beta) \\
& - \frac{1}{6} \delta J(x, y) + \frac{1}{10} \delta J(\alpha, \beta) , \\
\delta S(y, z; \beta, \gamma) &= -\frac{1}{60} \delta U(\alpha) + \frac{1}{10} \delta U(x, \alpha) - \frac{1}{10} \delta U(x, \beta) + \frac{1}{60} \delta U(\alpha, \beta) \\
& - \frac{1}{18} \delta J(x, y) + \frac{1}{30} \delta J(\alpha, \beta) ,
\end{aligned}$$

$$\begin{aligned}
\delta S(y, z; \gamma, \beta) &= -\frac{2}{15}\delta U(\alpha) - \frac{3}{5}\delta U(x, \alpha) + \frac{3}{5}\delta U(x, \beta) + \frac{2}{15}\delta U(\alpha, \beta) \\
&\quad - \frac{4}{9}\delta J(x, y) + \frac{4}{5}\delta J(\alpha, \beta) , \\
\delta S(y, \beta; \gamma, z) &= \frac{1}{20}\delta U(\alpha) + \frac{1}{2}\delta U(x, \alpha) - \frac{1}{2}\delta U(x, \beta) - \frac{1}{20}\delta U(\alpha, \beta) \\
&\quad + \frac{1}{6}\delta J(x, y) - \frac{1}{10}\delta J(\alpha, \beta) .
\end{aligned}$$

## 2.6 $f$ -orbitals, group $T_h$

Independent parameter variations:

$$\delta U(\alpha), \delta U(a, \alpha), \delta U(x, \alpha), \delta U(x, \beta), \delta U(\alpha, \beta), \delta J(a, x), \delta J(x, y), \delta J(\alpha, \beta).$$

Dependent parameter variations:

$$\begin{aligned} \delta U(\beta) &= \delta U(\alpha) , \\ \delta U(\gamma) &= \delta U(\alpha) , \\ \delta U(a, \beta) &= \delta U(a, \alpha) , \\ \delta U(a, \gamma) &= \delta U(a, \alpha) , \\ \delta U(x, \gamma) &= \delta U(x, \beta) , \\ \delta U(y, \alpha) &= \delta U(x, \beta) , \\ \delta U(y, \beta) &= \delta U(x, \alpha) , \\ \delta U(y, \gamma) &= \delta U(x, \beta) , \\ \delta U(z, \alpha) &= \delta U(x, \beta) , \\ \delta U(z, \beta) &= \delta U(x, \beta) , \\ \delta U(z, \gamma) &= \delta U(x, \alpha) , \\ \delta U(\alpha, \gamma) &= \delta U(\alpha, \beta) , \\ \delta U(\beta, \gamma) &= \delta U(\alpha, \beta) , \\ \delta J(a, y) &= \delta J(a, x) , \\ \delta J(a, z) &= \delta J(a, x) , \\ \delta J(a, \alpha) &= \frac{1}{4}\delta U(\alpha) - \frac{1}{2}\delta U(a, \alpha) , \\ \delta J(a, \beta) &= \frac{1}{4}\delta U(\alpha) - \frac{1}{2}\delta U(a, \alpha) , \\ \delta J(a, \gamma) &= \frac{1}{4}\delta U(\alpha) - \frac{1}{2}\delta U(a, \alpha) , \\ \delta J(x, z) &= \delta J(x, y) , \\ \delta J(x, \alpha) &= -\frac{1}{60}\delta U(\alpha) - \frac{1}{2}\delta U(x, \alpha) + \frac{4}{5}\delta U(\alpha, \beta) - \frac{8}{15}\delta J(x, y) \\ &\quad + \frac{8}{15}\delta J(\alpha, \beta) , \\ \delta J(x, \beta) &= \frac{7}{30}\delta U(\alpha) - \frac{1}{2}\delta U(x, \beta) + \frac{1}{60}\delta U(\alpha, \beta) + \frac{3}{10}\delta J(x, y) \\ &\quad + \frac{1}{30}\delta J(\alpha, \beta) , \\ \delta J(x, \gamma) &= \frac{7}{30}\delta U(\alpha) - \frac{1}{2}\delta U(x, \beta) + \frac{1}{60}\delta U(\alpha, \beta) + \frac{3}{10}\delta J(x, y) \\ &\quad + \frac{1}{30}\delta J(\alpha, \beta) , \\ \delta J(y, z) &= \delta J(x, y) , \\ \delta J(y, \alpha) &= \frac{7}{30}\delta U(\alpha) - \frac{1}{2}\delta U(x, \beta) + \frac{1}{60}\delta U(\alpha, \beta) + \frac{3}{10}\delta J(x, y) \\ &\quad + \frac{1}{30}\delta J(\alpha, \beta) , \\ \delta J(y, \beta) &= -\frac{1}{60}\delta U(\alpha) - \frac{1}{2}\delta U(x, \alpha) + \frac{4}{5}\delta U(\alpha, \beta) - \frac{8}{15}\delta J(x, y) \\ &\quad + \frac{8}{15}\delta J(\alpha, \beta) , \\ \delta J(y, \gamma) &= \frac{7}{30}\delta U(\alpha) - \frac{1}{2}\delta U(x, \beta) + \frac{1}{60}\delta U(\alpha, \beta) + \frac{3}{10}\delta J(x, y) \end{aligned}$$

$$\begin{aligned}
& + \frac{1}{30} \delta J(\alpha, \beta) , \\
\delta J(z, \alpha) &= \frac{7}{30} \delta U(\alpha) - \frac{1}{2} \delta U(x, \beta) + \frac{1}{60} \delta U(\alpha, \beta) + \frac{3}{10} \delta J(x, y) \\
& + \frac{1}{30} \delta J(\alpha, \beta) , \\
\delta J(z, \beta) &= \frac{7}{30} \delta U(\alpha) - \frac{1}{2} \delta U(x, \beta) + \frac{1}{60} \delta U(\alpha, \beta) + \frac{3}{10} \delta J(x, y) \\
& + \frac{1}{30} \delta J(\alpha, \beta) , \\
\delta J(z, \gamma) &= -\frac{1}{60} \delta U(\alpha) - \frac{1}{2} \delta U(x, \alpha) + \frac{4}{5} \delta U(\alpha, \beta) - \frac{8}{15} \delta J(x, y) \\
& + \frac{8}{15} \delta J(\alpha, \beta) , \\
\delta J(\alpha, \gamma) &= \delta J(\alpha, \beta) , \\
\delta J(\beta, \gamma) &= \delta J(\alpha, \beta) , \\
\delta T(y; x, \alpha) &= \frac{2}{5\sqrt{15}} \delta U(\alpha) + \frac{9}{4} \sqrt{\frac{3}{5}} \delta U(x, \alpha) - \frac{3}{8} \sqrt{\frac{3}{5}} \delta U(x, \beta) - \frac{257}{80\sqrt{15}} \delta U(\alpha, \beta) \\
& + 2\sqrt{\frac{3}{5}} \delta J(x, y) - \frac{4}{5\sqrt{15}} \delta J(\alpha, \beta) , \\
\delta T(x; y, \beta) &= \frac{2}{5\sqrt{15}} \delta U(\alpha) + \frac{9}{4} \sqrt{\frac{3}{5}} \delta U(x, \alpha) - \frac{3}{8} \sqrt{\frac{3}{5}} \delta U(x, \beta) - \frac{257}{80\sqrt{15}} \delta U(\alpha, \beta) \\
& + 2\sqrt{\frac{3}{5}} \delta J(x, y) - \frac{4}{5\sqrt{15}} \delta J(\alpha, \beta) , \\
\delta T(z; x, \alpha) &= -\frac{2}{5\sqrt{15}} \delta U(\alpha) - \frac{9}{4} \sqrt{\frac{3}{5}} \delta U(x, \alpha) + \frac{3}{8} \sqrt{\frac{3}{5}} \delta U(x, \beta) + \frac{257}{80\sqrt{15}} \delta U(\alpha, \beta) \\
& - 2\sqrt{\frac{3}{5}} \delta J(x, y) + \frac{4}{5\sqrt{15}} \delta J(\alpha, \beta) , \\
\delta T(x; z, \gamma) &= \frac{2}{5\sqrt{15}} \delta U(\alpha) + \frac{9}{4} \sqrt{\frac{3}{5}} \delta U(x, \alpha) - \frac{3}{8} \sqrt{\frac{3}{5}} \delta U(x, \beta) - \frac{257}{80\sqrt{15}} \delta U(\alpha, \beta) \\
& + 2\sqrt{\frac{3}{5}} \delta J(x, y) - \frac{4}{5\sqrt{15}} \delta J(\alpha, \beta) , \\
\delta T(\beta; x, \alpha) &= -\frac{1}{4\sqrt{15}} \delta U(x, \alpha) - \frac{13}{8\sqrt{15}} \delta U(x, \beta) + \frac{1}{9} \sqrt{\frac{5}{3}} \delta U(\alpha, \beta) - \frac{2}{3\sqrt{15}} \delta J(x, y) , \\
\delta T(\gamma; x, \alpha) &= \frac{1}{4\sqrt{15}} \delta U(x, \alpha) + \frac{13}{8\sqrt{15}} \delta U(x, \beta) - \frac{1}{9} \sqrt{\frac{5}{3}} \delta U(\alpha, \beta) + \frac{2}{3\sqrt{15}} \delta J(x, y) , \\
\delta T(z; y, \beta) &= -\frac{2}{5\sqrt{15}} \delta U(\alpha) - \frac{9}{4} \sqrt{\frac{3}{5}} \delta U(x, \alpha) + \frac{3}{8} \sqrt{\frac{3}{5}} \delta U(x, \beta) + \frac{257}{80\sqrt{15}} \delta U(\alpha, \beta) \\
& - 2\sqrt{\frac{3}{5}} \delta J(x, y) + \frac{4}{5\sqrt{15}} \delta J(\alpha, \beta) , \\
\delta T(y; z, \gamma) &= -\frac{2}{5\sqrt{15}} \delta U(\alpha) - \frac{9}{4} \sqrt{\frac{3}{5}} \delta U(x, \alpha) + \frac{3}{8} \sqrt{\frac{3}{5}} \delta U(x, \beta) + \frac{257}{80\sqrt{15}} \delta U(\alpha, \beta) \\
& - 2\sqrt{\frac{3}{5}} \delta J(x, y) + \frac{4}{5\sqrt{15}} \delta J(\alpha, \beta) , \\
\delta T(\alpha; y, \beta) &= -\frac{1}{4\sqrt{15}} \delta U(x, \alpha) - \frac{13}{8\sqrt{15}} \delta U(x, \beta) + \frac{1}{9} \sqrt{\frac{5}{3}} \delta U(\alpha, \beta) - \frac{2}{3\sqrt{15}} \delta J(x, y) , \\
\delta T(\gamma; y, \beta) &= \frac{1}{4\sqrt{15}} \delta U(x, \alpha) + \frac{13}{8\sqrt{15}} \delta U(x, \beta) - \frac{1}{9} \sqrt{\frac{5}{3}} \delta U(\alpha, \beta) + \frac{2}{3\sqrt{15}} \delta J(x, y) ,
\end{aligned}$$



$$\begin{aligned}
\delta T(\alpha; z, \gamma) &= -\frac{1}{4\sqrt{15}}\delta U(x, \alpha) - \frac{13}{8\sqrt{15}}\delta U(x, \beta) + \frac{1}{9}\sqrt{\frac{5}{3}}\delta U(\alpha, \beta) - \frac{2}{3\sqrt{15}}\delta J(x, y) , \\
\delta T(\beta; z, \gamma) &= \frac{1}{4\sqrt{15}}\delta U(x, \alpha) + \frac{13}{8\sqrt{15}}\delta U(x, \beta) - \frac{1}{9}\sqrt{\frac{5}{3}}\delta U(\alpha, \beta) + \frac{2}{3\sqrt{15}}\delta J(x, y) , \\
\delta A(x; x, \beta) &= \frac{1}{40\sqrt{15}}\delta U(\alpha) - \frac{9}{8}\sqrt{\frac{3}{5}}\delta U(x, \alpha) + \frac{3}{16}\sqrt{\frac{3}{5}}\delta U(x, \beta) + \frac{221}{800}\sqrt{\frac{3}{5}}\delta U(\alpha, \beta) \\
&\quad - \frac{1}{4}\sqrt{\frac{3}{5}}\delta J(x, y) - \frac{1}{20\sqrt{15}}\delta J(\alpha, \beta) , \\
\delta A(x; x, \gamma) &= \frac{1}{40\sqrt{15}}\delta U(\alpha) - \frac{9}{8}\sqrt{\frac{3}{5}}\delta U(x, \alpha) + \frac{3}{16}\sqrt{\frac{3}{5}}\delta U(x, \beta) + \frac{221}{800}\sqrt{\frac{3}{5}}\delta U(\alpha, \beta) \\
&\quad - \frac{1}{4}\sqrt{\frac{3}{5}}\delta J(x, y) - \frac{1}{20\sqrt{15}}\delta J(\alpha, \beta) , \\
\delta A(y; x, \alpha) &= \frac{1}{40\sqrt{15}}\delta U(\alpha) - \frac{9}{8}\sqrt{\frac{3}{5}}\delta U(x, \alpha) + \frac{3}{16}\sqrt{\frac{3}{5}}\delta U(x, \beta) + \frac{221}{800}\sqrt{\frac{3}{5}}\delta U(\alpha, \beta) \\
&\quad - \frac{1}{4}\sqrt{\frac{3}{5}}\delta J(x, y) - \frac{1}{20\sqrt{15}}\delta J(\alpha, \beta) , \\
\delta A(z; x, \alpha) &= -\frac{1}{40\sqrt{15}}\delta U(\alpha) + \frac{9}{8}\sqrt{\frac{3}{5}}\delta U(x, \alpha) - \frac{3}{16}\sqrt{\frac{3}{5}}\delta U(x, \beta) - \frac{221}{800}\sqrt{\frac{3}{5}}\delta U(\alpha, \beta) \\
&\quad + \frac{1}{4}\sqrt{\frac{3}{5}}\delta J(x, y) + \frac{1}{20\sqrt{15}}\delta J(\alpha, \beta) , \\
\delta A(\beta; x, \alpha) &= -\frac{1}{8}\sqrt{\frac{3}{5}}\delta U(\alpha) + \frac{1}{8\sqrt{15}}\delta U(x, \alpha) + \frac{13}{16\sqrt{15}}\delta U(x, \beta) - \frac{1}{32}\sqrt{\frac{3}{5}}\delta U(\alpha, \beta) \\
&\quad - \frac{1}{12\sqrt{15}}\delta J(x, y) + \frac{1}{4}\sqrt{\frac{3}{5}}\delta J(\alpha, \beta) , \\
\delta A(\gamma; x, \alpha) &= \frac{1}{8}\sqrt{\frac{3}{5}}\delta U(\alpha) - \frac{1}{8\sqrt{15}}\delta U(x, \alpha) - \frac{13}{16\sqrt{15}}\delta U(x, \beta) + \frac{1}{32}\sqrt{\frac{3}{5}}\delta U(\alpha, \beta) \\
&\quad + \frac{1}{12\sqrt{15}}\delta J(x, y) - \frac{1}{4}\sqrt{\frac{3}{5}}\delta J(\alpha, \beta) , \\
\delta A(y; y, \gamma) &= -\frac{1}{40\sqrt{15}}\delta U(\alpha) + \frac{9}{8}\sqrt{\frac{3}{5}}\delta U(x, \alpha) - \frac{3}{16}\sqrt{\frac{3}{5}}\delta U(x, \beta) - \frac{221}{800}\sqrt{\frac{3}{5}}\delta U(\alpha, \beta) \\
&\quad + \frac{1}{4}\sqrt{\frac{3}{5}}\delta J(x, y) + \frac{1}{20\sqrt{15}}\delta J(\alpha, \beta) , \\
\delta A(z; y, \beta) &= -\frac{1}{40\sqrt{15}}\delta U(\alpha) + \frac{9}{8}\sqrt{\frac{3}{5}}\delta U(x, \alpha) - \frac{3}{16}\sqrt{\frac{3}{5}}\delta U(x, \beta) - \frac{221}{800}\sqrt{\frac{3}{5}}\delta U(\alpha, \beta) \\
&\quad + \frac{1}{4}\sqrt{\frac{3}{5}}\delta J(x, y) + \frac{1}{20\sqrt{15}}\delta J(\alpha, \beta) , \\
\delta A(\alpha; y, \beta) &= -\frac{1}{8}\sqrt{\frac{3}{5}}\delta U(\alpha) + \frac{1}{8\sqrt{15}}\delta U(x, \alpha) + \frac{13}{16\sqrt{15}}\delta U(x, \beta) - \frac{1}{32}\sqrt{\frac{3}{5}}\delta U(\alpha, \beta) \\
&\quad - \frac{1}{12\sqrt{15}}\delta J(x, y) + \frac{1}{4}\sqrt{\frac{3}{5}}\delta J(\alpha, \beta) , \\
\delta A(\gamma; y, \beta) &= \frac{1}{8}\sqrt{\frac{3}{5}}\delta U(\alpha) - \frac{1}{8\sqrt{15}}\delta U(x, \alpha) - \frac{13}{16\sqrt{15}}\delta U(x, \beta) + \frac{1}{32}\sqrt{\frac{3}{5}}\delta U(\alpha, \beta) \\
&\quad + \frac{1}{12\sqrt{15}}\delta J(x, y) - \frac{1}{4}\sqrt{\frac{3}{5}}\delta J(\alpha, \beta) ,
\end{aligned}$$

$$\begin{aligned}
\delta A(\alpha; z, \gamma) &= -\frac{1}{8}\sqrt{\frac{3}{5}}\delta U(\alpha) + \frac{1}{8\sqrt{15}}\delta U(x, \alpha) + \frac{13}{16\sqrt{15}}\delta U(x, \beta) - \frac{1}{32}\sqrt{\frac{3}{5}}\delta U(\alpha, \beta) \\
&\quad - \frac{1}{12\sqrt{15}}\delta J(x, y) + \frac{1}{4}\sqrt{\frac{3}{5}}\delta J(\alpha, \beta) , \\
\delta A(\beta; z, \gamma) &= \frac{1}{8}\sqrt{\frac{3}{5}}\delta U(\alpha) - \frac{1}{8\sqrt{15}}\delta U(x, \alpha) - \frac{13}{16\sqrt{15}}\delta U(x, \beta) + \frac{1}{32}\sqrt{\frac{3}{5}}\delta U(\alpha, \beta) \\
&\quad + \frac{1}{12\sqrt{15}}\delta J(x, y) - \frac{1}{4}\sqrt{\frac{3}{5}}\delta J(\alpha, \beta) , \\
\delta S(a, x; y, z) &= \frac{1}{8}\sqrt{\frac{3}{5}}\delta J(a, x) - \frac{4}{5\sqrt{15}}\delta J(x, y) , \\
\delta S(a, x; z, y) &= \frac{1}{8}\sqrt{\frac{3}{5}}\delta J(a, x) - \frac{4}{5\sqrt{15}}\delta J(x, y) , \\
\delta S(a, x; \beta, z) &= \frac{1}{30}\delta U(\alpha) - \frac{3}{16}\delta U(a, \alpha) + \frac{79}{160}\delta U(x, \alpha) + \frac{7}{320}\delta U(x, \beta) \\
&\quad - \frac{379}{1920}\delta U(\alpha, \beta) - \frac{1}{8}\delta J(a, x) + \frac{73}{180}\delta J(x, y) - \frac{1}{15}\delta J(\alpha, \beta) , \\
\delta S(a, x; \beta, \gamma) &= \frac{1}{9}\sqrt{\frac{5}{3}}\delta U(a, \alpha) + \frac{1}{32\sqrt{15}}\delta U(x, \alpha) + \frac{73}{64\sqrt{15}}\delta U(x, \beta) - \frac{9\sqrt{15}}{128}\delta U(\alpha, \beta) \\
&\quad + \frac{1}{12\sqrt{15}}\delta J(x, y) , \\
\delta S(a, x; \gamma, y) &= \frac{1}{30}\delta U(\alpha) - \frac{3}{16}\delta U(a, \alpha) + \frac{79}{160}\delta U(x, \alpha) + \frac{7}{320}\delta U(x, \beta) \\
&\quad - \frac{379}{1920}\delta U(\alpha, \beta) - \frac{1}{8}\delta J(a, x) + \frac{73}{180}\delta J(x, y) - \frac{1}{15}\delta J(\alpha, \beta) , \\
\delta S(a, x; \gamma, \beta) &= \frac{1}{9}\sqrt{\frac{5}{3}}\delta U(a, \alpha) + \frac{1}{32\sqrt{15}}\delta U(x, \alpha) + \frac{73}{64\sqrt{15}}\delta U(x, \beta) - \frac{9\sqrt{15}}{128}\delta U(\alpha, \beta) \\
&\quad + \frac{1}{12\sqrt{15}}\delta J(x, y) , \\
\delta S(a, y; z, x) &= \frac{1}{8}\sqrt{\frac{3}{5}}\delta J(a, x) - \frac{4}{5\sqrt{15}}\delta J(x, y) , \\
\delta S(a, y; \alpha, z) &= \frac{1}{30}\delta U(\alpha) - \frac{3}{16}\delta U(a, \alpha) + \frac{79}{160}\delta U(x, \alpha) + \frac{7}{320}\delta U(x, \beta) \\
&\quad - \frac{379}{1920}\delta U(\alpha, \beta) - \frac{1}{8}\delta J(a, x) + \frac{73}{180}\delta J(x, y) - \frac{1}{15}\delta J(\alpha, \beta) , \\
\delta S(a, y; \alpha, \gamma) &= -\frac{1}{9}\sqrt{\frac{5}{3}}\delta U(a, \alpha) - \frac{1}{32\sqrt{15}}\delta U(x, \alpha) - \frac{73}{64\sqrt{15}}\delta U(x, \beta) + \frac{9\sqrt{15}}{128}\delta U(\alpha, \beta) \\
&\quad - \frac{1}{12\sqrt{15}}\delta J(x, y) , \\
\delta S(a, y; \gamma, x) &= -\frac{1}{30}\delta U(\alpha) + \frac{3}{16}\delta U(a, \alpha) - \frac{79}{160}\delta U(x, \alpha) - \frac{7}{320}\delta U(x, \beta) \\
&\quad + \frac{379}{1920}\delta U(\alpha, \beta) + \frac{1}{8}\delta J(a, x) - \frac{73}{180}\delta J(x, y) + \frac{1}{15}\delta J(\alpha, \beta) , \\
\delta S(a, y; \gamma, \alpha) &= -\frac{1}{9}\sqrt{\frac{5}{3}}\delta U(a, \alpha) - \frac{1}{32\sqrt{15}}\delta U(x, \alpha) - \frac{73}{64\sqrt{15}}\delta U(x, \beta) + \frac{9\sqrt{15}}{128}\delta U(\alpha, \beta) \\
&\quad - \frac{1}{12\sqrt{15}}\delta J(x, y) , \\
\delta S(a, z; \alpha, y) &= -\frac{1}{30}\delta U(\alpha) + \frac{3}{16}\delta U(a, \alpha) - \frac{79}{160}\delta U(x, \alpha) - \frac{7}{320}\delta U(x, \beta) \\
&\quad + \frac{379}{1920}\delta U(\alpha, \beta) + \frac{1}{8}\delta J(a, x) - \frac{73}{180}\delta J(x, y) + \frac{1}{15}\delta J(\alpha, \beta) ,
\end{aligned}$$

$$\begin{aligned}
\delta S(a, z; \alpha, \beta) &= \frac{1}{9} \sqrt{\frac{5}{3}} \delta U(a, \alpha) + \frac{1}{32\sqrt{15}} \delta U(x, \alpha) + \frac{73}{64\sqrt{15}} \delta U(x, \beta) - \frac{9\sqrt{15}}{128} \delta U(\alpha, \beta) \\
&\quad + \frac{1}{12\sqrt{15}} \delta J(x, y) , \\
\delta S(a, z; \beta, x) &= -\frac{1}{30} \delta U(\alpha) + \frac{3}{16} \delta U(a, \alpha) - \frac{79}{160} \delta U(x, \alpha) - \frac{7}{320} \delta U(x, \beta) \\
&\quad + \frac{379}{1920} \delta U(\alpha, \beta) + \frac{1}{8} \delta J(a, x) - \frac{73}{180} \delta J(x, y) + \frac{1}{15} \delta J(\alpha, \beta) , \\
\delta S(a, z; \beta, \alpha) &= \frac{1}{9} \sqrt{\frac{5}{3}} \delta U(a, \alpha) + \frac{1}{32\sqrt{15}} \delta U(x, \alpha) + \frac{73}{64\sqrt{15}} \delta U(x, \beta) - \frac{9\sqrt{15}}{128} \delta U(\alpha, \beta) \\
&\quad + \frac{1}{12\sqrt{15}} \delta J(x, y) , \\
\delta S(a, \alpha; \beta, z) &= \frac{1}{\sqrt{15}} \delta U(\alpha) - \frac{1}{8\sqrt{15}} \delta U(a, \alpha) - \frac{1}{16\sqrt{15}} \delta U(x, \alpha) - \frac{73}{32\sqrt{15}} \delta U(x, \beta) \\
&\quad + \frac{71}{64\sqrt{15}} \delta U(\alpha, \beta) - \frac{1}{8\sqrt{15}} \delta J(a, x) + \frac{1}{2\sqrt{15}} \delta J(x, y) - \frac{2}{\sqrt{15}} \delta J(\alpha, \beta) , \\
\delta S(a, \alpha; \gamma, y) &= -\frac{1}{\sqrt{15}} \delta U(\alpha) + \frac{1}{8\sqrt{15}} \delta U(a, \alpha) + \frac{1}{16\sqrt{15}} \delta U(x, \alpha) + \frac{73}{32\sqrt{15}} \delta U(x, \beta) \\
&\quad - \frac{71}{64\sqrt{15}} \delta U(\alpha, \beta) + \frac{1}{8\sqrt{15}} \delta J(a, x) - \frac{1}{2\sqrt{15}} \delta J(x, y) + \frac{2}{\sqrt{15}} \delta J(\alpha, \beta) , \\
\delta S(a, \beta; \gamma, x) &= \frac{1}{\sqrt{15}} \delta U(\alpha) - \frac{1}{8\sqrt{15}} \delta U(a, \alpha) - \frac{1}{16\sqrt{15}} \delta U(x, \alpha) - \frac{73}{32\sqrt{15}} \delta U(x, \beta) \\
&\quad + \frac{71}{64\sqrt{15}} \delta U(\alpha, \beta) - \frac{1}{8\sqrt{15}} \delta J(a, x) + \frac{1}{2\sqrt{15}} \delta J(x, y) - \frac{2}{\sqrt{15}} \delta J(\alpha, \beta) , \\
\delta S(x, y; \alpha, \beta) &= -\frac{1}{60} \delta U(\alpha) + \frac{1}{10} \delta U(x, \alpha) - \frac{1}{10} \delta U(x, \beta) + \frac{1}{60} \delta U(\alpha, \beta) \\
&\quad - \frac{1}{18} \delta J(x, y) + \frac{1}{30} \delta J(\alpha, \beta) , \\
\delta S(x, y; \beta, \alpha) &= -\frac{2}{15} \delta U(\alpha) - \frac{3}{5} \delta U(x, \alpha) + \frac{3}{5} \delta U(x, \beta) + \frac{2}{15} \delta U(\alpha, \beta) \\
&\quad - \frac{4}{9} \delta J(x, y) + \frac{4}{5} \delta J(\alpha, \beta) , \\
\delta S(x, z; \alpha, \gamma) &= \frac{1}{60} \delta U(\alpha) - \frac{1}{10} \delta U(x, \alpha) + \frac{1}{10} \delta U(x, \beta) - \frac{1}{60} \delta U(\alpha, \beta) \\
&\quad + \frac{1}{18} \delta J(x, y) - \frac{1}{30} \delta J(\alpha, \beta) , \\
\delta S(x, z; \gamma, \alpha) &= \frac{2}{15} \delta U(\alpha) + \frac{3}{5} \delta U(x, \alpha) - \frac{3}{5} \delta U(x, \beta) - \frac{2}{15} \delta U(\alpha, \beta) \\
&\quad + \frac{4}{9} \delta J(x, y) - \frac{4}{5} \delta J(\alpha, \beta) , \\
\delta S(x, \alpha; \beta, y) &= \frac{1}{20} \delta U(\alpha) + \frac{1}{2} \delta U(x, \alpha) - \frac{1}{2} \delta U(x, \beta) - \frac{1}{20} \delta U(\alpha, \beta) \\
&\quad + \frac{1}{6} \delta J(x, y) - \frac{1}{10} \delta J(\alpha, \beta) , \\
\delta S(x, \alpha; \gamma, z) &= -\frac{1}{20} \delta U(\alpha) - \frac{1}{2} \delta U(x, \alpha) + \frac{1}{2} \delta U(x, \beta) + \frac{1}{20} \delta U(\alpha, \beta) \\
&\quad - \frac{1}{6} \delta J(x, y) + \frac{1}{10} \delta J(\alpha, \beta) , \\
\delta S(y, z; \beta, \gamma) &= -\frac{1}{60} \delta U(\alpha) + \frac{1}{10} \delta U(x, \alpha) - \frac{1}{10} \delta U(x, \beta) + \frac{1}{60} \delta U(\alpha, \beta) \\
&\quad - \frac{1}{18} \delta J(x, y) + \frac{1}{30} \delta J(\alpha, \beta) , \\
\delta S(y, z; \gamma, \beta) &= -\frac{2}{15} \delta U(\alpha) - \frac{3}{5} \delta U(x, \alpha) + \frac{3}{5} \delta U(x, \beta) + \frac{2}{15} \delta U(\alpha, \beta)
\end{aligned}$$

$$\begin{aligned}
& -\frac{4}{9}\delta J(x, y) + \frac{4}{5}\delta J(\alpha, \beta) , \\
\delta S(y, \beta; \gamma, z) = & \frac{1}{20}\delta U(\alpha) + \frac{1}{2}\delta U(x, \alpha) - \frac{1}{2}\delta U(x, \beta) - \frac{1}{20}\delta U(\alpha, \beta) \\
& + \frac{1}{6}\delta J(x, y) - \frac{1}{10}\delta J(\alpha, \beta) .
\end{aligned}$$

## 2.7 $f$ -orbitals, group $D_{6h}$

Independent parameter variations:

$$\begin{aligned} &\delta U(z), \delta U(\alpha'), \delta U(\beta'), \delta U(x', y'), \delta U(x', z), \delta U(a, \alpha'), \delta U(x', \alpha'), \delta U(a, \beta'), \delta U(a, \gamma), \\ &\delta U(x', \beta'), \delta U(z, \alpha'), \delta U(\alpha', \beta'), \delta J(x', \alpha'), \delta J(a, x'), \delta J(a, \alpha'), \delta J(a, z). \end{aligned}$$

Dependent parameter variations:

$$\begin{aligned} \delta U(y', z) &= \delta U(x', z), \\ \delta U(y', \alpha') &= \delta U(x', \alpha'), \\ \delta U(y', \beta') &= \delta U(x', \beta'), \\ \delta U(z, \beta') &= \frac{1}{6}\delta U(z) - \frac{73}{150}\delta U(\alpha') - \frac{8}{15}\delta J(x', \alpha') - \frac{7}{6}\delta U(x', y') \\ &\quad + \frac{16}{25}\delta U(a, \alpha') - \frac{11}{30}\delta U(x', \alpha') - \frac{3}{5}\delta U(a, \beta') - \frac{1}{15}\delta U(a, \gamma) \\ &\quad + \frac{3}{2}\delta U(x', \beta') + \frac{3}{5}\delta U(z, \alpha') + \frac{1}{10}\delta U(\alpha', \beta') - \frac{106}{45}\delta J(a, x') \\ &\quad + \frac{62}{25}\delta J(a, \alpha') - \frac{2}{3}\delta J(a, z), \\ \delta U(\alpha', \gamma) &= \delta U(a, \alpha'), \\ \delta U(\beta', \gamma) &= \delta U(a, \beta'), \\ \delta J(a, y') &= \delta J(a, x'), \\ \delta J(a, \alpha') &= \delta J(a, \alpha'), \\ \delta J(a, \beta') &= -\frac{1}{4}\delta U(\alpha') + \frac{1}{4}\delta U(\beta') + \frac{1}{2}\delta U(a, \alpha') - \frac{1}{2}\delta U(a, \beta') \\ &\quad + \delta J(a, \alpha'), \\ \delta J(a, \gamma) &= -\frac{1}{2}\delta U(a, \gamma), \\ \delta J(x', y') &= -\frac{1}{2}\delta U(x', y'), \\ \delta J(x', z) &= \frac{1}{4}\delta U(z) + \frac{1}{8}\delta U(\alpha') - \frac{1}{2}\delta U(x', z) - \frac{1}{4}\delta U(a, \alpha') \\ &\quad + \frac{5}{6}\delta J(a, x') - \frac{1}{2}\delta J(a, \alpha'), \\ \delta J(x', \beta') &= \frac{1}{2}\delta U(z) - \frac{171}{100}\delta U(\alpha') + \frac{1}{4}\delta U(\beta') - \frac{3}{5}\delta J(x', \alpha') \\ &\quad - \frac{7}{2}\delta U(x', y') + \frac{48}{25}\delta U(a, \alpha') + \frac{12}{5}\delta U(x', \alpha') - \frac{9}{5}\delta U(a, \beta') \\ &\quad - \frac{2}{10}\delta U(a, \gamma) + \delta U(x', \beta') - \frac{6}{5}\delta U(z, \alpha') + \frac{3}{10}\delta U(\alpha', \beta') \\ &\quad - \frac{106}{15}\delta J(a, x') + \frac{186}{25}\delta J(a, \alpha') - 2\delta J(a, z), \\ \delta J(x', \gamma) &= \delta J(a, x'), \\ \delta J(y', z) &= \frac{1}{4}\delta U(z) + \frac{1}{8}\delta U(\alpha') - \frac{1}{2}\delta U(x', z) - \frac{1}{4}\delta U(a, \alpha') \\ &\quad + \frac{5}{6}\delta J(a, x') - \frac{1}{2}\delta J(a, \alpha'), \\ \delta J(y', \alpha') &= \delta J(x', \alpha'), \\ \delta J(y', \beta') &= \frac{1}{2}\delta U(z) - \frac{171}{100}\delta U(\alpha') + \frac{1}{4}\delta U(\beta') - \frac{3}{5}\delta J(x', \alpha') \\ &\quad - \frac{7}{2}\delta U(x', y') + \frac{48}{25}\delta U(a, \alpha') + \frac{12}{5}\delta U(x', \alpha') - \frac{9}{5}\delta U(a, \beta') \\ &\quad - \frac{2}{10}\delta U(a, \gamma) + \delta U(x', \beta') - \frac{6}{5}\delta U(z, \alpha') + \frac{3}{10}\delta U(\alpha', \beta') \end{aligned}$$

$$\begin{aligned}
& -\frac{106}{15}\delta J(a, x') + \frac{186}{25}\delta J(a, \alpha') - 2\delta J(a, z) , \\
\delta J(y', \gamma) &= \delta J(a, x') , \\
\delta J(z, \alpha') &= \frac{5}{8}\delta U(z) - \frac{17}{10}\delta U(\alpha') + \frac{3}{2}\delta J(x', \alpha') + \frac{63}{20}\delta U(a, \alpha') \\
&+ \frac{3}{4}\delta U(x', \alpha') - \frac{1}{2}\delta U(z, \alpha') - \frac{13}{2}\delta J(a, x') + \frac{63}{10}\delta J(a, \alpha') \\
&- \frac{3}{2}\delta J(a, z) , \\
\delta J(z, \beta') &= \frac{31}{24}\delta U(z) - \frac{1169}{300}\delta U(\alpha') + \frac{1}{4}\delta U(\beta') - \frac{19}{30}\delta J(x', \alpha') \\
&- \frac{14}{3}\delta U(x', y') + \frac{571}{100}\delta U(a, \alpha') + \frac{227}{60}\delta U(x', \alpha') - \frac{12}{5}\delta U(a, \beta') \\
&- \frac{4}{5}\delta U(a, \gamma) + \frac{3}{2}\delta U(x', \beta') - \frac{21}{10}\delta U(z, \alpha') + \frac{2}{5}\delta U(\alpha', \beta') \\
&- \frac{1433}{90}\delta J(a, x') + \frac{811}{50}\delta J(a, \alpha') - \frac{25}{6}\delta J(a, z) , \\
\delta J(z, \gamma) &= \delta J(a, z) , \\
\delta J(\alpha', \beta') &= \frac{1}{4}\delta U(\alpha') + \frac{1}{4}\delta U(\beta') - \frac{1}{2}\delta U(\alpha', \beta') , \\
\delta J(\alpha', \gamma) &= \delta J(a, \alpha') , \\
\delta J(\beta', \gamma) &= -\frac{1}{4}\delta U(\alpha') + \frac{1}{4}\delta U(\beta') + \frac{1}{2}\delta U(a, \alpha') - \frac{1}{2}\delta U(a, \beta') \\
&+ \delta J(a, \alpha') , \\
\delta T(a; x', \alpha') &= -\frac{\sqrt{\frac{5}{3}}}{4}\delta U(z) + \frac{151}{40\sqrt{15}}\delta U(\alpha') + 2\sqrt{\frac{3}{5}}\delta J(x', \alpha') + \frac{2}{3}\sqrt{\frac{5}{3}}\delta U(x', y') \\
&- \frac{29}{5\sqrt{15}}\delta U(a, \alpha') - \frac{19}{4\sqrt{15}}\delta U(x', \alpha') + \frac{1}{6}\sqrt{\frac{5}{3}}\delta U(a, \gamma) + \sqrt{\frac{3}{5}}\delta U(z, \alpha') \\
&+ \frac{43}{3\sqrt{15}}\delta J(a, x') - \frac{83}{5\sqrt{15}}\delta J(a, \alpha') + \sqrt{\frac{5}{3}}\delta J(a, z) , \\
\delta T(a; y', \beta') &= -\frac{1}{8\sqrt{15}}\delta U(\alpha') + \frac{1}{2}\sqrt{\frac{5}{3}}\delta J(x', \alpha') + \frac{13\sqrt{\frac{5}{3}}}{12}\delta U(x', y') + \frac{7}{2\sqrt{15}}\delta U(a, \alpha') \\
&- \frac{1}{2}\sqrt{\frac{5}{3}}\delta U(x', \alpha') + \frac{2}{\sqrt{15}}\delta U(a, \beta') - \frac{1}{3\sqrt{15}}\delta U(a, \gamma) - \frac{\sqrt{\frac{5}{3}}}{4}\delta U(x', \beta') \\
&- \frac{1}{4}\sqrt{\frac{3}{5}}\delta U(\alpha', \beta') + \frac{2}{3}\sqrt{\frac{5}{3}}\delta J(a, x') - \frac{2}{\sqrt{15}}\delta J(a, \alpha') , \\
\delta T(y'; x', \alpha') &= -\frac{9\sqrt{\frac{3}{5}}}{20}\delta U(\alpha') - \frac{1}{\sqrt{15}}\delta J(x', \alpha') + \frac{16}{5\sqrt{15}}\delta U(a, \alpha') - \frac{1}{2\sqrt{15}}\delta U(x', \alpha') \\
&- \frac{32}{3\sqrt{15}}\delta J(a, x') + \frac{32}{5\sqrt{15}}\delta J(a, \alpha') , \\
\delta T(x'; y', \beta') &= \frac{1}{2\sqrt{15}}\delta U(z) - \frac{11}{100\sqrt{15}}\delta U(\alpha') - \frac{\sqrt{\frac{3}{5}}}{5}\delta J(x', \alpha') - \frac{7}{2\sqrt{15}}\delta U(x', y') \\
&- \frac{32}{25\sqrt{15}}\delta U(a, \alpha') + \frac{4\sqrt{\frac{3}{5}}}{5}\delta U(x', \alpha') - \frac{3\sqrt{\frac{3}{5}}}{5}\delta U(a, \beta') - \frac{1}{5\sqrt{15}}\delta U(a, \gamma) \\
&+ 2\sqrt{\frac{3}{5}}\delta U(x', \beta') - \frac{2\sqrt{\frac{3}{5}}}{5}\delta U(z, \alpha') + \frac{\sqrt{\frac{3}{5}}}{10}\delta U(\alpha', \beta') + \frac{6\sqrt{\frac{3}{5}}}{5}\delta J(a, x')
\end{aligned}$$

$$\begin{aligned}
& + \frac{26}{25\sqrt{15}}\delta J(a, \alpha') - \frac{2}{\sqrt{15}}\delta J(a, z) , \\
\delta T(x'; z, \gamma) &= \frac{\sqrt{\frac{5}{3}}}{4}\delta U(z) - \frac{161}{80\sqrt{15}}\delta U(\alpha') + \frac{1}{4}\sqrt{\frac{3}{5}}\delta J(x', \alpha') + \frac{1}{3}\sqrt{\frac{5}{3}}\delta U(x', y') \\
& - \frac{\sqrt{\frac{5}{3}}}{4}\delta U(x', z) + \frac{73}{20\sqrt{15}}\delta U(a, \alpha') + \frac{7\sqrt{\frac{3}{5}}}{8}\delta U(x', \alpha') + \frac{\sqrt{\frac{5}{3}}}{12}\delta U(a, \gamma) \\
& - \frac{3}{4}\sqrt{\frac{3}{5}}\delta U(z, \alpha') - \frac{17}{6\sqrt{15}}\delta J(a, x') + \frac{73}{10\sqrt{15}}\delta J(a, \alpha') - \sqrt{\frac{5}{3}}\delta J(a, z) , \\
\delta T(\gamma; x', \alpha') &= \frac{\sqrt{\frac{5}{3}}}{4}\delta U(z) - \frac{151}{40\sqrt{15}}\delta U(\alpha') - 2\sqrt{\frac{3}{5}}\delta J(x', \alpha') - \frac{2}{3}\sqrt{\frac{5}{3}}\delta U(x', y') \\
& + \frac{29}{5\sqrt{15}}\delta U(a, \alpha') + \frac{19}{4\sqrt{15}}\delta U(x', \alpha') - \frac{1}{6}\sqrt{\frac{5}{3}}\delta U(a, \gamma) - \sqrt{\frac{3}{5}}\delta U(z, \alpha') \\
& - \frac{43}{3\sqrt{15}}\delta J(a, x') + \frac{83}{5\sqrt{15}}\delta J(a, \alpha') - \sqrt{\frac{5}{3}}\delta J(a, z) , \\
\delta T(y'; z, \gamma) &= -\frac{\sqrt{\frac{5}{3}}}{4}\delta U(z) + \frac{161}{80\sqrt{15}}\delta U(\alpha') - \frac{1}{4}\sqrt{\frac{3}{5}}\delta J(x', \alpha') - \frac{1}{3}\sqrt{\frac{5}{3}}\delta U(x', y') \\
& + \frac{\sqrt{\frac{5}{3}}}{4}\delta U(x', z) - \frac{73}{20\sqrt{15}}\delta U(a, \alpha') - \frac{7\sqrt{\frac{3}{5}}}{8}\delta U(x', \alpha') - \frac{\sqrt{\frac{5}{3}}}{12}\delta U(a, \gamma) \\
& + \frac{3}{4}\sqrt{\frac{3}{5}}\delta U(z, \alpha') + \frac{17}{6\sqrt{15}}\delta J(a, x') - \frac{73}{10\sqrt{15}}\delta J(a, \alpha') + \sqrt{\frac{5}{3}}\delta J(a, z) , \\
\delta T(\gamma; y', \beta') &= \frac{1}{8\sqrt{15}}\delta U(\alpha') - \frac{1}{2}\sqrt{\frac{5}{3}}\delta J(x', \alpha') - \frac{13\sqrt{\frac{5}{3}}}{12}\delta U(x', y') - \frac{7}{2\sqrt{15}}\delta U(a, \alpha') \\
& + \frac{1}{2}\sqrt{\frac{5}{3}}\delta U(x', \alpha') - \frac{2}{\sqrt{15}}\delta U(a, \beta') + \frac{1}{3\sqrt{15}}\delta U(a, \gamma) + \frac{\sqrt{\frac{5}{3}}}{4}\delta U(x', \beta') \\
& + \frac{1}{4}\sqrt{\frac{3}{5}}\delta U(\alpha', \beta') - \frac{2}{3}\sqrt{\frac{5}{3}}\delta J(a, x') + \frac{2}{\sqrt{15}}\delta J(a, \alpha') , \\
\delta A(a; a, \alpha') &= \frac{\sqrt{\frac{5}{3}}}{8}\delta U(z) - \frac{53}{40\sqrt{15}}\delta U(\alpha') + \frac{1}{2\sqrt{15}}\delta J(x', \alpha') - \frac{1}{3}\sqrt{\frac{5}{3}}\delta U(x', y') \\
& + \frac{23}{20\sqrt{15}}\delta U(a, \alpha') + \sqrt{\frac{3}{5}}\delta U(x', \alpha') - \frac{\sqrt{\frac{5}{3}}}{12}\delta U(a, \gamma) - 2\sqrt{\frac{3}{5}}\delta U(z, \alpha') \\
& - \frac{19}{3\sqrt{15}}\delta J(a, x') + \frac{8\sqrt{\frac{3}{5}}}{5}\delta J(a, \alpha') - \frac{1}{2}\sqrt{\frac{5}{3}}\delta J(a, z) , \\
\delta A(a; a, \beta') &= -\frac{\sqrt{\frac{5}{3}}}{8}\delta U(z) + \frac{53}{40\sqrt{15}}\delta U(\alpha') - \frac{1}{2\sqrt{15}}\delta J(x', \alpha') + \frac{1}{3}\sqrt{\frac{5}{3}}\delta U(x', y') \\
& - \frac{4\sqrt{\frac{3}{5}}}{5}\delta U(a, \alpha') - \frac{7}{4\sqrt{15}}\delta U(x', \alpha') + \frac{\sqrt{\frac{5}{3}}}{4}\delta U(a, \beta') + \frac{\sqrt{\frac{5}{3}}}{12}\delta U(a, \gamma) \\
& - \frac{\sqrt{\frac{5}{3}}}{4}\delta U(x', \beta') + 2\sqrt{\frac{3}{5}}\delta U(z, \alpha') + \frac{19}{3\sqrt{15}}\delta J(a, x') - \frac{8\sqrt{\frac{3}{5}}}{5}\delta J(a, \alpha') \\
& + \frac{1}{2}\sqrt{\frac{5}{3}}\delta J(a, z) ,
\end{aligned}$$

$$\begin{aligned}
\delta A(x'; x', \alpha') &= \frac{9\sqrt{\frac{3}{5}}}{20} \delta U(\alpha') + \frac{1}{\sqrt{15}} \delta J(x', \alpha') - \frac{16}{5\sqrt{15}} \delta U(a, \alpha') + \frac{1}{2\sqrt{15}} \delta U(x', \alpha') \\
&\quad + \frac{32}{3\sqrt{15}} \delta J(a, x') - \frac{32}{5\sqrt{15}} \delta J(a, \alpha') , \\
\delta A(x'; x', \beta') &= \frac{1}{2\sqrt{15}} \delta U(z) - \frac{11}{100\sqrt{15}} \delta U(\alpha') - \frac{\sqrt{\frac{3}{5}}}{5} \delta J(x', \alpha') - \frac{7}{2\sqrt{15}} \delta U(x', y') \\
&\quad - \frac{32}{25\sqrt{15}} \delta U(a, \alpha') + \frac{4\sqrt{\frac{3}{5}}}{5} \delta U(x', \alpha') - \frac{3\sqrt{\frac{3}{5}}}{5} \delta U(a, \beta') - \frac{1}{5\sqrt{15}} \delta U(a, \gamma) \\
&\quad + 2\sqrt{\frac{3}{5}} \delta U(x', \beta') - \frac{2\sqrt{\frac{3}{5}}}{5} \delta U(z, \alpha') + \frac{\sqrt{\frac{3}{5}}}{10} \delta U(\alpha', \beta') + \frac{6\sqrt{\frac{3}{5}}}{5} \delta J(a, x') \\
&\quad + \frac{26}{25\sqrt{15}} \delta J(a, \alpha') - \frac{2}{\sqrt{15}} \delta J(a, z) , \\
\delta A(x'; x', \gamma) &= -\frac{\sqrt{15}}{32} \delta U(z) + \frac{53}{32\sqrt{15}} \delta U(\alpha') - \frac{1}{8} \sqrt{\frac{3}{5}} \delta J(x', \alpha') - \frac{1}{6} \sqrt{\frac{5}{3}} \delta U(x', y') \\
&\quad + \frac{\sqrt{\frac{5}{3}}}{8} \delta U(x', z) - \frac{5\sqrt{\frac{5}{3}}}{8} \delta U(a, \alpha') - \frac{7}{16} \sqrt{\frac{3}{5}} \delta U(x', \alpha') - \frac{\sqrt{\frac{5}{3}}}{24} \delta U(a, \gamma) \\
&\quad + \frac{3}{8} \sqrt{\frac{3}{5}} \delta U(z, \alpha') + \frac{77}{12\sqrt{15}} \delta J(a, x') - \frac{5}{4} \sqrt{\frac{5}{3}} \delta J(a, \alpha') + \frac{1}{8\sqrt{15}} \delta J(a, z) , \\
\delta A(y'; x', \alpha') &= -\frac{9\sqrt{\frac{3}{5}}}{20} \delta U(\alpha') - \frac{1}{\sqrt{15}} \delta J(x', \alpha') + \frac{16}{5\sqrt{15}} \delta U(a, \alpha') - \frac{1}{2\sqrt{15}} \delta U(x', \alpha') \\
&\quad - \frac{32}{3\sqrt{15}} \delta J(a, x') + \frac{32}{5\sqrt{15}} \delta J(a, \alpha') , \\
\delta A(\gamma; x', \alpha') &= -\frac{\sqrt{\frac{5}{3}}}{8} \delta U(z) + \frac{53}{40\sqrt{15}} \delta U(\alpha') - \frac{1}{2\sqrt{15}} \delta J(x', \alpha') + \frac{1}{3} \sqrt{\frac{5}{3}} \delta U(x', y') \\
&\quad - \frac{23}{20\sqrt{15}} \delta U(a, \alpha') - \sqrt{\frac{3}{5}} \delta U(x', \alpha') + \frac{\sqrt{\frac{5}{3}}}{12} \delta U(a, \gamma) + 2\sqrt{\frac{3}{5}} \delta U(z, \alpha') \\
&\quad + \frac{19}{3\sqrt{15}} \delta J(a, x') - \frac{8\sqrt{\frac{3}{5}}}{5} \delta J(a, \alpha') + \frac{1}{2} \sqrt{\frac{5}{3}} \delta J(a, z) , \\
\delta A(y'; y', \beta') &= -\frac{1}{2\sqrt{15}} \delta U(z) + \frac{11}{100\sqrt{15}} \delta U(\alpha') + \frac{\sqrt{\frac{3}{5}}}{5} \delta J(x', \alpha') + \frac{7}{2\sqrt{15}} \delta U(x', y') \\
&\quad + \frac{32}{25\sqrt{15}} \delta U(a, \alpha') - \frac{4\sqrt{\frac{3}{5}}}{5} \delta U(x', \alpha') + \frac{3\sqrt{\frac{3}{5}}}{5} \delta U(a, \beta') + \frac{1}{5\sqrt{15}} \delta U(a, \gamma) \\
&\quad - 2\sqrt{\frac{3}{5}} \delta U(x', \beta') + \frac{2\sqrt{\frac{3}{5}}}{5} \delta U(z, \alpha') - \frac{\sqrt{\frac{3}{5}}}{10} \delta U(\alpha', \beta') - \frac{6\sqrt{\frac{3}{5}}}{5} \delta J(a, x') \\
&\quad - \frac{26}{25\sqrt{15}} \delta J(a, \alpha') + \frac{2}{\sqrt{15}} \delta J(a, z) , \\
\delta A(y'; y', \gamma) &= \frac{\sqrt{15}}{32} \delta U(z) - \frac{53}{32\sqrt{15}} \delta U(\alpha') + \frac{1}{8} \sqrt{\frac{3}{5}} \delta J(x', \alpha') + \frac{1}{6} \sqrt{\frac{5}{3}} \delta U(x', y') \\
&\quad - \frac{\sqrt{\frac{5}{3}}}{8} \delta U(x', z) + \frac{5\sqrt{\frac{5}{3}}}{8} \delta U(a, \alpha') + \frac{7}{16} \sqrt{\frac{3}{5}} \delta U(x', \alpha') + \frac{\sqrt{\frac{5}{3}}}{24} \delta U(a, \gamma) \\
&\quad - \frac{3}{8} \sqrt{\frac{3}{5}} \delta U(z, \alpha') - \frac{77}{12\sqrt{15}} \delta J(a, x') + \frac{5}{4} \sqrt{\frac{5}{3}} \delta J(a, \alpha') - \frac{1}{8\sqrt{15}} \delta J(a, z) ,
\end{aligned}$$



$$\begin{aligned}
\delta A(\gamma; y', \beta') &= \frac{\sqrt{\frac{5}{3}}}{8} \delta U(z) - \frac{53}{40\sqrt{15}} \delta U(\alpha') + \frac{1}{2\sqrt{15}} \delta J(x', \alpha') - \frac{1}{3} \sqrt{\frac{5}{3}} \delta U(x', y') \\
&\quad + \frac{4\sqrt{\frac{3}{5}}}{5} \delta U(a, \alpha') + \frac{7}{4\sqrt{15}} \delta U(x', \alpha') - \frac{\sqrt{\frac{5}{3}}}{4} \delta U(a, \beta') - \frac{\sqrt{\frac{5}{3}}}{12} \delta U(a, \gamma) \\
&\quad + \frac{\sqrt{\frac{5}{3}}}{4} \delta U(x', \beta') - 2\sqrt{\frac{3}{5}} \delta U(z, \alpha') - \frac{19}{3\sqrt{15}} \delta J(a, x') + \frac{8\sqrt{\frac{3}{5}}}{5} \delta J(a, \alpha') \\
&\quad - \frac{1}{2} \sqrt{\frac{5}{3}} \delta J(a, z) , \\
\delta S(a, x'; y', z) &= \frac{\sqrt{\frac{5}{3}}}{4} \delta U(z) - \frac{161}{80\sqrt{15}} \delta U(\alpha') + \frac{1}{4} \sqrt{\frac{3}{5}} \delta J(x', \alpha') + \frac{1}{3} \sqrt{\frac{5}{3}} \delta U(x', y') \\
&\quad - \frac{\sqrt{\frac{5}{3}}}{4} \delta U(x', z) + \frac{73}{20\sqrt{15}} \delta U(a, \alpha') + \frac{7\sqrt{\frac{3}{5}}}{8} \delta U(x', \alpha') + \frac{\sqrt{\frac{5}{3}}}{12} \delta U(a, \gamma) \\
&\quad - \frac{3}{4} \sqrt{\frac{3}{5}} \delta U(z, \alpha') - \frac{17}{6\sqrt{15}} \delta J(a, x') + \frac{73}{10\sqrt{15}} \delta J(a, \alpha') - \sqrt{\frac{5}{3}} \delta J(a, z) , \\
\delta S(a, x'; z, y') &= -\frac{\sqrt{15}}{32} \delta U(z) + \frac{53}{32\sqrt{15}} \delta U(\alpha') - \frac{1}{8} \sqrt{\frac{3}{5}} \delta J(x', \alpha') - \frac{1}{6} \sqrt{\frac{5}{3}} \delta U(x', y') \\
&\quad + \frac{\sqrt{\frac{5}{3}}}{8} \delta U(x', z) - \frac{5\sqrt{\frac{5}{3}}}{8} \delta U(a, \alpha') - \frac{7}{16} \sqrt{\frac{3}{5}} \delta U(x', \alpha') - \frac{\sqrt{\frac{5}{3}}}{24} \delta U(a, \gamma) \\
&\quad + \frac{3}{8} \sqrt{\frac{3}{5}} \delta U(z, \alpha') + \frac{77}{12\sqrt{15}} \delta J(a, x') - \frac{5}{4} \sqrt{\frac{5}{3}} \delta J(a, \alpha') + \frac{1}{8\sqrt{15}} \delta J(a, z) , \\
\delta S(a, x'; z, \beta') &= -\frac{13}{96} \delta U(z) + \frac{181}{600} \delta U(\alpha') + \frac{1}{10} \delta J(x', \alpha') + \frac{7}{12} \delta U(x', y') \\
&\quad - \frac{53}{150} \delta U(a, \alpha') - \frac{2}{5} \delta U(x', \alpha') + \frac{3}{10} \delta U(a, \beta') + \frac{1}{30} \delta U(a, \gamma) \\
&\quad - \frac{1}{4} \delta U(x', \beta') + \frac{2}{10} \delta U(z, \alpha') - \frac{1}{20} \delta U(\alpha', \beta') + \frac{16}{15} \delta J(a, x') \\
&\quad - \frac{98}{75} \delta J(a, \alpha') + \frac{13}{24} \delta J(a, z) , \\
\delta S(a, x'; \beta', z) &= -\frac{1}{12} \delta U(z) + \frac{143}{2400} \delta U(\alpha') - \frac{7}{40} \delta J(x', \alpha') - \frac{1}{12} \delta U(x', y') \\
&\quad + \frac{1}{8} \delta U(x', z) - \frac{199}{600} \delta U(a, \alpha') + \frac{11}{80} \delta U(x', \alpha') + \frac{2}{10} \delta U(a, \beta') \\
&\quad + \frac{11}{120} \delta U(a, \gamma) - \frac{1}{4} \delta U(x', \beta') + \frac{1}{40} \delta U(z, \alpha') + \frac{1}{20} \delta U(\alpha', \beta') \\
&\quad - \frac{7}{60} \delta J(a, x') - \frac{19}{300} \delta J(a, \alpha') + \frac{1}{3} \delta J(a, z) , \\
\delta S(a, x'; \beta', \gamma) &= -\frac{1}{8\sqrt{15}} \delta U(\alpha') + \frac{1}{2} \sqrt{\frac{5}{3}} \delta J(x', \alpha') + \frac{13\sqrt{\frac{5}{3}}}{12} \delta U(x', y') + \frac{7}{2\sqrt{15}} \delta U(a, \alpha') \\
&\quad - \frac{1}{2} \sqrt{\frac{5}{3}} \delta U(x', \alpha') + \frac{2}{\sqrt{15}} \delta U(a, \beta') - \frac{1}{3\sqrt{15}} \delta U(a, \gamma) - \frac{\sqrt{\frac{5}{3}}}{4} \delta U(x', \beta') \\
&\quad - \frac{1}{4} \sqrt{\frac{3}{5}} \delta U(\alpha', \beta') + \frac{2}{3} \sqrt{\frac{5}{3}} \delta J(a, x') - \frac{2}{\sqrt{15}} \delta J(a, \alpha') , \\
\delta S(a, x'; \gamma, y') &= -\frac{3}{8} \delta U(z) + \frac{51}{50} \delta U(\alpha') - \frac{3}{10} \delta J(x', \alpha') - \frac{189}{100} \delta U(a, \alpha') \\
&\quad - \frac{21}{20} \delta U(x', \alpha') + \frac{9}{10} \delta U(z, \alpha') + \frac{33}{10} \delta J(a, x') - \frac{189}{50} \delta J(a, \alpha')
\end{aligned}$$

$$\begin{aligned}
& + \frac{3}{2} \delta J(a, z) , \\
\delta S(a, x'; \gamma, \beta') &= -\frac{\sqrt{\frac{5}{3}}}{8} \delta U(z) + \frac{53}{40\sqrt{15}} \delta U(\alpha') - \frac{1}{2\sqrt{15}} \delta J(x', \alpha') + \frac{1}{3} \sqrt{\frac{5}{3}} \delta U(x', y') \\
& - \frac{4\sqrt{\frac{3}{5}}}{5} \delta U(a, \alpha') - \frac{7}{4\sqrt{15}} \delta U(x', \alpha') + \frac{\sqrt{\frac{5}{3}}}{4} \delta U(a, \beta') + \frac{\sqrt{\frac{5}{3}}}{12} \delta U(a, \gamma) \\
& - \frac{\sqrt{\frac{5}{3}}}{4} \delta U(x', \beta') + 2\sqrt{\frac{3}{5}} \delta U(z, \alpha') + \frac{19}{3\sqrt{15}} \delta J(a, x') - \frac{8\sqrt{\frac{3}{5}}}{5} \delta J(a, \alpha') \\
& + \frac{1}{2} \sqrt{\frac{5}{3}} \delta J(a, z) , \\
\delta S(a, y'; z, x') &= -\frac{\sqrt{15}}{32} \delta U(z) + \frac{53}{32\sqrt{15}} \delta U(\alpha') - \frac{1}{8} \sqrt{\frac{3}{5}} \delta J(x', \alpha') - \frac{1}{6} \sqrt{\frac{5}{3}} \delta U(x', y') \\
& + \frac{\sqrt{\frac{5}{3}}}{8} \delta U(x', z) - \frac{5\sqrt{\frac{5}{3}}}{8} \delta U(a, \alpha') - \frac{7}{16} \sqrt{\frac{3}{5}} \delta U(x', \alpha') - \frac{\sqrt{\frac{5}{3}}}{24} \delta U(a, \gamma) \\
& + \frac{3}{8} \sqrt{\frac{3}{5}} \delta U(z, \alpha') + \frac{77}{12\sqrt{15}} \delta J(a, x') - \frac{5}{4} \sqrt{\frac{5}{3}} \delta J(a, \alpha') + \frac{1}{8\sqrt{15}} \delta J(a, z) , \\
\delta S(a, y'; z, \alpha') &= \frac{5}{96} \delta U(z) - \frac{7}{120} \delta U(\alpha') + \frac{1}{6} \delta J(x', \alpha') + \frac{1}{30} \delta U(a, \alpha') \\
& + \frac{1}{12} \delta U(x', \alpha') + \frac{2}{18} \delta J(a, x') + \frac{1}{15} \delta J(a, \alpha') - \frac{5}{24} \delta J(a, z) , \\
\delta S(a, y'; \alpha', z) &= \frac{1}{6} \delta U(z) - \frac{727}{2400} \delta U(\alpha') - \frac{11}{120} \delta J(x', \alpha') - \frac{1}{2} \delta U(x', y') \\
& - \frac{1}{8} \delta U(x', z) + \frac{91}{600} \delta U(a, \alpha') + \frac{163}{240} \delta U(x', \alpha') - \frac{1}{8} \delta U(a, \gamma) \\
& - \frac{9}{40} \delta U(z, \alpha') - \frac{191}{180} \delta J(a, x') + \frac{391}{300} \delta J(a, \alpha') - \frac{2}{3} \delta J(a, z) , \\
\delta S(a, y'; \alpha', \gamma) &= \frac{\sqrt{\frac{5}{3}}}{4} \delta U(z) - \frac{151}{40\sqrt{15}} \delta U(\alpha') - 2\sqrt{\frac{3}{5}} \delta J(x', \alpha') - \frac{2}{3} \sqrt{\frac{5}{3}} \delta U(x', y') \\
& + \frac{29}{5\sqrt{15}} \delta U(a, \alpha') + \frac{19}{4\sqrt{15}} \delta U(x', \alpha') - \frac{1}{6} \sqrt{\frac{5}{3}} \delta U(a, \gamma) - \sqrt{\frac{3}{5}} \delta U(z, \alpha') \\
& - \frac{43}{3\sqrt{15}} \delta J(a, x') + \frac{83}{5\sqrt{15}} \delta J(a, \alpha') - \sqrt{\frac{5}{3}} \delta J(a, z) , \\
\delta S(a, y'; \gamma, x') &= \frac{3}{8} \delta U(z) - \frac{51}{50} \delta U(\alpha') + \frac{3}{10} \delta J(x', \alpha') + \frac{189}{100} \delta U(a, \alpha') \\
& + \frac{21}{20} \delta U(x', \alpha') - \frac{9}{10} \delta U(z, \alpha') - \frac{33}{10} \delta J(a, x') + \frac{189}{50} \delta J(a, \alpha') \\
& - \frac{3}{2} \delta J(a, z) , \\
\delta S(a, y'; \gamma, \alpha') &= -\frac{\sqrt{\frac{5}{3}}}{8} \delta U(z) + \frac{53}{40\sqrt{15}} \delta U(\alpha') - \frac{1}{2\sqrt{15}} \delta J(x', \alpha') + \frac{1}{3} \sqrt{\frac{5}{3}} \delta U(x', y') \\
& - \frac{23}{20\sqrt{15}} \delta U(a, \alpha') - \sqrt{\frac{3}{5}} \delta U(x', \alpha') + \frac{\sqrt{\frac{5}{3}}}{12} \delta U(a, \gamma) + 2\sqrt{\frac{3}{5}} \delta U(z, \alpha') \\
& + \frac{19}{3\sqrt{15}} \delta J(a, x') - \frac{8\sqrt{\frac{3}{5}}}{5} \delta J(a, \alpha') + \frac{1}{2} \sqrt{\frac{5}{3}} \delta J(a, z) , \\
\delta S(a, z; \alpha', y') &= -\frac{1}{16} \delta U(z) + \frac{149}{800} \delta U(\alpha') + \frac{17}{40} \delta J(x', \alpha') + \frac{1}{2} \delta U(x', y')
\end{aligned}$$

$$\begin{aligned}
& + \frac{1}{8}\delta U(x', z) - \frac{17}{200}\delta U(a, \alpha') - \frac{41}{80}\delta U(x', \alpha') + \frac{1}{8}\delta U(a, \gamma) \\
& + \frac{9}{40}\delta U(z, \alpha') + \frac{77}{60}\delta J(a, x') - \frac{117}{100}\delta J(a, \alpha') + \frac{1}{4}\delta J(a, z) , \\
\delta S(a, z; \beta', x') &= -\frac{3}{16}\delta U(z) + \frac{87}{160}\delta U(\alpha') + \frac{3}{8}\delta J(x', \alpha') + \frac{5}{4}\delta U(x', y') \\
& - \frac{1}{8}\delta U(x', z) - \frac{3}{8}\delta U(a, \alpha') - \frac{15}{16}\delta U(x', \alpha') + \frac{2}{5}\delta U(a, \beta') \\
& - \frac{1}{40}\delta U(a, \gamma) - \frac{1}{4}\delta U(x', \beta') + \frac{3}{8}\delta U(z, \alpha') - \frac{3}{20}\delta U(\alpha', \beta') \\
& + \frac{9}{4}\delta J(a, x') - \frac{51}{20}\delta J(a, \alpha') + \frac{3}{4}\delta J(a, z) , \\
\delta S(a, \alpha'; \gamma, y') &= -\frac{\sqrt{\frac{5}{3}}}{8}\delta U(z) + \frac{53}{40\sqrt{15}}\delta U(\alpha') - \frac{1}{2\sqrt{15}}\delta J(x', \alpha') + \frac{1}{3}\sqrt{\frac{5}{3}}\delta U(x', y') \\
& - \frac{23}{20\sqrt{15}}\delta U(a, \alpha') - \sqrt{\frac{3}{5}}\delta U(x', \alpha') + \frac{\sqrt{\frac{5}{3}}}{12}\delta U(a, \gamma) + 2\sqrt{\frac{3}{5}}\delta U(z, \alpha') \\
& + \frac{19}{3\sqrt{15}}\delta J(a, x') - \frac{8\sqrt{\frac{3}{5}}}{5}\delta J(a, \alpha') + \frac{1}{2}\sqrt{\frac{5}{3}}\delta J(a, z) , \\
\delta S(a, \alpha'; \gamma, \beta') &= -\frac{5}{24}\delta U(z) + \frac{29}{60}\delta U(\alpha') - \frac{1}{6}\delta J(x', \alpha') + \frac{5}{12}\delta U(x', y') \\
& - \frac{17}{15}\delta U(a, \alpha') - \frac{7}{12}\delta U(x', \alpha') - \frac{1}{4}\delta U(a, \beta') + \frac{2}{3}\delta U(a, \gamma) \\
& + \frac{1}{2}\delta U(z, \alpha') + \frac{1}{4}\delta U(\alpha', \beta') + \frac{43}{18}\delta J(a, x') - \frac{53}{30}\delta J(a, \alpha') \\
& + \frac{5}{6}\delta J(a, z) , \\
\delta S(a, \beta'; \gamma, x') &= -\frac{\sqrt{\frac{5}{3}}}{8}\delta U(z) + \frac{53}{40\sqrt{15}}\delta U(\alpha') - \frac{1}{2\sqrt{15}}\delta J(x', \alpha') + \frac{1}{3}\sqrt{\frac{5}{3}}\delta U(x', y') \\
& - \frac{4\sqrt{\frac{3}{5}}}{5}\delta U(a, \alpha') - \frac{7}{4\sqrt{15}}\delta U(x', \alpha') + \frac{\sqrt{\frac{5}{3}}}{4}\delta U(a, \beta') + \frac{\sqrt{\frac{5}{3}}}{12}\delta U(a, \gamma) \\
& - \frac{\sqrt{\frac{5}{3}}}{4}\delta U(x', \beta') + 2\sqrt{\frac{3}{5}}\delta U(z, \alpha') + \frac{19}{3\sqrt{15}}\delta J(a, x') - \frac{8\sqrt{\frac{3}{5}}}{5}\delta J(a, \alpha') \\
& + \frac{1}{2}\sqrt{\frac{5}{3}}\delta J(a, z) , \\
\delta S(a, \beta'; \gamma, \alpha') &= \frac{5}{24}\delta U(z) - \frac{29}{60}\delta U(\alpha') + \frac{1}{6}\delta J(x', \alpha') - \frac{5}{12}\delta U(x', y') \\
& + \frac{17}{15}\delta U(a, \alpha') + \frac{7}{12}\delta U(x', \alpha') + \frac{1}{4}\delta U(a, \beta') - \frac{2}{3}\delta U(a, \gamma) \\
& - \frac{1}{2}\delta U(z, \alpha') - \frac{1}{4}\delta U(\alpha', \beta') - \frac{43}{18}\delta J(a, x') + \frac{53}{30}\delta J(a, \alpha') \\
& - \frac{5}{6}\delta J(a, z) , \\
\delta S(x', y'; \alpha', \beta') &= \frac{1}{12}\delta U(z) - \frac{29}{150}\delta U(\alpha') + \frac{1}{15}\delta J(x', \alpha') + \frac{1}{3}\delta U(x', y') \\
& + \frac{34}{75}\delta U(a, \alpha') + \frac{7}{30}\delta U(x', \alpha') + \frac{1}{10}\delta U(a, \beta') + \frac{7}{30}\delta U(a, \gamma) \\
& - \frac{2}{10}\delta U(z, \alpha') - \frac{1}{10}\delta U(\alpha', \beta') - \frac{13}{45}\delta J(a, x') + \frac{53}{75}\delta J(a, \alpha') \\
& - \frac{1}{3}\delta J(a, z) ,
\end{aligned}$$

$$\begin{aligned}
\delta S(x', y'; \beta', \alpha') &= -\frac{1}{12}\delta U(z) + \frac{29}{150}\delta U(\alpha') - \frac{1}{15}\delta J(x', \alpha') - \frac{1}{3}\delta U(x', y') \\
&\quad - \frac{34}{75}\delta U(a, \alpha') - \frac{7}{30}\delta U(x', \alpha') - \frac{1}{10}\delta U(a, \beta') - \frac{7}{30}\delta U(a, \gamma) \\
&\quad + \frac{2}{10}\delta U(z, \alpha') + \frac{1}{10}\delta U(\alpha', \beta') + \frac{13}{45}\delta J(a, x') - \frac{53}{75}\delta J(a, \alpha') \\
&\quad + \frac{1}{3}\delta J(a, z) , \\
\delta S(x', z; \alpha', \gamma) &= \frac{1}{16}\delta U(z) - \frac{149}{800}\delta U(\alpha') - \frac{17}{40}\delta J(x', \alpha') - \frac{1}{2}\delta U(x', y') \\
&\quad - \frac{1}{8}\delta U(x', z) + \frac{17}{200}\delta U(a, \alpha') + \frac{41}{80}\delta U(x', \alpha') - \frac{1}{8}\delta U(a, \gamma) \\
&\quad - \frac{9}{40}\delta U(z, \alpha') - \frac{77}{60}\delta J(a, x') + \frac{117}{100}\delta J(a, \alpha') - \frac{1}{4}\delta J(a, z) , \\
\delta S(x', z; \gamma, \alpha') &= -\frac{1}{6}\delta U(z) + \frac{727}{2400}\delta U(\alpha') + \frac{11}{120}\delta J(x', \alpha') + \frac{1}{2}\delta U(x', y') \\
&\quad + \frac{1}{8}\delta U(x', z) - \frac{91}{600}\delta U(a, \alpha') - \frac{163}{240}\delta U(x', \alpha') + \frac{1}{8}\delta U(a, \gamma) \\
&\quad + \frac{9}{40}\delta U(z, \alpha') + \frac{191}{180}\delta J(a, x') - \frac{391}{300}\delta J(a, \alpha') + \frac{2}{3}\delta J(a, z) , \\
\delta S(x', \alpha'; \gamma, z) &= -\frac{5}{96}\delta U(z) + \frac{7}{120}\delta U(\alpha') - \frac{1}{6}\delta J(x', \alpha') - \frac{1}{30}\delta U(a, \alpha') \\
&\quad - \frac{1}{12}\delta U(x', \alpha') - \frac{2}{18}\delta J(a, x') - \frac{1}{15}\delta J(a, \alpha') + \frac{5}{24}\delta J(a, z) , \\
\delta S(y', z; \beta', \gamma) &= -\frac{3}{16}\delta U(z) + \frac{87}{160}\delta U(\alpha') + \frac{3}{8}\delta J(x', \alpha') + \frac{5}{4}\delta U(x', y') \\
&\quad - \frac{1}{8}\delta U(x', z) - \frac{3}{8}\delta U(a, \alpha') - \frac{15}{16}\delta U(x', \alpha') + \frac{2}{5}\delta U(a, \beta') \\
&\quad - \frac{1}{40}\delta U(a, \gamma) - \frac{1}{4}\delta U(x', \beta') + \frac{3}{8}\delta U(z, \alpha') - \frac{3}{20}\delta U(\alpha', \beta') \\
&\quad + \frac{9}{4}\delta J(a, x') - \frac{51}{20}\delta J(a, \alpha') + \frac{3}{4}\delta J(a, z) , \\
\delta S(y', z; \gamma, \beta') &= -\frac{1}{12}\delta U(z) + \frac{143}{2400}\delta U(\alpha') - \frac{7}{40}\delta J(x', \alpha') - \frac{1}{12}\delta U(x', y') \\
&\quad + \frac{1}{8}\delta U(x', z) - \frac{199}{600}\delta U(a, \alpha') + \frac{11}{80}\delta U(x', \alpha') + \frac{2}{10}\delta U(a, \beta') \\
&\quad + \frac{11}{120}\delta U(a, \gamma) - \frac{1}{4}\delta U(x', \beta') + \frac{1}{40}\delta U(z, \alpha') + \frac{1}{20}\delta U(\alpha', \beta') \\
&\quad - \frac{7}{60}\delta J(a, x') - \frac{19}{300}\delta J(a, \alpha') + \frac{1}{3}\delta J(a, z) , \\
\delta S(y', \beta'; \gamma, z) &= -\frac{13}{96}\delta U(z) + \frac{181}{600}\delta U(\alpha') + \frac{1}{10}\delta J(x', \alpha') + \frac{7}{12}\delta U(x', y') \\
&\quad - \frac{53}{150}\delta U(a, \alpha') - \frac{2}{5}\delta U(x', \alpha') + \frac{3}{10}\delta U(a, \beta') + \frac{1}{30}\delta U(a, \gamma) \\
&\quad - \frac{1}{4}\delta U(x', \beta') + \frac{2}{10}\delta U(z, \alpha') - \frac{1}{20}\delta U(\alpha', \beta') + \frac{16}{15}\delta J(a, x') \\
&\quad - \frac{98}{75}\delta J(a, \alpha') + \frac{13}{24}\delta J(a, z) .
\end{aligned}$$

## 2.8 $f$ -orbitals, group $D_{4h}$

Independent parameter variations:

$$\begin{aligned} \delta U(z), \delta U(\alpha'), \delta U(\gamma), \delta U(x', y'), \delta U(x', z), \delta U(a, \alpha'), \delta U(x', \alpha'), \delta U(a, \gamma), \delta U(z, \alpha'), \\ \delta U(x', \gamma), \delta U(z, \gamma), \delta U(\alpha', \beta'), \delta J(x', \gamma), \delta J(x', \alpha'), \delta J(a, x'), \delta J(a, z). \end{aligned}$$

Dependent parameter variations:

$$\begin{aligned} \delta U(y', z) &= \delta U(x', z), \\ \delta U(y', \alpha') &= \delta U(x', \alpha'), \\ \delta U(y', \beta') &= \delta U(x', \beta'), \\ \delta U(z, \beta') &= \frac{1}{6}\delta U(z) - \frac{73}{150}\delta U(\alpha') - \frac{8}{15}\delta J(x', \alpha') - \frac{7}{6}\delta U(x', y') \\ &\quad + \frac{16}{25}\delta U(a, \alpha') - \frac{11}{30}\delta U(x', \alpha') - \frac{3}{5}\delta U(a, \beta') - \frac{1}{15}\delta U(a, \gamma) \\ &\quad + \frac{3}{2}\delta U(x', \beta') + \frac{3}{5}\delta U(z, \alpha') + \frac{1}{10}\delta U(\alpha', \beta') - \frac{106}{45}\delta J(a, x') \\ &\quad + \frac{62}{25}\delta J(a, \alpha') - \frac{2}{3}\delta J(a, z), \\ \delta U(\alpha', \gamma) &= \delta U(a, \alpha'), \\ \delta U(\beta', \gamma) &= \delta U(a, \beta'), \\ \delta J(a, y') &= \delta J(a, x'), \\ \delta J(a, \alpha') &= \delta J(a, \alpha'), \\ \delta J(a, \beta') &= -\frac{1}{4}\delta U(\alpha') + \frac{1}{4}\delta U(\beta') + \frac{1}{2}\delta U(a, \alpha') - \frac{1}{2}\delta U(a, \beta') \\ &\quad + \delta J(a, \alpha'), \\ \delta J(a, \gamma) &= -\frac{1}{2}\delta U(a, \gamma), \\ \delta J(x', y') &= -\frac{1}{2}\delta U(x', y'), \\ \delta J(x', z) &= \frac{1}{4}\delta U(z) + \frac{1}{8}\delta U(\alpha') - \frac{1}{2}\delta U(x', z) - \frac{1}{4}\delta U(a, \alpha') \\ &\quad + \frac{5}{6}\delta J(a, x') - \frac{1}{2}\delta J(a, \alpha'), \\ \delta J(x', \beta') &= \frac{1}{2}\delta U(z) - \frac{171}{100}\delta U(\alpha') + \frac{1}{4}\delta U(\beta') - \frac{3}{5}\delta J(x', \alpha') \\ &\quad - \frac{7}{2}\delta U(x', y') + \frac{48}{25}\delta U(a, \alpha') + \frac{12}{5}\delta U(x', \alpha') - \frac{9}{5}\delta U(a, \beta') \\ &\quad - \frac{2}{10}\delta U(a, \gamma) + \delta U(x', \beta') - \frac{6}{5}\delta U(z, \alpha') + \frac{3}{10}\delta U(\alpha', \beta') \\ &\quad - \frac{106}{15}\delta J(a, x') + \frac{186}{25}\delta J(a, \alpha') - 2\delta J(a, z), \\ \delta J(x', \gamma) &= \delta J(a, x'), \\ \delta J(y', z) &= \frac{1}{4}\delta U(z) + \frac{1}{8}\delta U(\alpha') - \frac{1}{2}\delta U(x', z) - \frac{1}{4}\delta U(a, \alpha') \\ &\quad + \frac{5}{6}\delta J(a, x') - \frac{1}{2}\delta J(a, \alpha'), \\ \delta J(y', \alpha') &= \delta J(x', \alpha'), \\ \delta J(y', \beta') &= \frac{1}{2}\delta U(z) - \frac{171}{100}\delta U(\alpha') + \frac{1}{4}\delta U(\beta') - \frac{3}{5}\delta J(x', \alpha') \\ &\quad - \frac{7}{2}\delta U(x', y') + \frac{48}{25}\delta U(a, \alpha') + \frac{12}{5}\delta U(x', \alpha') - \frac{9}{5}\delta U(a, \beta') \\ &\quad - \frac{2}{10}\delta U(a, \gamma) + \delta U(x', \beta') - \frac{6}{5}\delta U(z, \alpha') + \frac{3}{10}\delta U(\alpha', \beta') \end{aligned}$$

$$\begin{aligned}
& -\frac{106}{15}\delta J(a, x') + \frac{186}{25}\delta J(a, \alpha') - 2\delta J(a, z) , \\
\delta J(y', \gamma) &= \delta J(a, x') , \\
\delta J(z, \alpha') &= \frac{5}{8}\delta U(z) - \frac{17}{10}\delta U(\alpha') + \frac{3}{2}\delta J(x', \alpha') + \frac{63}{20}\delta U(a, \alpha') \\
&+ \frac{3}{4}\delta U(x', \alpha') - \frac{1}{2}\delta U(z, \alpha') - \frac{13}{2}\delta J(a, x') + \frac{63}{10}\delta J(a, \alpha') \\
&- \frac{3}{2}\delta J(a, z) , \\
\delta J(z, \beta') &= \frac{31}{24}\delta U(z) - \frac{1169}{300}\delta U(\alpha') + \frac{1}{4}\delta U(\beta') - \frac{19}{30}\delta J(x', \alpha') \\
&- \frac{14}{3}\delta U(x', y') + \frac{571}{100}\delta U(a, \alpha') + \frac{227}{60}\delta U(x', \alpha') - \frac{12}{5}\delta U(a, \beta') \\
&- \frac{4}{5}\delta U(a, \gamma) + \frac{3}{2}\delta U(x', \beta') - \frac{21}{10}\delta U(z, \alpha') + \frac{2}{5}\delta U(\alpha', \beta') \\
&- \frac{1433}{90}\delta J(a, x') + \frac{811}{50}\delta J(a, \alpha') - \frac{25}{6}\delta J(a, z) , \\
\delta J(z, \gamma) &= \delta J(a, z) , \\
\delta J(\alpha', \beta') &= \frac{1}{4}\delta U(\alpha') + \frac{1}{4}\delta U(\beta') - \frac{1}{2}\delta U(\alpha', \beta') , \\
\delta J(\alpha', \gamma) &= \delta J(a, \alpha') , \\
\delta J(\beta', \gamma) &= -\frac{1}{4}\delta U(\alpha') + \frac{1}{4}\delta U(\beta') + \frac{1}{2}\delta U(a, \alpha') - \frac{1}{2}\delta U(a, \beta') \\
&+ \delta J(a, \alpha') , \\
\delta T(a; x', \alpha') &= -\frac{\sqrt{\frac{5}{3}}}{4}\delta U(z) + \frac{151}{40\sqrt{15}}\delta U(\alpha') + 2\sqrt{\frac{3}{5}}\delta J(x', \alpha') + \frac{2}{3}\sqrt{\frac{5}{3}}\delta U(x', y') \\
&- \frac{29}{5\sqrt{15}}\delta U(a, \alpha') - \frac{19}{4\sqrt{15}}\delta U(x', \alpha') + \frac{1}{6}\sqrt{\frac{5}{3}}\delta U(a, \gamma) + \sqrt{\frac{3}{5}}\delta U(z, \alpha') \\
&+ \frac{43}{3\sqrt{15}}\delta J(a, x') - \frac{83}{5\sqrt{15}}\delta J(a, \alpha') + \sqrt{\frac{5}{3}}\delta J(a, z) , \\
\delta T(a; y', \beta') &= -\frac{1}{8\sqrt{15}}\delta U(\alpha') + \frac{1}{2}\sqrt{\frac{5}{3}}\delta J(x', \alpha') + \frac{13\sqrt{\frac{5}{3}}}{12}\delta U(x', y') + \frac{7}{2\sqrt{15}}\delta U(a, \alpha') \\
&- \frac{1}{2}\sqrt{\frac{5}{3}}\delta U(x', \alpha') + \frac{2}{\sqrt{15}}\delta U(a, \beta') - \frac{1}{3\sqrt{15}}\delta U(a, \gamma) - \frac{\sqrt{\frac{5}{3}}}{4}\delta U(x', \beta') \\
&- \frac{1}{4}\sqrt{\frac{3}{5}}\delta U(\alpha', \beta') + \frac{2}{3}\sqrt{\frac{5}{3}}\delta J(a, x') - \frac{2}{\sqrt{15}}\delta J(a, \alpha') , \\
\delta T(y'; x', \alpha') &= -\frac{9\sqrt{\frac{3}{5}}}{20}\delta U(\alpha') - \frac{1}{\sqrt{15}}\delta J(x', \alpha') + \frac{16}{5\sqrt{15}}\delta U(a, \alpha') - \frac{1}{2\sqrt{15}}\delta U(x', \alpha') \\
&- \frac{32}{3\sqrt{15}}\delta J(a, x') + \frac{32}{5\sqrt{15}}\delta J(a, \alpha') , \\
\delta T(x'; y', \beta') &= \frac{1}{2\sqrt{15}}\delta U(z) - \frac{11}{100\sqrt{15}}\delta U(\alpha') - \frac{\sqrt{\frac{3}{5}}}{5}\delta J(x', \alpha') - \frac{7}{2\sqrt{15}}\delta U(x', y') \\
&- \frac{32}{25\sqrt{15}}\delta U(a, \alpha') + \frac{4\sqrt{\frac{3}{5}}}{5}\delta U(x', \alpha') - \frac{3\sqrt{\frac{3}{5}}}{5}\delta U(a, \beta') - \frac{1}{5\sqrt{15}}\delta U(a, \gamma) \\
&+ 2\sqrt{\frac{3}{5}}\delta U(x', \beta') - \frac{2\sqrt{\frac{3}{5}}}{5}\delta U(z, \alpha') + \frac{\sqrt{\frac{3}{5}}}{10}\delta U(\alpha', \beta') + \frac{6\sqrt{\frac{3}{5}}}{5}\delta J(a, x')
\end{aligned}$$

$$\begin{aligned}
& + \frac{26}{25\sqrt{15}}\delta J(a, \alpha') - \frac{2}{\sqrt{15}}\delta J(a, z) , \\
\delta T(x'; z, \gamma) &= \frac{\sqrt{\frac{5}{3}}}{4}\delta U(z) - \frac{161}{80\sqrt{15}}\delta U(\alpha') + \frac{1}{4}\sqrt{\frac{3}{5}}\delta J(x', \alpha') + \frac{1}{3}\sqrt{\frac{5}{3}}\delta U(x', y') \\
& - \frac{\sqrt{\frac{5}{3}}}{4}\delta U(x', z) + \frac{73}{20\sqrt{15}}\delta U(a, \alpha') + \frac{7\sqrt{\frac{3}{5}}}{8}\delta U(x', \alpha') + \frac{\sqrt{\frac{5}{3}}}{12}\delta U(a, \gamma) \\
& - \frac{3}{4}\sqrt{\frac{3}{5}}\delta U(z, \alpha') - \frac{17}{6\sqrt{15}}\delta J(a, x') + \frac{73}{10\sqrt{15}}\delta J(a, \alpha') - \sqrt{\frac{5}{3}}\delta J(a, z) , \\
\delta T(\gamma; x', \alpha') &= \frac{\sqrt{\frac{5}{3}}}{4}\delta U(z) - \frac{151}{40\sqrt{15}}\delta U(\alpha') - 2\sqrt{\frac{3}{5}}\delta J(x', \alpha') - \frac{2}{3}\sqrt{\frac{5}{3}}\delta U(x', y') \\
& + \frac{29}{5\sqrt{15}}\delta U(a, \alpha') + \frac{19}{4\sqrt{15}}\delta U(x', \alpha') - \frac{1}{6}\sqrt{\frac{5}{3}}\delta U(a, \gamma) - \sqrt{\frac{3}{5}}\delta U(z, \alpha') \\
& - \frac{43}{3\sqrt{15}}\delta J(a, x') + \frac{83}{5\sqrt{15}}\delta J(a, \alpha') - \sqrt{\frac{5}{3}}\delta J(a, z) , \\
\delta T(y'; z, \gamma) &= -\frac{\sqrt{\frac{5}{3}}}{4}\delta U(z) + \frac{161}{80\sqrt{15}}\delta U(\alpha') - \frac{1}{4}\sqrt{\frac{3}{5}}\delta J(x', \alpha') - \frac{1}{3}\sqrt{\frac{5}{3}}\delta U(x', y') \\
& + \frac{\sqrt{\frac{5}{3}}}{4}\delta U(x', z) - \frac{73}{20\sqrt{15}}\delta U(a, \alpha') - \frac{7\sqrt{\frac{3}{5}}}{8}\delta U(x', \alpha') - \frac{\sqrt{\frac{5}{3}}}{12}\delta U(a, \gamma) \\
& + \frac{3}{4}\sqrt{\frac{3}{5}}\delta U(z, \alpha') + \frac{17}{6\sqrt{15}}\delta J(a, x') - \frac{73}{10\sqrt{15}}\delta J(a, \alpha') + \sqrt{\frac{5}{3}}\delta J(a, z) , \\
\delta T(\gamma; y', \beta') &= \frac{1}{8\sqrt{15}}\delta U(\alpha') - \frac{1}{2}\sqrt{\frac{5}{3}}\delta J(x', \alpha') - \frac{13\sqrt{\frac{5}{3}}}{12}\delta U(x', y') - \frac{7}{2\sqrt{15}}\delta U(a, \alpha') \\
& + \frac{1}{2}\sqrt{\frac{5}{3}}\delta U(x', \alpha') - \frac{2}{\sqrt{15}}\delta U(a, \beta') + \frac{1}{3\sqrt{15}}\delta U(a, \gamma) + \frac{\sqrt{\frac{5}{3}}}{4}\delta U(x', \beta') \\
& + \frac{1}{4}\sqrt{\frac{3}{5}}\delta U(\alpha', \beta') - \frac{2}{3}\sqrt{\frac{5}{3}}\delta J(a, x') + \frac{2}{\sqrt{15}}\delta J(a, \alpha') , \\
\delta A(a; a, \alpha') &= \frac{\sqrt{\frac{5}{3}}}{8}\delta U(z) - \frac{53}{40\sqrt{15}}\delta U(\alpha') + \frac{1}{2\sqrt{15}}\delta J(x', \alpha') - \frac{1}{3}\sqrt{\frac{5}{3}}\delta U(x', y') \\
& + \frac{23}{20\sqrt{15}}\delta U(a, \alpha') + \sqrt{\frac{3}{5}}\delta U(x', \alpha') - \frac{\sqrt{\frac{5}{3}}}{12}\delta U(a, \gamma) - 2\sqrt{\frac{3}{5}}\delta U(z, \alpha') \\
& - \frac{19}{3\sqrt{15}}\delta J(a, x') + \frac{8\sqrt{\frac{3}{5}}}{5}\delta J(a, \alpha') - \frac{1}{2}\sqrt{\frac{5}{3}}\delta J(a, z) , \\
\delta A(a; a, \beta') &= -\frac{\sqrt{\frac{5}{3}}}{8}\delta U(z) + \frac{53}{40\sqrt{15}}\delta U(\alpha') - \frac{1}{2\sqrt{15}}\delta J(x', \alpha') + \frac{1}{3}\sqrt{\frac{5}{3}}\delta U(x', y') \\
& - \frac{4\sqrt{\frac{3}{5}}}{5}\delta U(a, \alpha') - \frac{7}{4\sqrt{15}}\delta U(x', \alpha') + \frac{\sqrt{\frac{5}{3}}}{4}\delta U(a, \beta') + \frac{\sqrt{\frac{5}{3}}}{12}\delta U(a, \gamma) \\
& - \frac{\sqrt{\frac{5}{3}}}{4}\delta U(x', \beta') + 2\sqrt{\frac{3}{5}}\delta U(z, \alpha') + \frac{19}{3\sqrt{15}}\delta J(a, x') - \frac{8\sqrt{\frac{3}{5}}}{5}\delta J(a, \alpha') \\
& + \frac{1}{2}\sqrt{\frac{5}{3}}\delta J(a, z) ,
\end{aligned}$$

$$\begin{aligned}
\delta A(x'; x', \alpha') &= \frac{9\sqrt{\frac{3}{5}}}{20} \delta U(\alpha') + \frac{1}{\sqrt{15}} \delta J(x', \alpha') - \frac{16}{5\sqrt{15}} \delta U(a, \alpha') + \frac{1}{2\sqrt{15}} \delta U(x', \alpha') \\
&\quad + \frac{32}{3\sqrt{15}} \delta J(a, x') - \frac{32}{5\sqrt{15}} \delta J(a, \alpha') , \\
\delta A(x'; x', \beta') &= \frac{1}{2\sqrt{15}} \delta U(z) - \frac{11}{100\sqrt{15}} \delta U(\alpha') - \frac{\sqrt{\frac{3}{5}}}{5} \delta J(x', \alpha') - \frac{7}{2\sqrt{15}} \delta U(x', y') \\
&\quad - \frac{32}{25\sqrt{15}} \delta U(a, \alpha') + \frac{4\sqrt{\frac{3}{5}}}{5} \delta U(x', \alpha') - \frac{3\sqrt{\frac{3}{5}}}{5} \delta U(a, \beta') - \frac{1}{5\sqrt{15}} \delta U(a, \gamma) \\
&\quad + 2\sqrt{\frac{3}{5}} \delta U(x', \beta') - \frac{2\sqrt{\frac{3}{5}}}{5} \delta U(z, \alpha') + \frac{\sqrt{\frac{3}{5}}}{10} \delta U(\alpha', \beta') + \frac{6\sqrt{\frac{3}{5}}}{5} \delta J(a, x') \\
&\quad + \frac{26}{25\sqrt{15}} \delta J(a, \alpha') - \frac{2}{\sqrt{15}} \delta J(a, z) , \\
\delta A(x'; x', \gamma) &= -\frac{\sqrt{15}}{32} \delta U(z) + \frac{53}{32\sqrt{15}} \delta U(\alpha') - \frac{1}{8} \sqrt{\frac{3}{5}} \delta J(x', \alpha') - \frac{1}{6} \sqrt{\frac{5}{3}} \delta U(x', y') \\
&\quad + \frac{\sqrt{\frac{5}{3}}}{8} \delta U(x', z) - \frac{5\sqrt{\frac{5}{3}}}{8} \delta U(a, \alpha') - \frac{7}{16} \sqrt{\frac{3}{5}} \delta U(x', \alpha') - \frac{\sqrt{\frac{5}{3}}}{24} \delta U(a, \gamma) \\
&\quad + \frac{3}{8} \sqrt{\frac{3}{5}} \delta U(z, \alpha') + \frac{77}{12\sqrt{15}} \delta J(a, x') - \frac{5}{4} \sqrt{\frac{5}{3}} \delta J(a, \alpha') + \frac{1}{8\sqrt{15}} \delta J(a, z) , \\
\delta A(y'; x', \alpha') &= -\frac{9\sqrt{\frac{3}{5}}}{20} \delta U(\alpha') - \frac{1}{\sqrt{15}} \delta J(x', \alpha') + \frac{16}{5\sqrt{15}} \delta U(a, \alpha') - \frac{1}{2\sqrt{15}} \delta U(x', \alpha') \\
&\quad - \frac{32}{3\sqrt{15}} \delta J(a, x') + \frac{32}{5\sqrt{15}} \delta J(a, \alpha') , \\
\delta A(\gamma; x', \alpha') &= -\frac{\sqrt{\frac{5}{3}}}{8} \delta U(z) + \frac{53}{40\sqrt{15}} \delta U(\alpha') - \frac{1}{2\sqrt{15}} \delta J(x', \alpha') + \frac{1}{3} \sqrt{\frac{5}{3}} \delta U(x', y') \\
&\quad - \frac{23}{20\sqrt{15}} \delta U(a, \alpha') - \sqrt{\frac{3}{5}} \delta U(x', \alpha') + \frac{\sqrt{\frac{5}{3}}}{12} \delta U(a, \gamma) + 2\sqrt{\frac{3}{5}} \delta U(z, \alpha') \\
&\quad + \frac{19}{3\sqrt{15}} \delta J(a, x') - \frac{8\sqrt{\frac{3}{5}}}{5} \delta J(a, \alpha') + \frac{1}{2} \sqrt{\frac{5}{3}} \delta J(a, z) , \\
\delta A(y'; y', \beta') &= -\frac{1}{2\sqrt{15}} \delta U(z) + \frac{11}{100\sqrt{15}} \delta U(\alpha') + \frac{\sqrt{\frac{3}{5}}}{5} \delta J(x', \alpha') + \frac{7}{2\sqrt{15}} \delta U(x', y') \\
&\quad + \frac{32}{25\sqrt{15}} \delta U(a, \alpha') - \frac{4\sqrt{\frac{3}{5}}}{5} \delta U(x', \alpha') + \frac{3\sqrt{\frac{3}{5}}}{5} \delta U(a, \beta') + \frac{1}{5\sqrt{15}} \delta U(a, \gamma) \\
&\quad - 2\sqrt{\frac{3}{5}} \delta U(x', \beta') + \frac{2\sqrt{\frac{3}{5}}}{5} \delta U(z, \alpha') - \frac{\sqrt{\frac{3}{5}}}{10} \delta U(\alpha', \beta') - \frac{6\sqrt{\frac{3}{5}}}{5} \delta J(a, x') \\
&\quad - \frac{26}{25\sqrt{15}} \delta J(a, \alpha') + \frac{2}{\sqrt{15}} \delta J(a, z) , \\
\delta A(y'; y', \gamma) &= \frac{\sqrt{15}}{32} \delta U(z) - \frac{53}{32\sqrt{15}} \delta U(\alpha') + \frac{1}{8} \sqrt{\frac{3}{5}} \delta J(x', \alpha') + \frac{1}{6} \sqrt{\frac{5}{3}} \delta U(x', y') \\
&\quad - \frac{\sqrt{\frac{5}{3}}}{8} \delta U(x', z) + \frac{5\sqrt{\frac{5}{3}}}{8} \delta U(a, \alpha') + \frac{7}{16} \sqrt{\frac{3}{5}} \delta U(x', \alpha') + \frac{\sqrt{\frac{5}{3}}}{24} \delta U(a, \gamma) \\
&\quad - \frac{3}{8} \sqrt{\frac{3}{5}} \delta U(z, \alpha') - \frac{77}{12\sqrt{15}} \delta J(a, x') + \frac{5}{4} \sqrt{\frac{5}{3}} \delta J(a, \alpha') - \frac{1}{8\sqrt{15}} \delta J(a, z) ,
\end{aligned}$$



$$\begin{aligned}
\delta A(\gamma; y', \beta') &= \frac{\sqrt{\frac{5}{3}}}{8} \delta U(z) - \frac{53}{40\sqrt{15}} \delta U(\alpha') + \frac{1}{2\sqrt{15}} \delta J(x', \alpha') - \frac{1}{3} \sqrt{\frac{5}{3}} \delta U(x', y') \\
&\quad + \frac{4\sqrt{\frac{3}{5}}}{5} \delta U(a, \alpha') + \frac{7}{4\sqrt{15}} \delta U(x', \alpha') - \frac{\sqrt{\frac{5}{3}}}{4} \delta U(a, \beta') - \frac{\sqrt{\frac{5}{3}}}{12} \delta U(a, \gamma) \\
&\quad + \frac{\sqrt{\frac{5}{3}}}{4} \delta U(x', \beta') - 2\sqrt{\frac{3}{5}} \delta U(z, \alpha') - \frac{19}{3\sqrt{15}} \delta J(a, x') + \frac{8\sqrt{\frac{3}{5}}}{5} \delta J(a, \alpha') \\
&\quad - \frac{1}{2} \sqrt{\frac{5}{3}} \delta J(a, z) , \\
\delta S(a, x'; y', z) &= \frac{\sqrt{\frac{5}{3}}}{4} \delta U(z) - \frac{161}{80\sqrt{15}} \delta U(\alpha') + \frac{1}{4} \sqrt{\frac{3}{5}} \delta J(x', \alpha') + \frac{1}{3} \sqrt{\frac{5}{3}} \delta U(x', y') \\
&\quad - \frac{\sqrt{\frac{5}{3}}}{4} \delta U(x', z) + \frac{73}{20\sqrt{15}} \delta U(a, \alpha') + \frac{7\sqrt{\frac{3}{5}}}{8} \delta U(x', \alpha') + \frac{\sqrt{\frac{5}{3}}}{12} \delta U(a, \gamma) \\
&\quad - \frac{3}{4} \sqrt{\frac{3}{5}} \delta U(z, \alpha') - \frac{17}{6\sqrt{15}} \delta J(a, x') + \frac{73}{10\sqrt{15}} \delta J(a, \alpha') - \sqrt{\frac{5}{3}} \delta J(a, z) , \\
\delta S(a, x'; z, y') &= -\frac{\sqrt{15}}{32} \delta U(z) + \frac{53}{32\sqrt{15}} \delta U(\alpha') - \frac{1}{8} \sqrt{\frac{3}{5}} \delta J(x', \alpha') - \frac{1}{6} \sqrt{\frac{5}{3}} \delta U(x', y') \\
&\quad + \frac{\sqrt{\frac{5}{3}}}{8} \delta U(x', z) - \frac{5\sqrt{\frac{5}{3}}}{8} \delta U(a, \alpha') - \frac{7}{16} \sqrt{\frac{3}{5}} \delta U(x', \alpha') - \frac{\sqrt{\frac{5}{3}}}{24} \delta U(a, \gamma) \\
&\quad + \frac{3}{8} \sqrt{\frac{3}{5}} \delta U(z, \alpha') + \frac{77}{12\sqrt{15}} \delta J(a, x') - \frac{5}{4} \sqrt{\frac{5}{3}} \delta J(a, \alpha') + \frac{1}{8\sqrt{15}} \delta J(a, z) , \\
\delta S(a, x'; z, \beta') &= -\frac{13}{96} \delta U(z) + \frac{181}{600} \delta U(\alpha') + \frac{1}{10} \delta J(x', \alpha') + \frac{7}{12} \delta U(x', y') \\
&\quad - \frac{53}{150} \delta U(a, \alpha') - \frac{2}{5} \delta U(x', \alpha') + \frac{3}{10} \delta U(a, \beta') + \frac{1}{30} \delta U(a, \gamma) \\
&\quad - \frac{1}{4} \delta U(x', \beta') + \frac{2}{10} \delta U(z, \alpha') - \frac{1}{20} \delta U(\alpha', \beta') + \frac{16}{15} \delta J(a, x') \\
&\quad - \frac{98}{75} \delta J(a, \alpha') + \frac{13}{24} \delta J(a, z) , \\
\delta S(a, x'; \beta', z) &= -\frac{1}{12} \delta U(z) + \frac{143}{2400} \delta U(\alpha') - \frac{7}{40} \delta J(x', \alpha') - \frac{1}{12} \delta U(x', y') \\
&\quad + \frac{1}{8} \delta U(x', z) - \frac{199}{600} \delta U(a, \alpha') + \frac{11}{80} \delta U(x', \alpha') + \frac{2}{10} \delta U(a, \beta') \\
&\quad + \frac{11}{120} \delta U(a, \gamma) - \frac{1}{4} \delta U(x', \beta') + \frac{1}{40} \delta U(z, \alpha') + \frac{1}{20} \delta U(\alpha', \beta') \\
&\quad - \frac{7}{60} \delta J(a, x') - \frac{19}{300} \delta J(a, \alpha') + \frac{1}{3} \delta J(a, z) , \\
\delta S(a, x'; \beta', \gamma) &= -\frac{1}{8\sqrt{15}} \delta U(\alpha') + \frac{1}{2} \sqrt{\frac{5}{3}} \delta J(x', \alpha') + \frac{13\sqrt{\frac{5}{3}}}{12} \delta U(x', y') + \frac{7}{2\sqrt{15}} \delta U(a, \alpha') \\
&\quad - \frac{1}{2} \sqrt{\frac{5}{3}} \delta U(x', \alpha') + \frac{2}{\sqrt{15}} \delta U(a, \beta') - \frac{1}{3\sqrt{15}} \delta U(a, \gamma) - \frac{\sqrt{\frac{5}{3}}}{4} \delta U(x', \beta') \\
&\quad - \frac{1}{4} \sqrt{\frac{3}{5}} \delta U(\alpha', \beta') + \frac{2}{3} \sqrt{\frac{5}{3}} \delta J(a, x') - \frac{2}{\sqrt{15}} \delta J(a, \alpha') , \\
\delta S(a, x'; \gamma, y') &= -\frac{3}{8} \delta U(z) + \frac{51}{50} \delta U(\alpha') - \frac{3}{10} \delta J(x', \alpha') - \frac{189}{100} \delta U(a, \alpha') \\
&\quad - \frac{21}{20} \delta U(x', \alpha') + \frac{9}{10} \delta U(z, \alpha') + \frac{33}{10} \delta J(a, x') - \frac{189}{50} \delta J(a, \alpha')
\end{aligned}$$

$$\begin{aligned}
& + \frac{3}{2} \delta J(a, z) , \\
\delta S(a, x'; \gamma, \beta') &= -\frac{\sqrt{\frac{5}{3}}}{8} \delta U(z) + \frac{53}{40\sqrt{15}} \delta U(\alpha') - \frac{1}{2\sqrt{15}} \delta J(x', \alpha') + \frac{1}{3} \sqrt{\frac{5}{3}} \delta U(x', y') \\
& - \frac{4\sqrt{\frac{3}{5}}}{5} \delta U(a, \alpha') - \frac{7}{4\sqrt{15}} \delta U(x', \alpha') + \frac{\sqrt{\frac{5}{3}}}{4} \delta U(a, \beta') + \frac{\sqrt{\frac{5}{3}}}{12} \delta U(a, \gamma) \\
& - \frac{\sqrt{\frac{5}{3}}}{4} \delta U(x', \beta') + 2\sqrt{\frac{3}{5}} \delta U(z, \alpha') + \frac{19}{3\sqrt{15}} \delta J(a, x') - \frac{8\sqrt{\frac{3}{5}}}{5} \delta J(a, \alpha') \\
& + \frac{1}{2} \sqrt{\frac{5}{3}} \delta J(a, z) , \\
\delta S(a, y'; z, x') &= -\frac{\sqrt{15}}{32} \delta U(z) + \frac{53}{32\sqrt{15}} \delta U(\alpha') - \frac{1}{8} \sqrt{\frac{3}{5}} \delta J(x', \alpha') - \frac{1}{6} \sqrt{\frac{5}{3}} \delta U(x', y') \\
& + \frac{\sqrt{\frac{5}{3}}}{8} \delta U(x', z) - \frac{5\sqrt{\frac{5}{3}}}{8} \delta U(a, \alpha') - \frac{7}{16} \sqrt{\frac{3}{5}} \delta U(x', \alpha') - \frac{\sqrt{\frac{5}{3}}}{24} \delta U(a, \gamma) \\
& + \frac{3}{8} \sqrt{\frac{3}{5}} \delta U(z, \alpha') + \frac{77}{12\sqrt{15}} \delta J(a, x') - \frac{5}{4} \sqrt{\frac{5}{3}} \delta J(a, \alpha') + \frac{1}{8\sqrt{15}} \delta J(a, z) , \\
\delta S(a, y'; z, \alpha') &= \frac{5}{96} \delta U(z) - \frac{7}{120} \delta U(\alpha') + \frac{1}{6} \delta J(x', \alpha') + \frac{1}{30} \delta U(a, \alpha') \\
& + \frac{1}{12} \delta U(x', \alpha') + \frac{2}{18} \delta J(a, x') + \frac{1}{15} \delta J(a, \alpha') - \frac{5}{24} \delta J(a, z) , \\
\delta S(a, y'; \alpha', z) &= \frac{1}{6} \delta U(z) - \frac{727}{2400} \delta U(\alpha') - \frac{11}{120} \delta J(x', \alpha') - \frac{1}{2} \delta U(x', y') \\
& - \frac{1}{8} \delta U(x', z) + \frac{91}{600} \delta U(a, \alpha') + \frac{163}{240} \delta U(x', \alpha') - \frac{1}{8} \delta U(a, \gamma) \\
& - \frac{9}{40} \delta U(z, \alpha') - \frac{191}{180} \delta J(a, x') + \frac{391}{300} \delta J(a, \alpha') - \frac{2}{3} \delta J(a, z) , \\
\delta S(a, y'; \alpha', \gamma) &= \frac{\sqrt{\frac{5}{3}}}{4} \delta U(z) - \frac{151}{40\sqrt{15}} \delta U(\alpha') - 2\sqrt{\frac{3}{5}} \delta J(x', \alpha') - \frac{2}{3} \sqrt{\frac{5}{3}} \delta U(x', y') \\
& + \frac{29}{5\sqrt{15}} \delta U(a, \alpha') + \frac{19}{4\sqrt{15}} \delta U(x', \alpha') - \frac{1}{6} \sqrt{\frac{5}{3}} \delta U(a, \gamma) - \sqrt{\frac{3}{5}} \delta U(z, \alpha') \\
& - \frac{43}{3\sqrt{15}} \delta J(a, x') + \frac{83}{5\sqrt{15}} \delta J(a, \alpha') - \sqrt{\frac{5}{3}} \delta J(a, z) , \\
\delta S(a, y'; \gamma, x') &= \frac{3}{8} \delta U(z) - \frac{51}{50} \delta U(\alpha') + \frac{3}{10} \delta J(x', \alpha') + \frac{189}{100} \delta U(a, \alpha') \\
& + \frac{21}{20} \delta U(x', \alpha') - \frac{9}{10} \delta U(z, \alpha') - \frac{33}{10} \delta J(a, x') + \frac{189}{50} \delta J(a, \alpha') \\
& - \frac{3}{2} \delta J(a, z) , \\
\delta S(a, y'; \gamma, \alpha') &= -\frac{\sqrt{\frac{5}{3}}}{8} \delta U(z) + \frac{53}{40\sqrt{15}} \delta U(\alpha') - \frac{1}{2\sqrt{15}} \delta J(x', \alpha') + \frac{1}{3} \sqrt{\frac{5}{3}} \delta U(x', y') \\
& - \frac{23}{20\sqrt{15}} \delta U(a, \alpha') - \sqrt{\frac{3}{5}} \delta U(x', \alpha') + \frac{\sqrt{\frac{5}{3}}}{12} \delta U(a, \gamma) + 2\sqrt{\frac{3}{5}} \delta U(z, \alpha') \\
& + \frac{19}{3\sqrt{15}} \delta J(a, x') - \frac{8\sqrt{\frac{3}{5}}}{5} \delta J(a, \alpha') + \frac{1}{2} \sqrt{\frac{5}{3}} \delta J(a, z) , \\
\delta S(a, z; \alpha', y') &= -\frac{1}{16} \delta U(z) + \frac{149}{800} \delta U(\alpha') + \frac{17}{40} \delta J(x', \alpha') + \frac{1}{2} \delta U(x', y')
\end{aligned}$$

$$\begin{aligned}
& + \frac{1}{8}\delta U(x', z) - \frac{17}{200}\delta U(a, \alpha') - \frac{41}{80}\delta U(x', \alpha') + \frac{1}{8}\delta U(a, \gamma) \\
& + \frac{9}{40}\delta U(z, \alpha') + \frac{77}{60}\delta J(a, x') - \frac{117}{100}\delta J(a, \alpha') + \frac{1}{4}\delta J(a, z) , \\
\delta S(a, z; \beta', x') &= -\frac{3}{16}\delta U(z) + \frac{87}{160}\delta U(\alpha') + \frac{3}{8}\delta J(x', \alpha') + \frac{5}{4}\delta U(x', y') \\
& - \frac{1}{8}\delta U(x', z) - \frac{3}{8}\delta U(a, \alpha') - \frac{15}{16}\delta U(x', \alpha') + \frac{2}{5}\delta U(a, \beta') \\
& - \frac{1}{40}\delta U(a, \gamma) - \frac{1}{4}\delta U(x', \beta') + \frac{3}{8}\delta U(z, \alpha') - \frac{3}{20}\delta U(\alpha', \beta') \\
& + \frac{9}{4}\delta J(a, x') - \frac{51}{20}\delta J(a, \alpha') + \frac{3}{4}\delta J(a, z) , \\
\delta S(a, \alpha'; \gamma, y') &= -\frac{\sqrt{\frac{5}{3}}}{8}\delta U(z) + \frac{53}{40\sqrt{15}}\delta U(\alpha') - \frac{1}{2\sqrt{15}}\delta J(x', \alpha') + \frac{1}{3}\sqrt{\frac{5}{3}}\delta U(x', y') \\
& - \frac{23}{20\sqrt{15}}\delta U(a, \alpha') - \sqrt{\frac{3}{5}}\delta U(x', \alpha') + \frac{\sqrt{\frac{5}{3}}}{12}\delta U(a, \gamma) + 2\sqrt{\frac{3}{5}}\delta U(z, \alpha') \\
& + \frac{19}{3\sqrt{15}}\delta J(a, x') - \frac{8\sqrt{\frac{3}{5}}}{5}\delta J(a, \alpha') + \frac{1}{2}\sqrt{\frac{5}{3}}\delta J(a, z) , \\
\delta S(a, \alpha'; \gamma, \beta') &= -\frac{5}{24}\delta U(z) + \frac{29}{60}\delta U(\alpha') - \frac{1}{6}\delta J(x', \alpha') + \frac{5}{12}\delta U(x', y') \\
& - \frac{17}{15}\delta U(a, \alpha') - \frac{7}{12}\delta U(x', \alpha') - \frac{1}{4}\delta U(a, \beta') + \frac{2}{3}\delta U(a, \gamma) \\
& + \frac{1}{2}\delta U(z, \alpha') + \frac{1}{4}\delta U(\alpha', \beta') + \frac{43}{18}\delta J(a, x') - \frac{53}{30}\delta J(a, \alpha') \\
& + \frac{5}{6}\delta J(a, z) , \\
\delta S(a, \beta'; \gamma, x') &= -\frac{\sqrt{\frac{5}{3}}}{8}\delta U(z) + \frac{53}{40\sqrt{15}}\delta U(\alpha') - \frac{1}{2\sqrt{15}}\delta J(x', \alpha') + \frac{1}{3}\sqrt{\frac{5}{3}}\delta U(x', y') \\
& - \frac{4\sqrt{\frac{3}{5}}}{5}\delta U(a, \alpha') - \frac{7}{4\sqrt{15}}\delta U(x', \alpha') + \frac{\sqrt{\frac{5}{3}}}{4}\delta U(a, \beta') + \frac{\sqrt{\frac{5}{3}}}{12}\delta U(a, \gamma) \\
& - \frac{\sqrt{\frac{5}{3}}}{4}\delta U(x', \beta') + 2\sqrt{\frac{3}{5}}\delta U(z, \alpha') + \frac{19}{3\sqrt{15}}\delta J(a, x') - \frac{8\sqrt{\frac{3}{5}}}{5}\delta J(a, \alpha') \\
& + \frac{1}{2}\sqrt{\frac{5}{3}}\delta J(a, z) , \\
\delta S(a, \beta'; \gamma, \alpha') &= \frac{5}{24}\delta U(z) - \frac{29}{60}\delta U(\alpha') + \frac{1}{6}\delta J(x', \alpha') - \frac{5}{12}\delta U(x', y') \\
& + \frac{17}{15}\delta U(a, \alpha') + \frac{7}{12}\delta U(x', \alpha') + \frac{1}{4}\delta U(a, \beta') - \frac{2}{3}\delta U(a, \gamma) \\
& - \frac{1}{2}\delta U(z, \alpha') - \frac{1}{4}\delta U(\alpha', \beta') - \frac{43}{18}\delta J(a, x') + \frac{53}{30}\delta J(a, \alpha') \\
& - \frac{5}{6}\delta J(a, z) , \\
\delta S(x', y'; \alpha', \beta') &= \frac{1}{12}\delta U(z) - \frac{29}{150}\delta U(\alpha') + \frac{1}{15}\delta J(x', \alpha') + \frac{1}{3}\delta U(x', y') \\
& + \frac{34}{75}\delta U(a, \alpha') + \frac{7}{30}\delta U(x', \alpha') + \frac{1}{10}\delta U(a, \beta') + \frac{7}{30}\delta U(a, \gamma) \\
& - \frac{2}{10}\delta U(z, \alpha') - \frac{1}{10}\delta U(\alpha', \beta') - \frac{13}{45}\delta J(a, x') + \frac{53}{75}\delta J(a, \alpha') \\
& - \frac{1}{3}\delta J(a, z) ,
\end{aligned}$$

$$\begin{aligned}
\delta S(x', y'; \beta', \alpha') &= -\frac{1}{12}\delta U(z) + \frac{29}{150}\delta U(\alpha') - \frac{1}{15}\delta J(x', \alpha') - \frac{1}{3}\delta U(x', y') \\
&\quad - \frac{34}{75}\delta U(a, \alpha') - \frac{7}{30}\delta U(x', \alpha') - \frac{1}{10}\delta U(a, \beta') - \frac{7}{30}\delta U(a, \gamma) \\
&\quad + \frac{2}{10}\delta U(z, \alpha') + \frac{1}{10}\delta U(\alpha', \beta') + \frac{13}{45}\delta J(a, x') - \frac{53}{75}\delta J(a, \alpha') \\
&\quad + \frac{1}{3}\delta J(a, z) , \\
\delta S(x', z; \alpha', \gamma) &= \frac{1}{16}\delta U(z) - \frac{149}{800}\delta U(\alpha') - \frac{17}{40}\delta J(x', \alpha') - \frac{1}{2}\delta U(x', y') \\
&\quad - \frac{1}{8}\delta U(x', z) + \frac{17}{200}\delta U(a, \alpha') + \frac{41}{80}\delta U(x', \alpha') - \frac{1}{8}\delta U(a, \gamma) \\
&\quad - \frac{9}{40}\delta U(z, \alpha') - \frac{77}{60}\delta J(a, x') + \frac{117}{100}\delta J(a, \alpha') - \frac{1}{4}\delta J(a, z) , \\
\delta S(x', z; \gamma, \alpha') &= -\frac{1}{6}\delta U(z) + \frac{727}{2400}\delta U(\alpha') + \frac{11}{120}\delta J(x', \alpha') + \frac{1}{2}\delta U(x', y') \\
&\quad + \frac{1}{8}\delta U(x', z) - \frac{91}{600}\delta U(a, \alpha') - \frac{163}{240}\delta U(x', \alpha') + \frac{1}{8}\delta U(a, \gamma) \\
&\quad + \frac{9}{40}\delta U(z, \alpha') + \frac{191}{180}\delta J(a, x') - \frac{391}{300}\delta J(a, \alpha') + \frac{2}{3}\delta J(a, z) , \\
\delta S(x', \alpha'; \gamma, z) &= -\frac{5}{96}\delta U(z) + \frac{7}{120}\delta U(\alpha') - \frac{1}{6}\delta J(x', \alpha') - \frac{1}{30}\delta U(a, \alpha') \\
&\quad - \frac{1}{12}\delta U(x', \alpha') - \frac{2}{18}\delta J(a, x') - \frac{1}{15}\delta J(a, \alpha') + \frac{5}{24}\delta J(a, z) , \\
\delta S(y', z; \beta', \gamma) &= -\frac{3}{16}\delta U(z) + \frac{87}{160}\delta U(\alpha') + \frac{3}{8}\delta J(x', \alpha') + \frac{5}{4}\delta U(x', y') \\
&\quad - \frac{1}{8}\delta U(x', z) - \frac{3}{8}\delta U(a, \alpha') - \frac{15}{16}\delta U(x', \alpha') + \frac{2}{5}\delta U(a, \beta') \\
&\quad - \frac{1}{40}\delta U(a, \gamma) - \frac{1}{4}\delta U(x', \beta') + \frac{3}{8}\delta U(z, \alpha') - \frac{3}{20}\delta U(\alpha', \beta') \\
&\quad + \frac{9}{4}\delta J(a, x') - \frac{51}{20}\delta J(a, \alpha') + \frac{3}{4}\delta J(a, z) , \\
\delta S(y', z; \gamma, \beta') &= -\frac{1}{12}\delta U(z) + \frac{143}{2400}\delta U(\alpha') - \frac{7}{40}\delta J(x', \alpha') - \frac{1}{12}\delta U(x', y') \\
&\quad + \frac{1}{8}\delta U(x', z) - \frac{199}{600}\delta U(a, \alpha') + \frac{11}{80}\delta U(x', \alpha') + \frac{2}{10}\delta U(a, \beta') \\
&\quad + \frac{11}{120}\delta U(a, \gamma) - \frac{1}{4}\delta U(x', \beta') + \frac{1}{40}\delta U(z, \alpha') + \frac{1}{20}\delta U(\alpha', \beta') \\
&\quad - \frac{7}{60}\delta J(a, x') - \frac{19}{300}\delta J(a, \alpha') + \frac{1}{3}\delta J(a, z) , \\
\delta S(y', \beta'; \gamma, z) &= -\frac{13}{96}\delta U(z) + \frac{181}{600}\delta U(\alpha') + \frac{1}{10}\delta J(x', \alpha') + \frac{7}{12}\delta U(x', y') \\
&\quad - \frac{53}{150}\delta U(a, \alpha') - \frac{2}{5}\delta U(x', \alpha') + \frac{3}{10}\delta U(a, \beta') + \frac{1}{30}\delta U(a, \gamma) \\
&\quad - \frac{1}{4}\delta U(x', \beta') + \frac{2}{10}\delta U(z, \alpha') - \frac{1}{20}\delta U(\alpha', \beta') + \frac{16}{15}\delta J(a, x') \\
&\quad - \frac{98}{75}\delta J(a, \alpha') + \frac{13}{24}\delta J(a, z) .
\end{aligned}$$
